# Supplementary material for: Towards Robust Probabilistic Modeling on SO(3) via Rotation Laplace Distribution
Source: arXiv:2305.10465 source file (2025-02-21)
Supplement: Supplementary file 1 [file additional_results.tex]

\section{Additional Results}

\subsection{Additional Numerical Results}
\label{sec:supp_results}

Table \ref{tab:supp_modelnet} and \ref{tab:supp_pascal} extend the results on ModelNet10-SO3 dataset and Pascal3D+ dataset in the main paper and show the per-category results.  
Our prediction with rotation Laplace distribution is at or near state-of-the-art on many categories. The numbers for  baselines are quoted from \cite{murphy2021implicit}.

\begin{table*}[ht]
\centering
% \scriptsize
\fontsize{7.5}{10}\selectfont
\caption{Per-category results ModelNet10-SO3 dataset.}
\resizebox{0.99\textwidth}{!}{
\begin{tabular}{@{}ll@{\hskip 0.3in}c@{\hskip 16pt}cccccccccc}
\toprule
       &                                      & {avg.}     & {bathtub}  & {bed}      & {chair}    & {desk}     & {dresser}  & {tv}       & {n. stand} & {sofa}     & {table}    & {toilet}   \\
\midrule
\multirow{4}{*}{Acc@15\textdegree$\uparrow$}                   & Deng \textit{et al.}\cite{deng2022deep}            & 0.562      & 0.140      & 0.788      & 0.800      & 0.345      & 0.563      & 0.708      & 0.279      & 0.733      & 0.440      & 0.832      \\      
       & Prokudin \textit{et al.}\cite{prokudin2018deep}        & 0.456      & 0.114      & 0.822      & 0.662      & 0.023      & 0.406      & 0.704      & 0.187      & 0.590      & 0.108      &  0.946 \\
       & Mohlin \textit{et al.}\cite{mohlin2020probabilistic} &  0.693 &  0.322 & \bgl 0.882 & \bgl 0.881 &  0.536 &  0.682 &  0.790 &  0.516 & \bgl 0.919 &  0.446 & \bgl 0.957 \\      
       & Murphy \textit{et al.}\cite{murphy2021implicit}     & \bgl 0.719 & \bgd 0.392 &  0.877 &  0.874 & \bgl 0.615 & \bgl 0.687 & \bgl 0.799 & \bgl 0.567 &  0.914 & \bgd 0.523 & 0.945      \\
       & rotation Laplace               & \bgd 0.741  & \bgl 0.390  & \bgd 0.902  & \bgd 0.909  & \bgd 0.644  & \bgd 0.722  & \bgd 0.815  & \bgd 0.590  & \bgd 0.934  & \bgl 0.521  & \bgd 0.977  \\
\midrule
\multirow{4}{*}{Acc@30\textdegree$\uparrow$}                   & Deng \textit{et al.}\cite{deng2022deep}           & 0.694      & 0.325      & 0.880      & 0.908      & 0.556      & 0.649      & 0.807      & 0.466      & 0.902      & 0.485      & 0.958      \\      
       & Prokudin \textit{et al.}\cite{prokudin2018deep}        & 0.528      & 0.175      & 0.847      & 0.777      & 0.061      & 0.500      & 0.788      & 0.306      & 0.673      & 0.183      & 0.972 \\
       & Mohlin \textit{et al.}\cite{mohlin2020probabilistic} & \bgl 0.757 &  0.403 & \bgl 0.908 & \bgl 0.935 & \bgl 0.674 & \bgl 0.739 & \bgl 0.863 & \bgl 0.614 & \bgl 0.944 & 0.511 & \bgl 0.981 \\      
       & Murphy \textit{et al.}\cite{murphy2021implicit}     & 0.735 & \bgl 0.410 &  0.883 &  0.917 & 0.629 & 0.688 &  0.832 &  0.570 &  0.921 & \bgl 0.531 & 0.967      \\
       & rotation Laplace               & \bgd  0.770  & \bgd 0.430 & \bgd 0.911  & \bgd 0.940 & \bgd 0.698  & \bgd 0.751  & \bgd 0.869 & \bgd 0.625  & \bgd 0.946  & \bgd 0.541  & \bgd 0.986  \\
\midrule
\multirow{4}{*}{\shortstack{Median \\ Error ($^\circ$)$\downarrow$}} & Deng \textit{et al.}\cite{deng2022deep}           & 32.6       & 147.8      & 9.2        & 8.3        & 25.0       & 11.9       & 9.8        & 36.9       & 10.0       & 58.6       & 8.5        \\
       & Prokudin \textit{et al.}\cite{prokudin2018deep}        & 49.3       &  122.8 & \bgl 3.6   & 9.6        & 117.2      & 29.9       & 6.7        & 73.0       & 10.4       & 115.5      &  4.1   \\
       & Mohlin \textit{et al.}\cite{mohlin2020probabilistic} & \bgl 17.1  & \bgl 89.1  &  4.4   & \bgl 5.2   &  13.0  &  6.3   &  5.8   &  13.5  & \bgl 4.0   &  25.8  & \bgl 4.0   \\      
       & Murphy \textit{et al.}\cite{murphy2021implicit}     &  21.5  & 161.0      &  4.4   &  5.5   & \bgl 7.1   & \bgl 5.5   & \bgl 5.7   & \bgl 7.5   &  4.1   & \bgd 9.0   & 4.8        \\
       & rotation Laplace               & \bgd 12.2  & \bgd 85.1  & \bgd 2.3  & \bgd 3.4 & \bgd 5.4 & \bgd 2.7  & \bgd 3.7 & \bgd 4.8  & \bgd 2.1  & \bgl 9.6  & \bgd 2.5  \\
\bottomrule
\end{tabular}
}
\label{tab:supp_modelnet}
\end{table*}

\begin{table*}[ht]
\caption{Per-category results on Pascal3D+ dataset.}
  \centering
  \fontsize{7.5}{10}\selectfont
%   \scriptsize
  \resizebox{0.99\textwidth}{!}{
    \begin{tabular}{@{}ll@{\hskip 0.3in}c@{\hskip 16pt}cccccccccccc}
      &                                      & {avg.}     & {aero}  & {bike}      & {boat}    & {bottle}     & {bus}  & {car}       & {chair} & {table}     & {mbike}    & {sofa} & {train}  & {tv} \\
    \midrule
    \multirow{6}{*}{Acc@30\textdegree  $\uparrow$} 
        & Tulsiani \& Malik \cite{tulsiani2015viewpoints}         & 0.808 & 0.81  & 0.77  &  0.59 & 0.93 &  \bgd {0.98} & 0.89 & 0.80 & 0.62 & \bgl 0.88 & 0.82 & 0.80 & 0.80 \\
        & Mahendran \textit{et al.}\cite{mahendran2018mixed}             & \bgl 0.859 & 0.87 & 0.81 &  \bgd {0.64} &  \bgd {0.96} &  0.97 &  0.95 &  \bgd {0.92} & 0.67 & 0.85 & \bgd 0.97 & \bgl 0.82 & \bgl 0.88 \\
        & Liao \textit{et al.}\cite{liao2019spherical}              & 0.819 & 0.82 & 0.77 & 0.55 & 0.93 & 0.95 & 0.94 & 0.85 & 0.61 & 0.80 &  0.95 &  \bgd {0.83} & 0.82     \\   
        & Prokudin \textit{et al.}\cite{liao2019spherical}               &  0.838 &   0.89 &  0.83 & 0.46 &  \bgd {0.96} & 0.93 & 0.90 & 0.80 & \bgl 0.76 & \bgd 0.90 &  {0.90} & \bgl 0.82 &  \bgd {0.91} \\
        & Mohlin \textit{et al.}\cite{mohlin2020probabilistic}        & 0.825 &  \bgd {0.90} & \bgl 0.85 & 0.57 &  0.94 & 0.95 &  \bgd {0.96} & 0.78 & 0.62 & 0.87 & 0.85 & 0.77 & 0.84 \\
        & Murphy \textit{et al.}\cite{murphy2021implicit}             & 0.837 & 0.81 & \bgl 0.85 & 0.56 & 0.93 & 0.95 & 0.94 &  0.87 &  \bgd {0.78} & 0.85 & 0.88 & 0.78 & 0.86  \\
        & rot. Laplace (Ours)                   & \bgd {0.876} & \bgd {0.90}  & \bgd {0.90}  & \bgl 0.60 & \bgd {0.96} & \bgd {0.98} & \bgd {0.96} & \bgl 0.91  & \bgl 0.76  & \bgl 0.88 & \bgd 0.97 &  0.81 & \bgl 0.88  \\
       
    \midrule
    \multirow{6}{*}{\shortstack{Median\\error ($^\circ$)  $\downarrow$}}
        & Tulsiani \& Malik \cite{tulsiani2015viewpoints} & 13.6 & 13.8 & 17.7 & \bgl 21.3 & 12.9 & 5.8 & 9.1 & 14.8 & 15.2 & 14.7 & 13.7 & 8.7 & 15.4 \\
        & Mahendran \textit{et al.}\cite{mahendran2018mixed} &  10.1 &  \bgd {8.5} &  14.8 &  \bgd {20.5} &  7.0 &  3.1 &  5.1 & \bgl 9.3 &  11.3 & 14.2 & 10.2 & \bgl 5.6 & \bgl 11.7 \\
        & Liao \textit{et al.}\cite{liao2019spherical}            & 13.0 & 13.0 & 16.4 & 29.1 & 10.3 & 4.8 & 6.8 & 11.6 & 12.0 & 17.1 & 12.3 & 8.6 & 14.3       \\
        & Prokudin \textit{et al.}\cite{liao2019spherical} & 12.2 &  9.7 & 15.5 & 45.6 &  \bgd {5.4} & \bgl 2.9 &  \bgd {4.5} & 13.1 & 12.6 &  \bgd {11.8} & \bgl 9.1 &  \bgd {4.3} & 12.0 \\
        & Mohlin \textit{et al.}\cite{mohlin2020probabilistic} & 11.5 & 10.1 & 15.6 & 24.3 & 7.8 & 3.3 & 5.3 & 13.5 & 12.5 &  12.9 & 13.8 & 7.4 & \bgl 11.7\\
        & Murphy \textit{et al.}\cite{murphy2021implicit}                        &  10.3 & 10.8 & \bgl 12.9 & 23.4 & 8.8 & 3.4 & 5.3 &  10.0 &  \bgd {7.3} & 13.6 &  9.5  & 6.4  & 12.3 \\
        & rot. Laplace (Ours)             &  \bgd {9.4}  & \bgl 8.6 & \bgd {11.7} &  21.8 & \bgl 6.9 & \bgd {2.8} & \bgl 4.8 & \bgd {7.9} & \bgl 9.1 & \bgl 12.2 & \bgd {8.1} & 6.9 & \bgd {11.6}    \\
      
      \bottomrule
    \end{tabular}
  }
  \label{tab:supp_pascal}
  \end{table*}

\ree{
\subsection{Additional Visual Results}

We show additional visual results on ModelNet10-SO3 dataset in Figure \ref{fig:vis_modelnet} and on Pascal3D+ dataset in Figure \ref{fig:vis_pascal}. As shown in the figures, our distribution provides rich information about the rotation estimations.

To visualize the predicted distributions, we adopt two popular visualization methods used in \cite{mohlin2020probabilistic} and \cite{murphy2021implicit}. 
The visualization in \cite{mohlin2020probabilistic} is achieved by summing the three marginal distributions over the standard basis of $\mathbb{R}^3$ and displaying them on the sphere with color coding. \cite{murphy2021implicit} introduces a new visualization method based on discretization over $\SO$. It projects a great circle of points on $\SO$ to each point on the 2-sphere, and then uses the color wheel to indicate the location on the great circle. The probability density is shown by the size of the points on the plot. See the corresponding papers for more details.

% \begin{figure}[t]
%     \centering
%     \includegraphics[clip,trim=2cm 2cm 2cm 0cm ,width=0.8\linewidth]{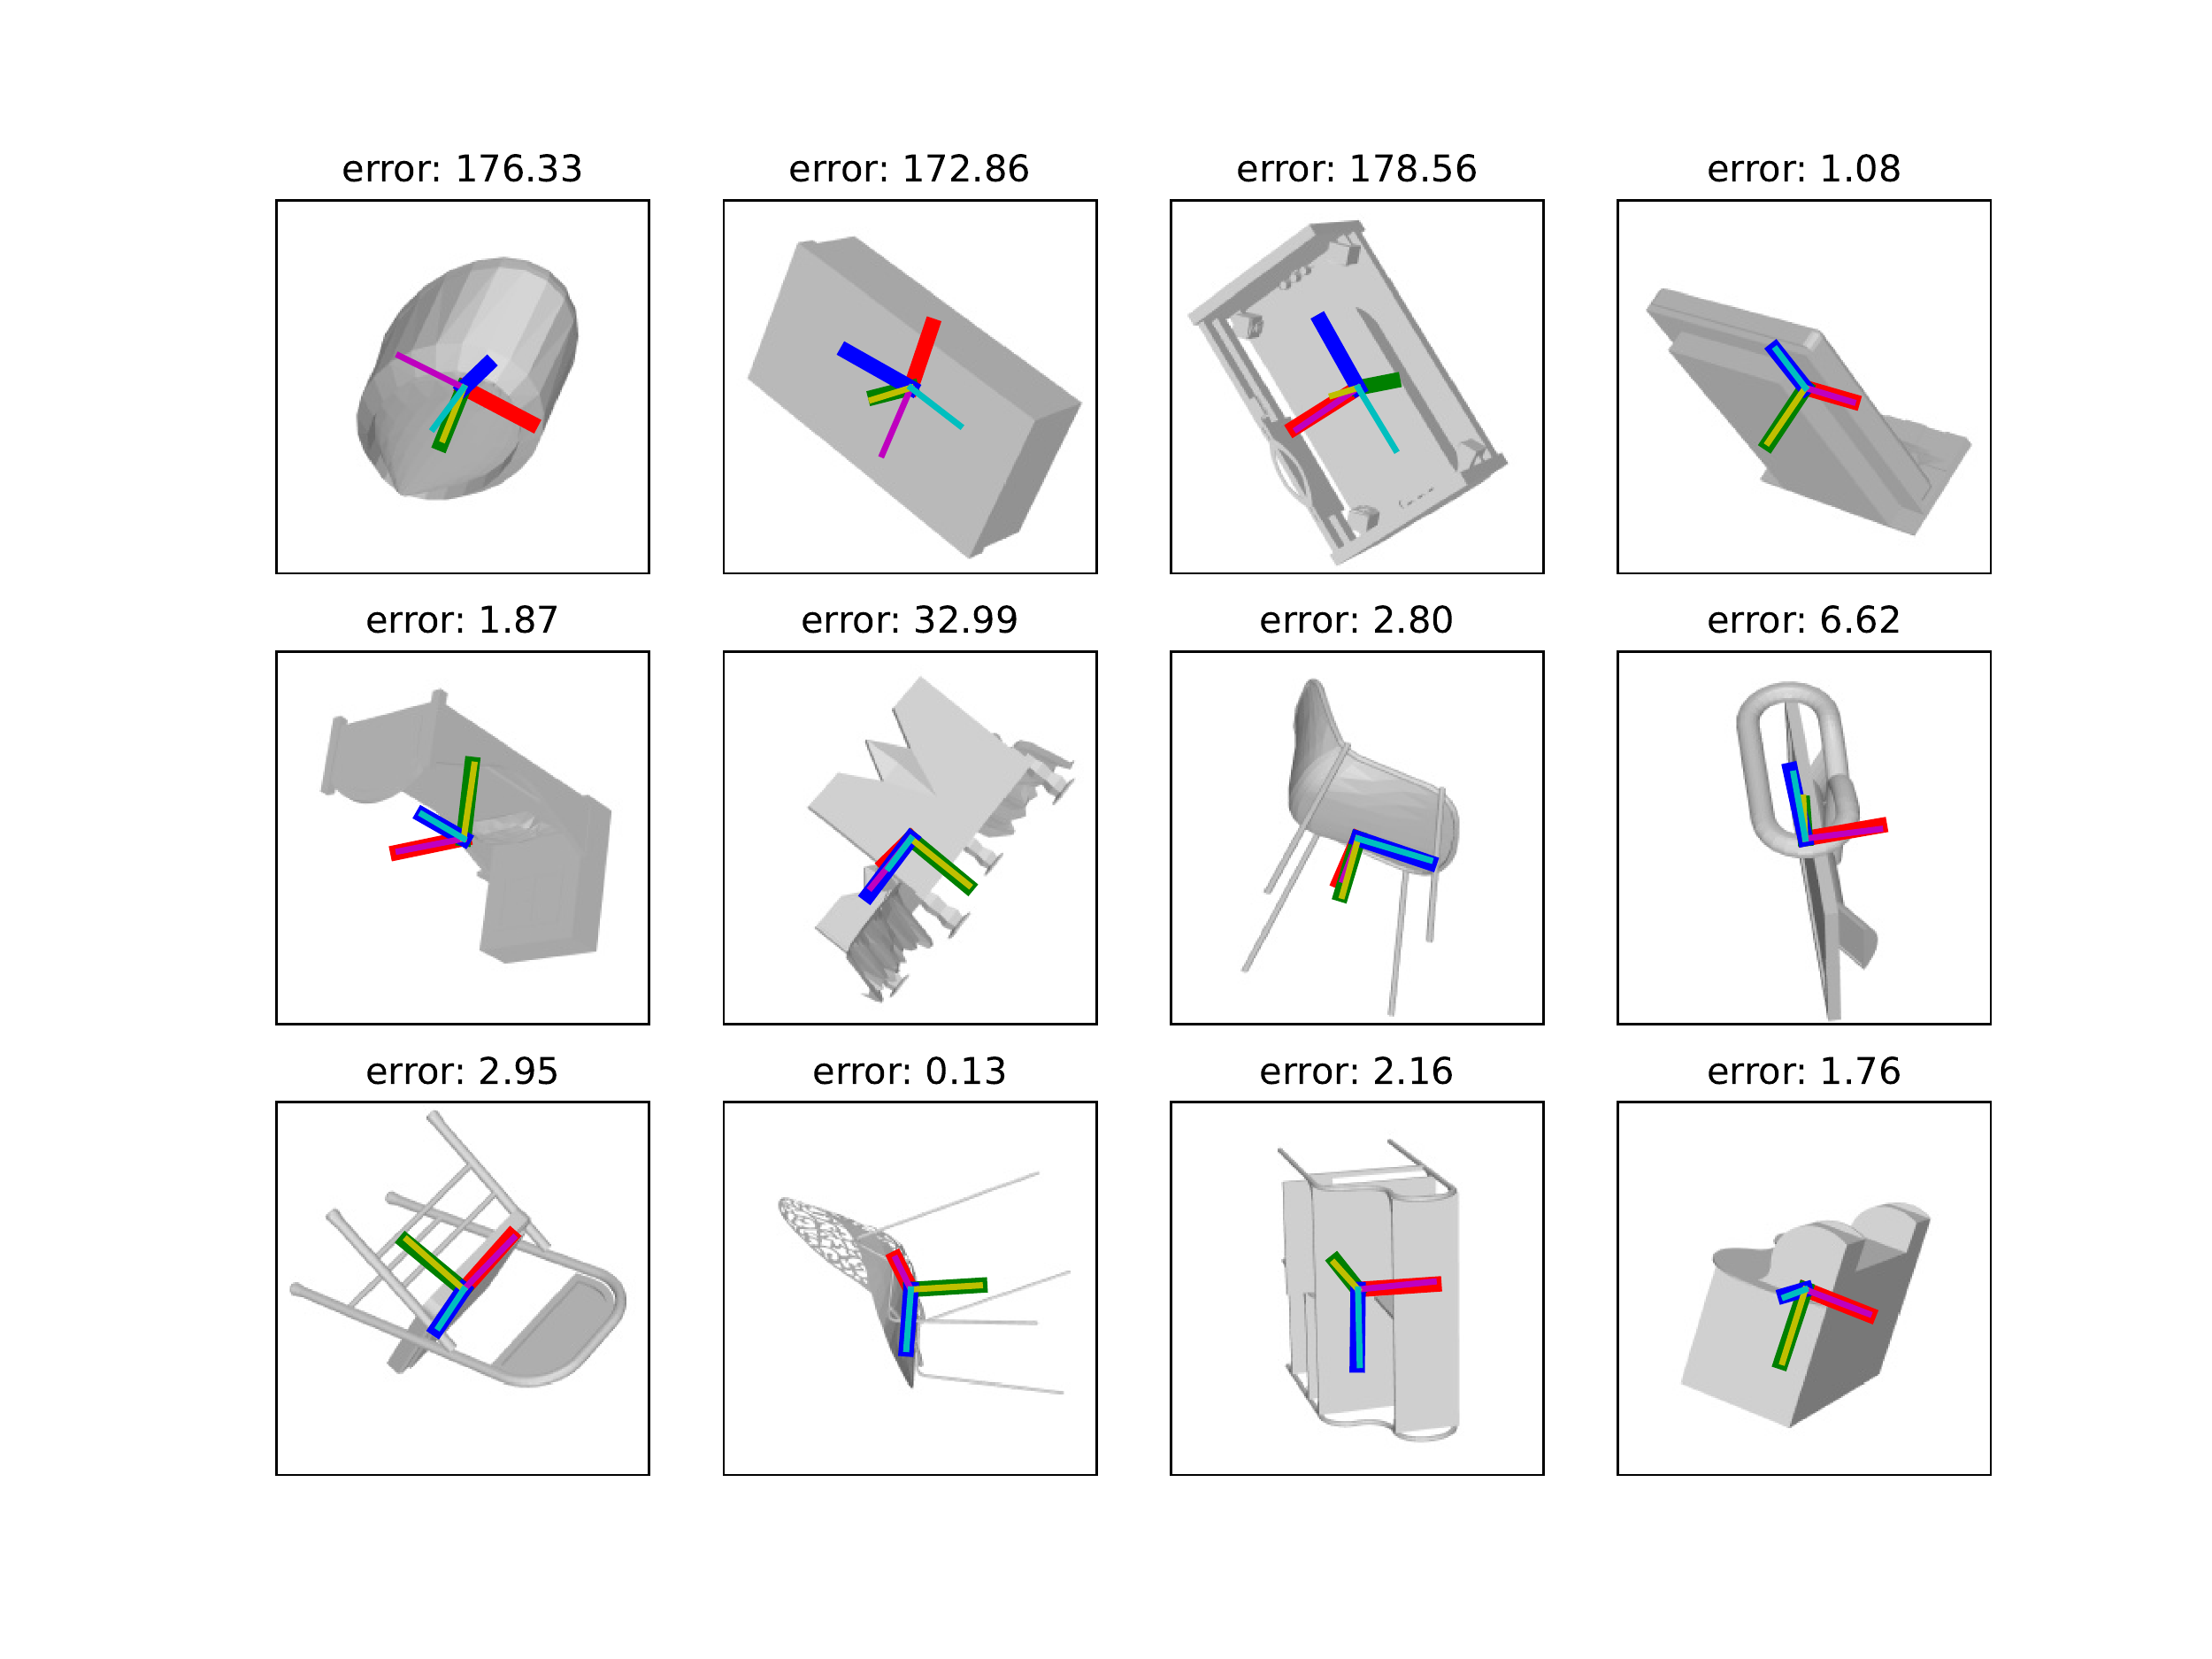}
%     \caption{\ree{Visual results on ModelNet10-SO3 dataset. The axes are projected onto the input images where predicted rotations are shown with thick lines and the ground truths are with thin lines.}}
%     \vspace{-2mm}
% 	\label{fig:vis_modelnet}
% \end{figure}

% \begin{figure}[t]
%     \centering
%     \includegraphics[clip,trim=2cm 2cm 2cm 0cm, width=0.8\linewidth]{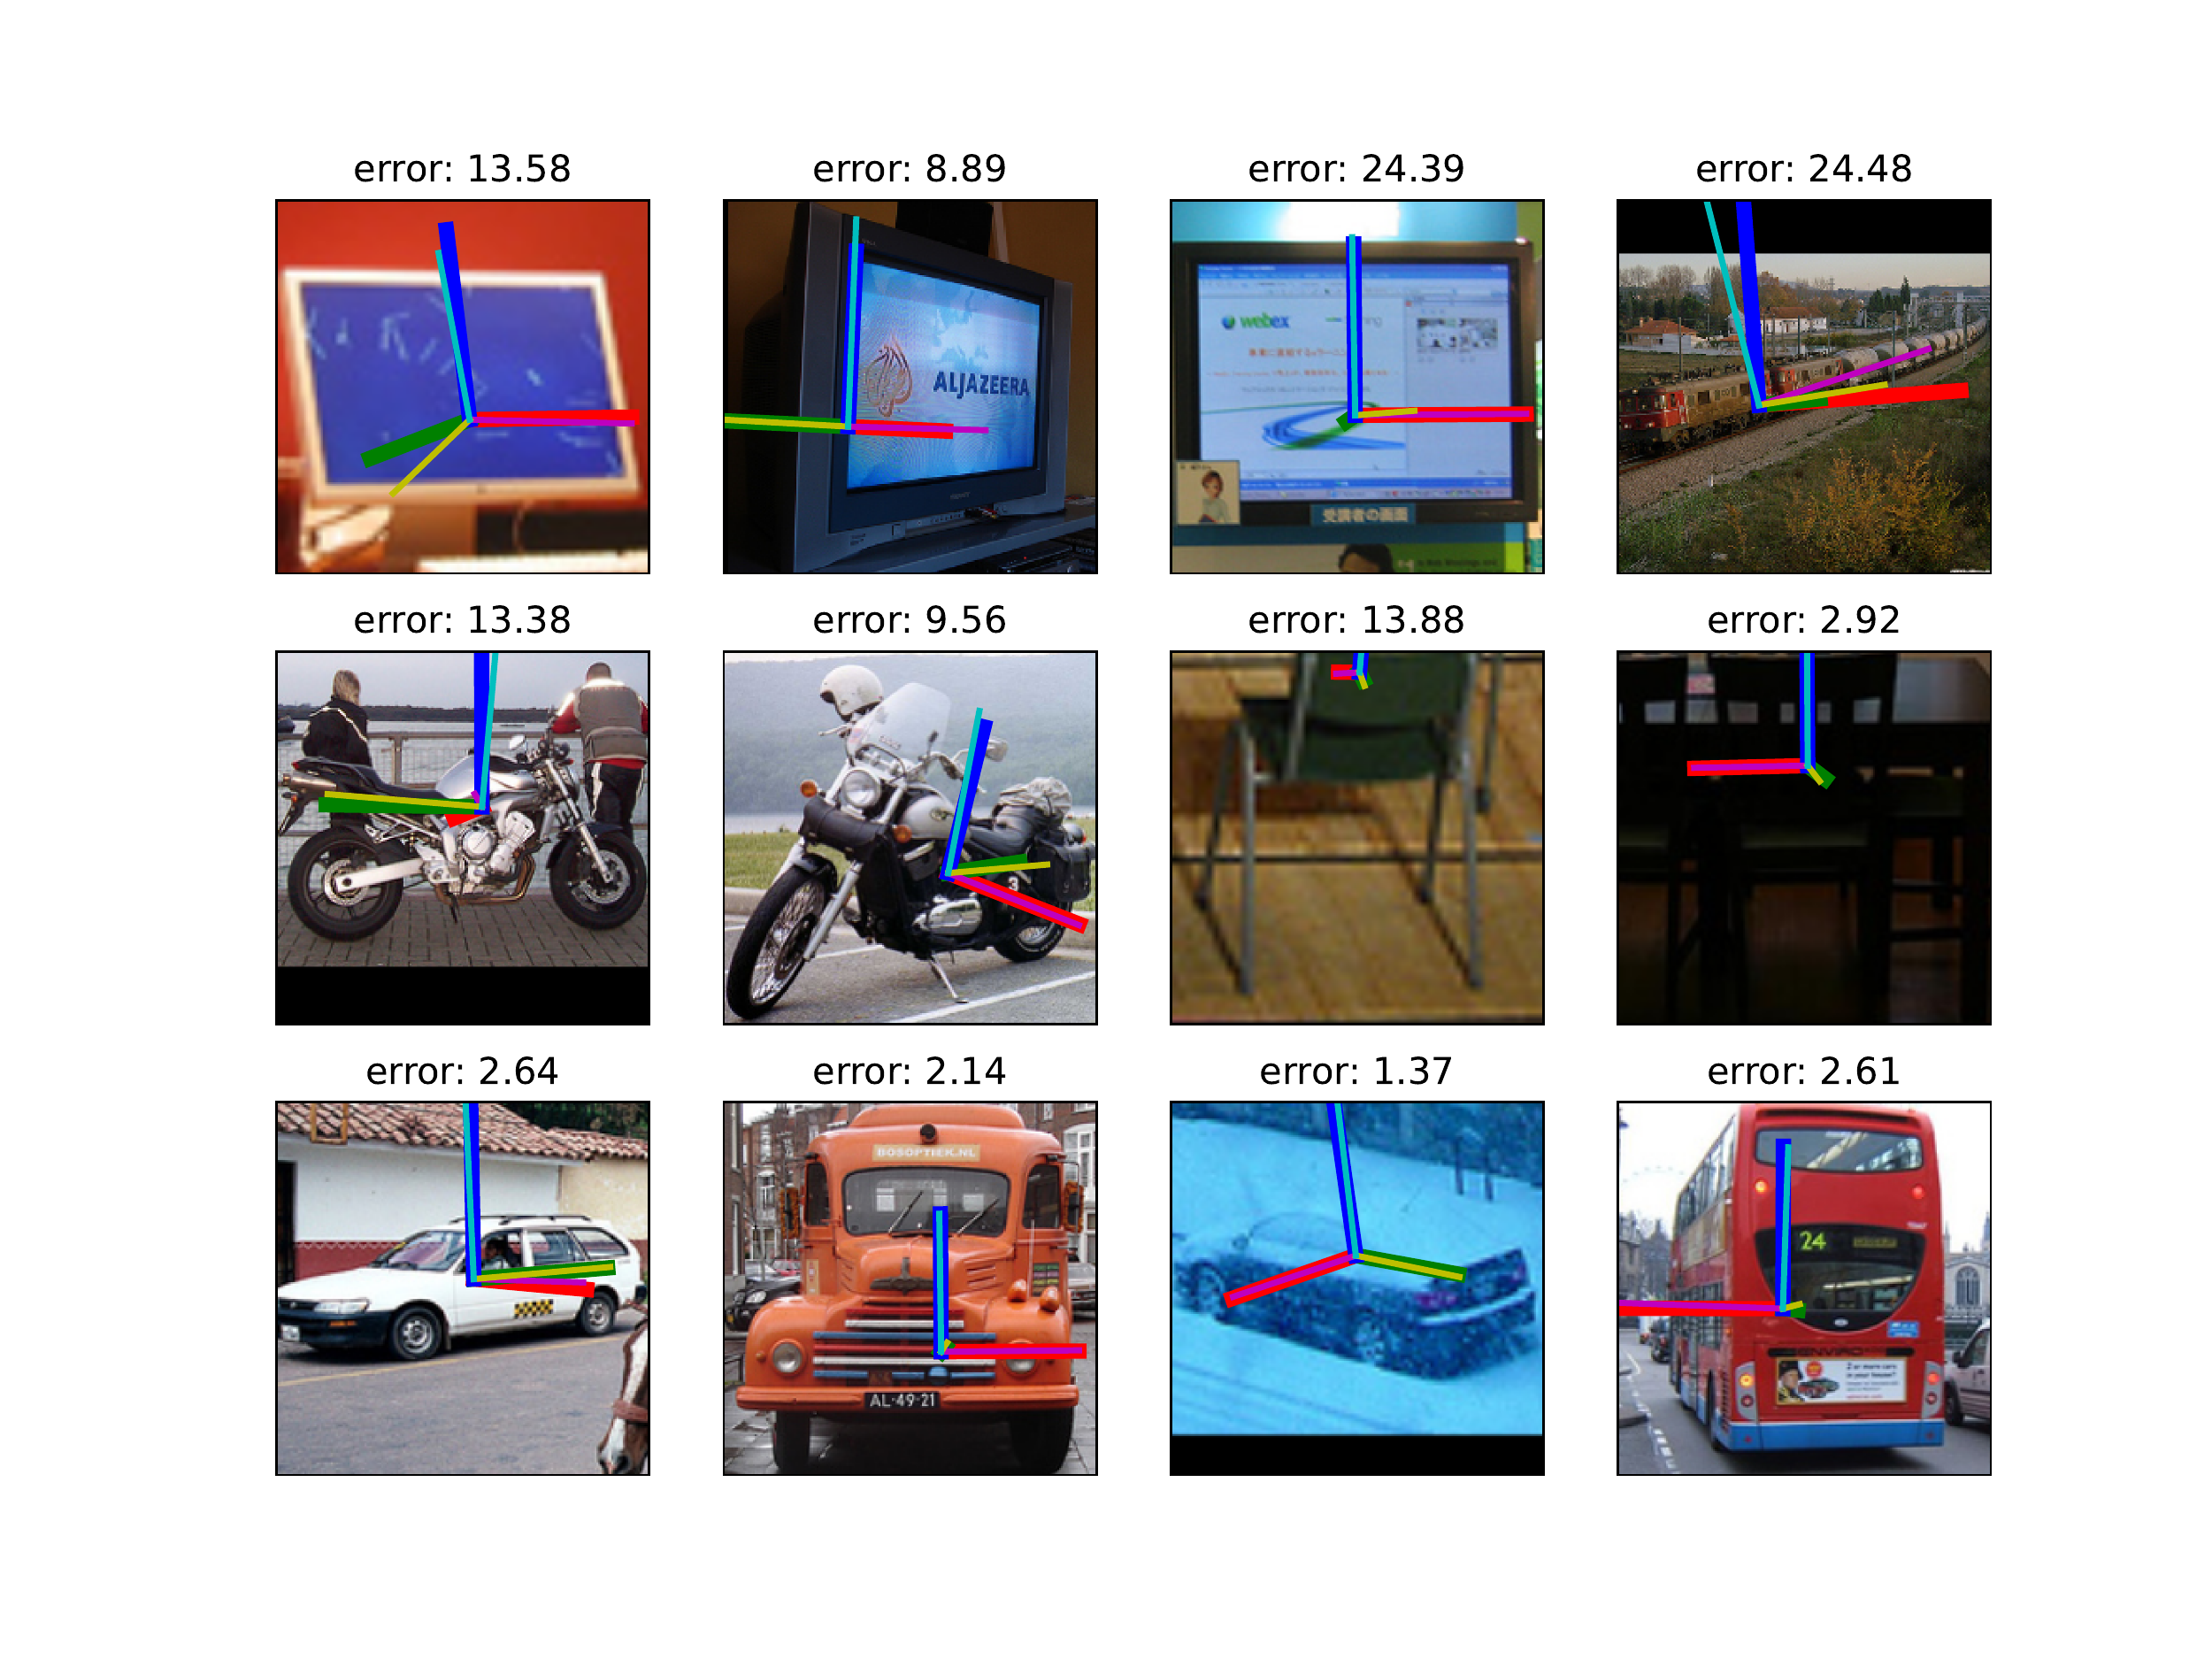}
%     \caption{\ree{Visual results on Pascal3D+ dataset. The axes are projected onto the input images where predicted rotations are shown with thick lines and the ground truths are with thin lines.}}
%     \vspace{-2mm}
% 	\label{fig:vis_pascal}
% \end{figure}

\begin{figure*}[t]
    \centering
    % \vspace{-6mm}
    % \hspace{-3mm}
    \begin{tabular}{cccccc}
    \includegraphics[height=1.6cm]{figures/more_vis/150.jpg}
    &\includegraphics[clip,trim=4.5cm 4cm 4.5cm 1.5cm, height=1.6cm]{figures/more_vis/150_rendering.jpg}
    &\includegraphics[height=1.2cm]{figures/more_vis/150_ipdf.jpg}
    \hspace{4mm}
    &\includegraphics[height=1.6cm]{figures/more_vis/330.jpg}
    &\includegraphics[clip,trim=4.5cm 4cm 4.5cm 1.5cm, height=1.6cm]{figures/more_vis/330_rendering.jpg}
    &\includegraphics[height=1.2cm]{figures/more_vis/330_ipdf.jpg}\\
    
    \includegraphics[height=1.6cm]{figures/more_vis/m450.jpg}
    &\includegraphics[clip,trim=4.5cm 4cm 4.5cm 1.5cm, height=1.6cm]{figures/more_vis/m450_rendering.jpg}
    &\includegraphics[height=1.2cm]{figures/more_vis/m450_ipdf.jpg}
    \hspace{4mm}
    &\includegraphics[height=1.6cm]{figures/more_vis/277.jpg}
    &\includegraphics[clip,trim=4.5cm 4cm 4.5cm 1.5cm, height=1.6cm]{figures/more_vis/277_rendering.jpg}
    &\includegraphics[height=1.2cm]{figures/more_vis/277_ipdf.jpg}\\
    
    \includegraphics[height=1.6cm]{figures/more_vis/1815.jpg}
    &\includegraphics[clip,trim=4.5cm 4cm 4.5cm 1.5cm, height=1.6cm]{figures/more_vis/1815_rendering.jpg}
    &\includegraphics[height=1.2cm]{figures/more_vis/1815_ipdf.jpg}
    \hspace{4mm}
    &\includegraphics[height=1.6cm]{figures/more_vis/1170.jpg}
    &\includegraphics[clip,trim=4.5cm 4cm 4.5cm 1.5cm, height=1.6cm]{figures/more_vis/1170_rendering.jpg}
    &\includegraphics[height=1.2cm]{figures/more_vis/1170_ipdf.jpg}\\
    
    \includegraphics[height=1.6cm]{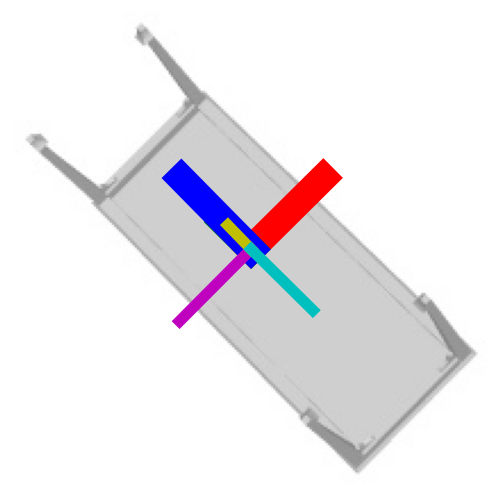}
    &\includegraphics[clip,trim=4.5cm 4cm 4.5cm 1.5cm, height=1.6cm]{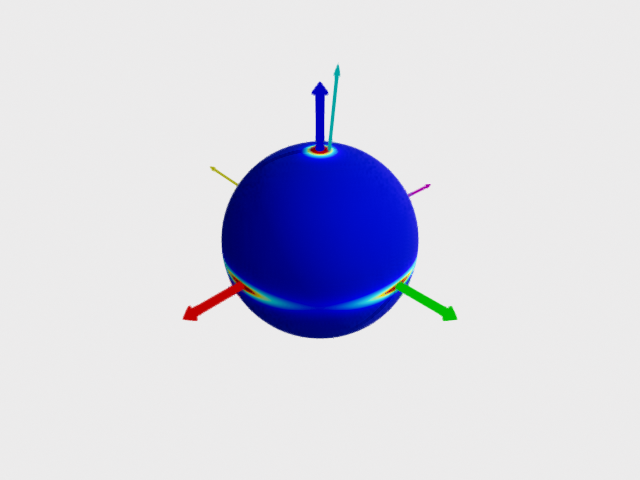}
    &\includegraphics[height=1.2cm]{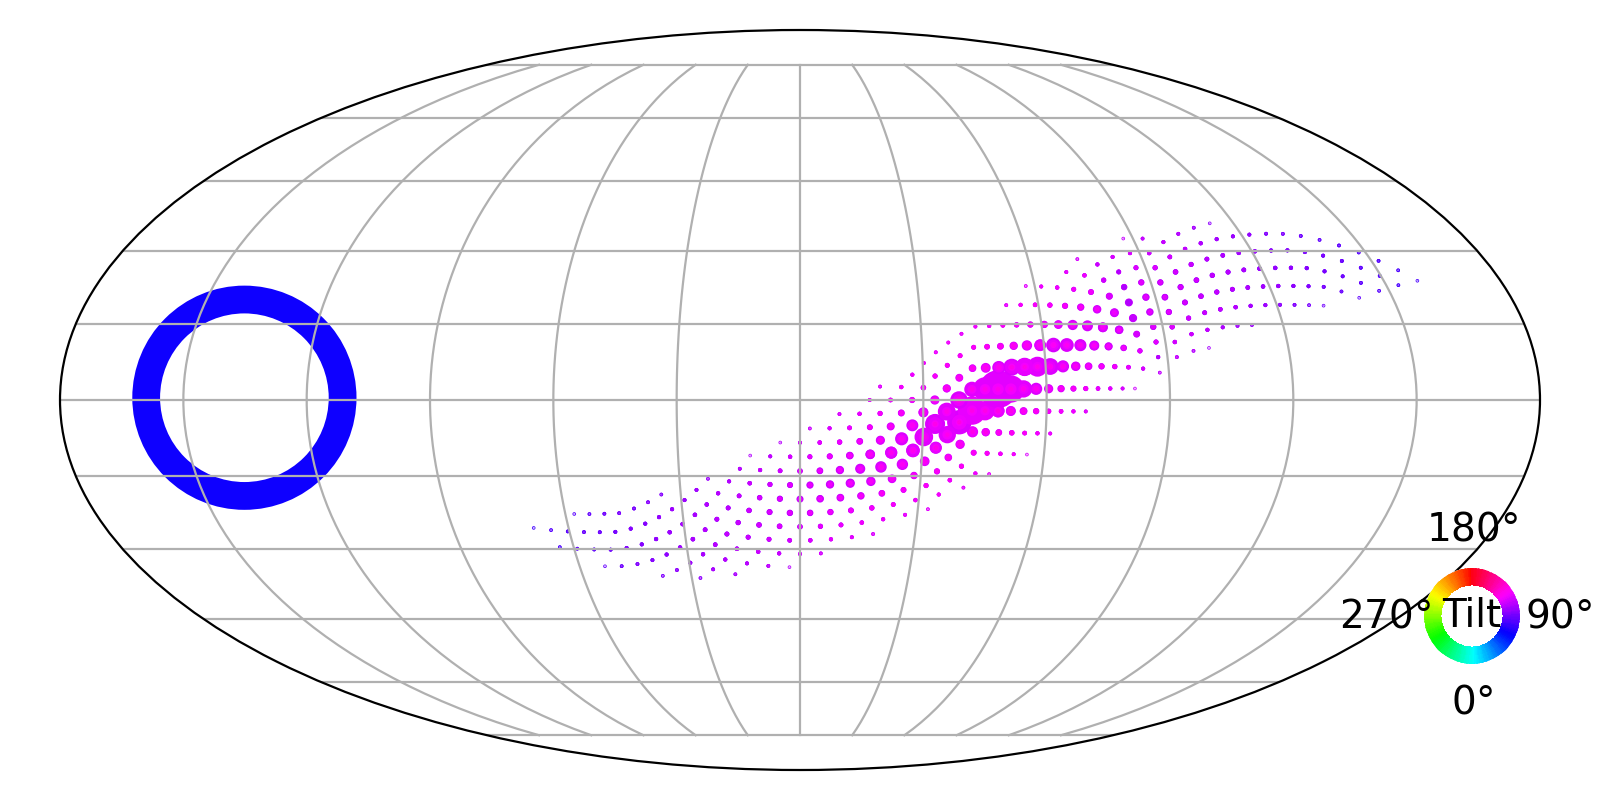}
    \hspace{4mm}
    &\includegraphics[height=1.6cm]{figures/more_vis/93.jpg}
    &\includegraphics[clip,trim=4.5cm 4cm 4.5cm 1.5cm, height=1.6cm]{figures/more_vis/93_rendering.jpg}
    &\includegraphics[height=1.2cm]{figures/more_vis/93_ipdf.jpg}\\
    
    \includegraphics[height=1.6cm]{figures/more_vis/21.jpg}
    &\includegraphics[clip,trim=4.5cm 4cm 4.5cm 1.5cm, height=1.6cm]{figures/more_vis/21_rendering.jpg}
    &\includegraphics[height=1.2cm]{figures/more_vis/21_ipdf.jpg}
    \hspace{4mm}
    &\includegraphics[height=1.6cm]{figures/more_vis/1290.jpg}
    &\includegraphics[clip,trim=4.5cm 4cm 4.5cm 1.5cm, height=1.6cm]{figures/more_vis/1290_rendering.jpg}
    &\includegraphics[height=1.2cm]{figures/more_vis/1290_ipdf.jpg}\\
    
    \includegraphics[height=1.6cm]{figures/more_vis/1255.jpg}
    &\includegraphics[clip,trim=4.5cm 4cm 4.5cm 1.5cm, height=1.6cm]{figures/more_vis/1255_rendering.jpg}
    &\includegraphics[height=1.2cm]{figures/more_vis/1255_ipdf.jpg}
    \hspace{4mm}
    &\includegraphics[height=1.6cm]{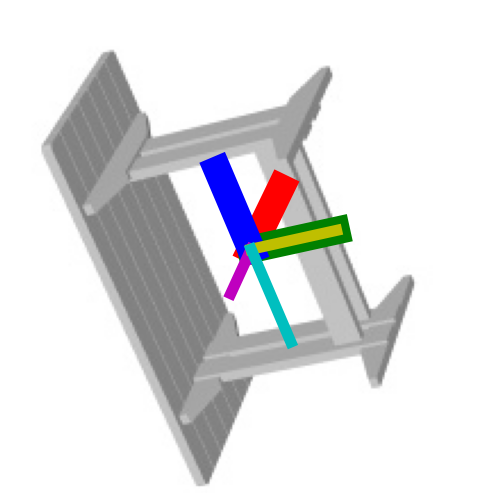}
    &\includegraphics[clip,trim=4.5cm 4cm 4.5cm 1.5cm, height=1.6cm]{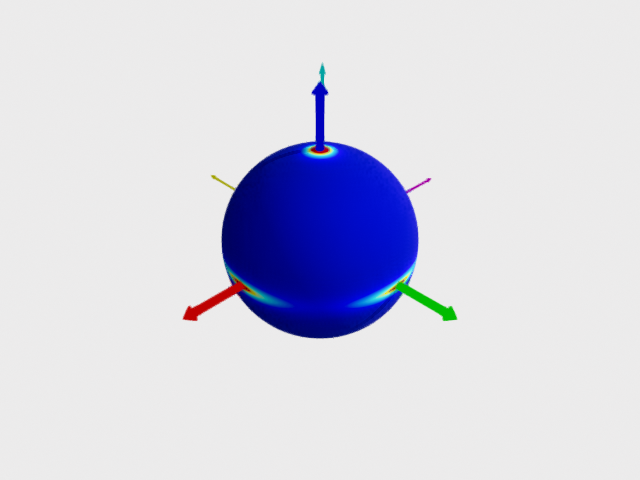}
    &\includegraphics[height=1.2cm]{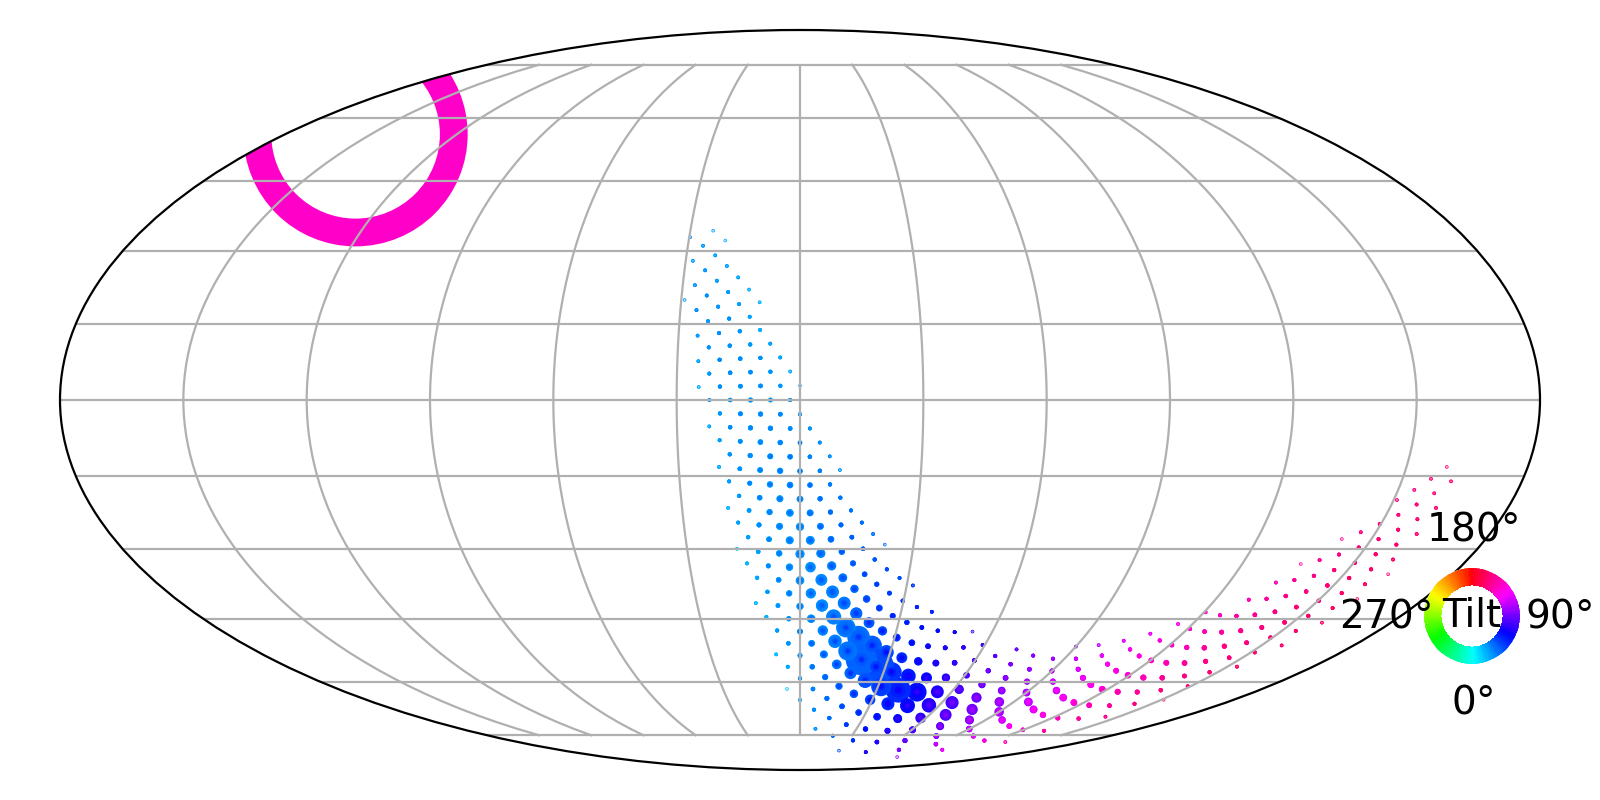}\\
    
    \small{Input image} & {\tiny\makecell{Distribution visual.\\\cite{mohlin2020probabilistic}}} & {\tiny\makecell{Distribution visual.\\\cite{murphy2021implicit}}}  \hspace{4mm} &
    \small{Input image} & {\tiny\makecell{Distribution visual.\\\cite{mohlin2020probabilistic}}} & {\tiny\makecell{Distribution visual.\\\cite{murphy2021implicit}}}
    \end{tabular}
    % \vspace{1mm}
    \caption{\small \ree{Visual results on ModelNet10-SO3 dataset. We adopt the distribution visualization methods in \cite{mohlin2020probabilistic} and \cite{murphy2021implicit}. For input images and visualizations with \cite{mohlin2020probabilistic}, predicted rotations are shown with thick lines and the ground truths are with thin lines. For visualizations with \cite{murphy2021implicit}, ground truths are shown by solid circles.}}
    \vspace{-2mm}
	\label{fig:vis_modelnet}
\end{figure*}
\begin{figure*}[t]
    \centering
    % \vspace{-6mm}
    % \hspace{-3mm}
    \begin{tabular}{cccccc}
    \includegraphics[height=1.6cm]{figures/more_vis/30.jpg}
    &\includegraphics[clip,trim=4.5cm 4cm 4.5cm 1.5cm, height=1.6cm]{figures/more_vis/30_rendering.jpg}
    &\includegraphics[height=1.2cm]{figures/more_vis/30_ipdf.jpg}
    \hspace{4mm}
    &\includegraphics[height=1.6cm]{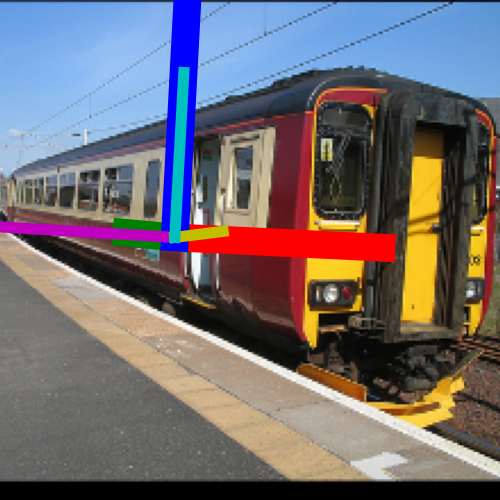}
    &\includegraphics[clip,trim=4.5cm 4cm 4.5cm 1.5cm, height=1.6cm]{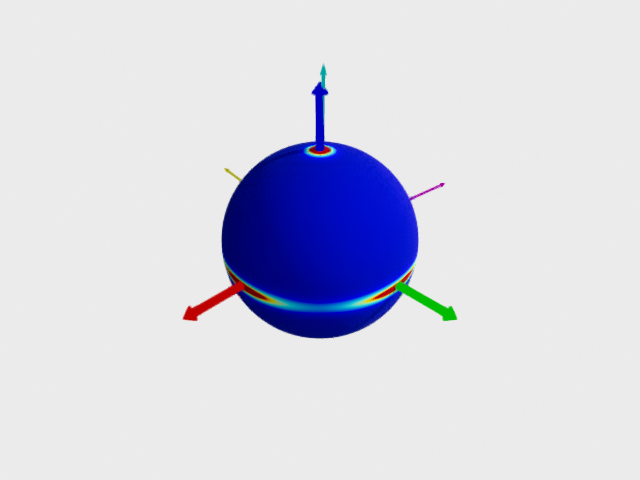}
    &\includegraphics[height=1.2cm]{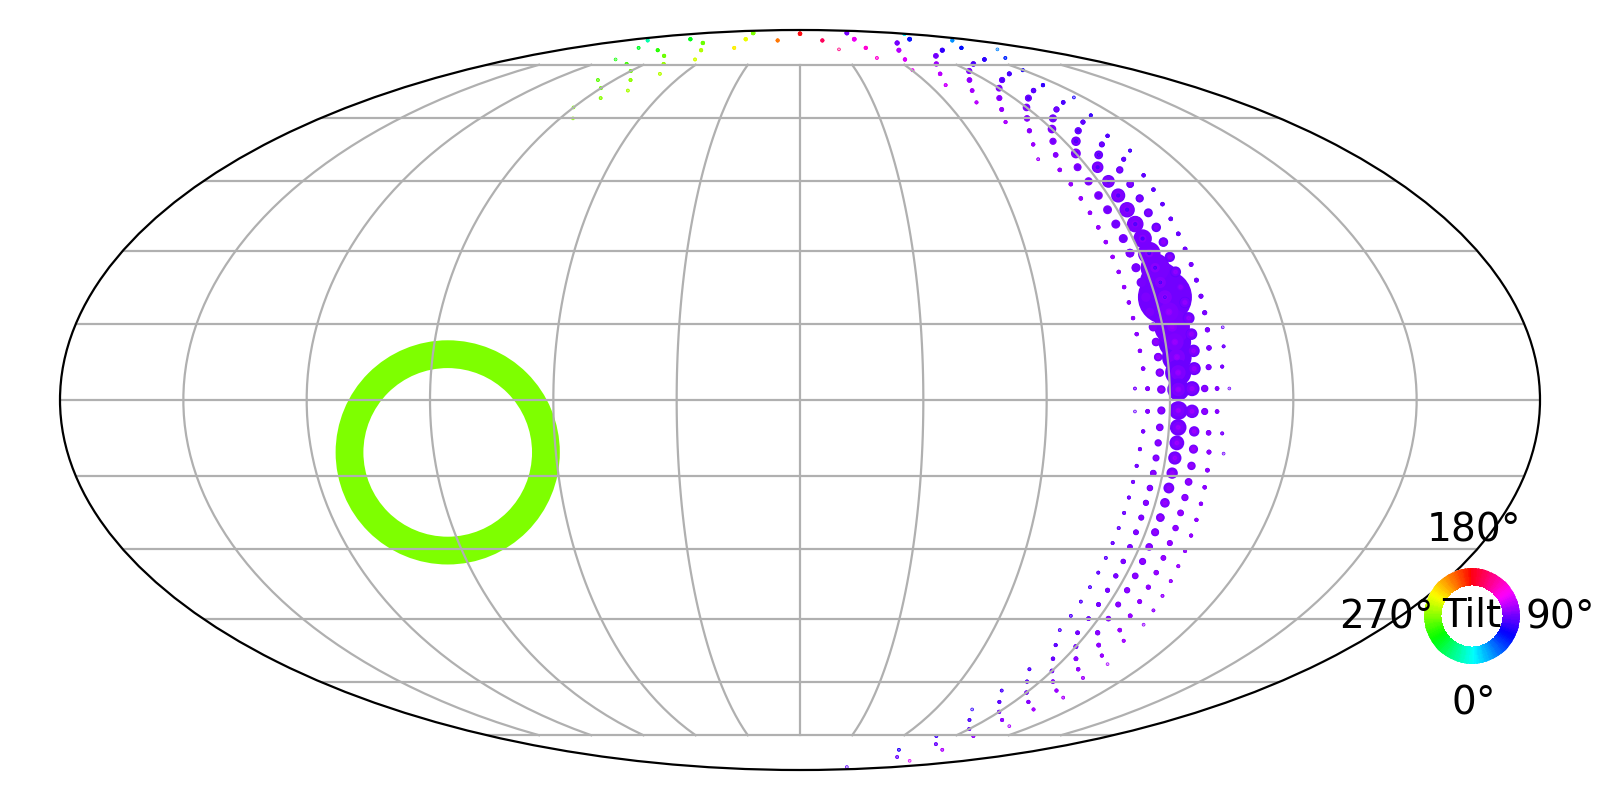}\\
    
    \includegraphics[height=1.6cm]{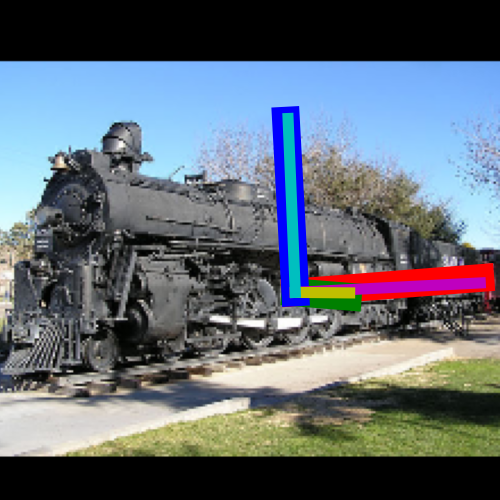}
    &\includegraphics[clip,trim=4.5cm 4cm 4.5cm 1.5cm, height=1.6cm]{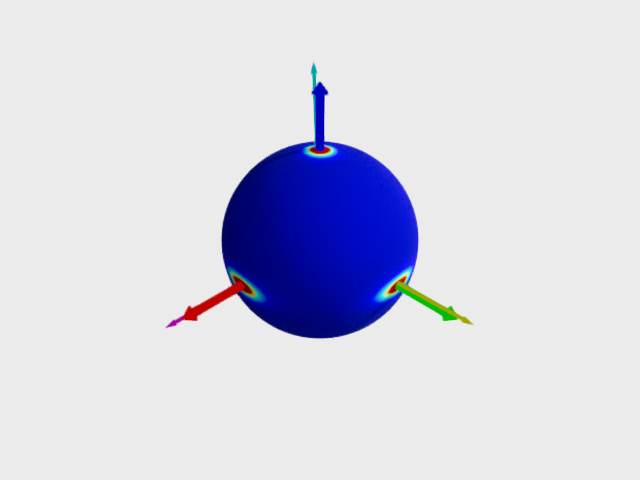}
    &\includegraphics[height=1.2cm]{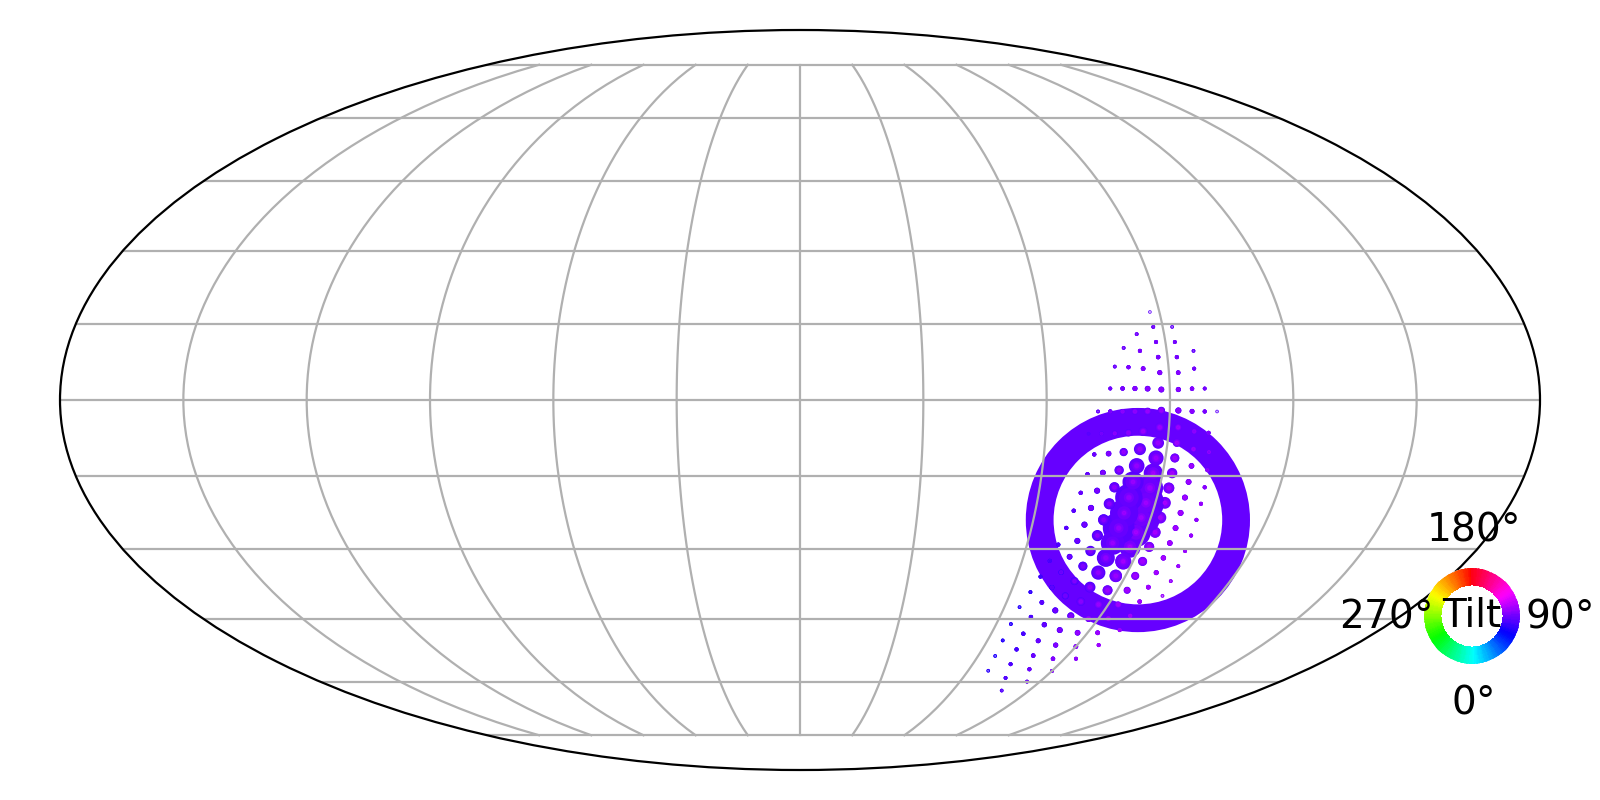}
    \hspace{4mm}
    &\includegraphics[height=1.6cm]{figures/more_vis/450.jpg}
    &\includegraphics[clip,trim=4.5cm 4cm 4.5cm 1.5cm, height=1.6cm]{figures/more_vis/450_rendering.jpg}
    &\includegraphics[height=1.2cm]{figures/more_vis/450_ipdf.jpg}\\
    
    \includegraphics[height=1.6cm]{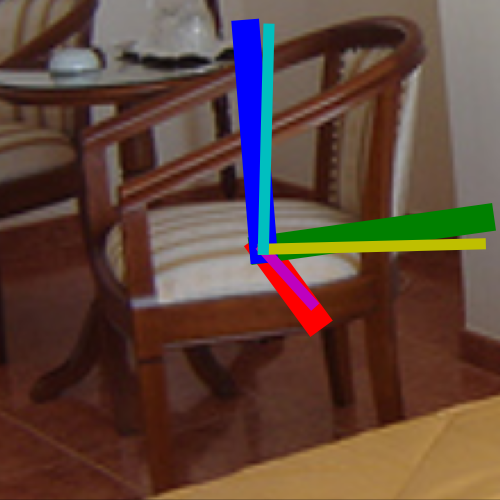}
    &\includegraphics[clip,trim=4.5cm 4cm 4.5cm 1.5cm, height=1.6cm]{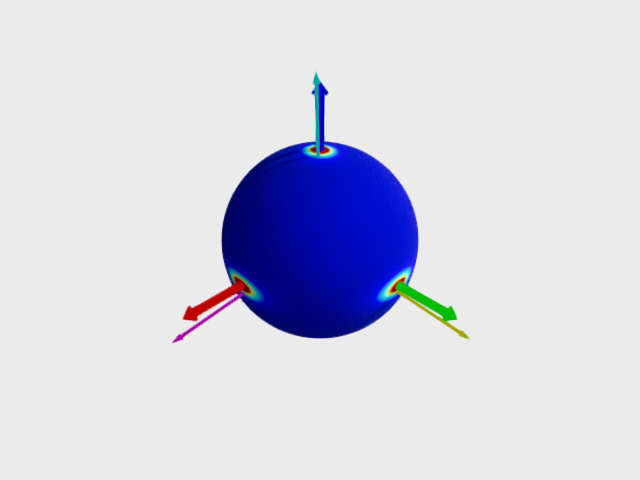}
    &\includegraphics[height=1.2cm]{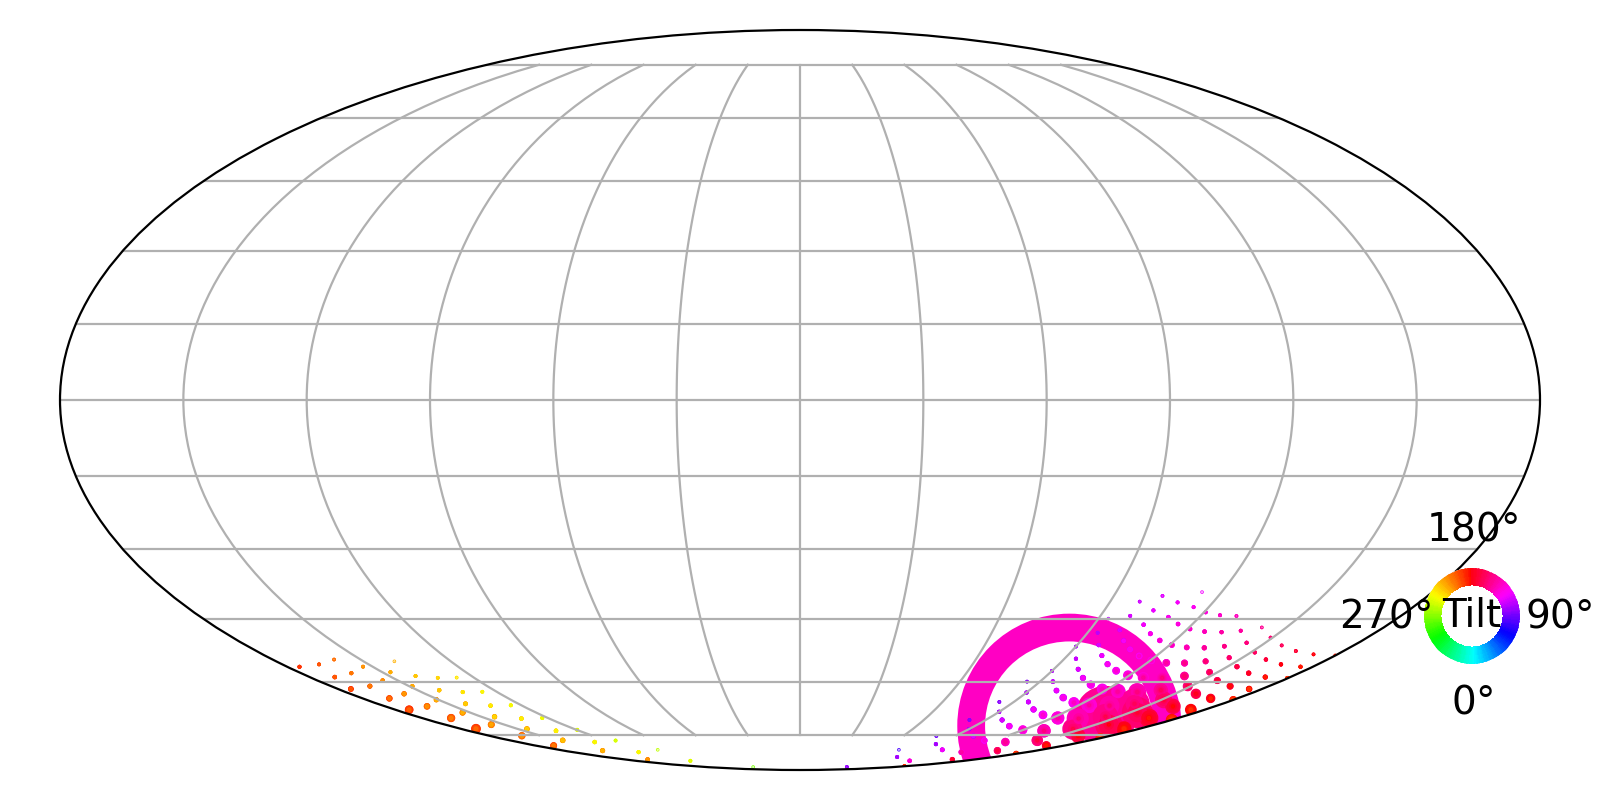}
    \hspace{4mm}
    &\includegraphics[height=1.6cm]{figures/more_vis/540.jpg}
    &\includegraphics[clip,trim=4.5cm 4cm 4.5cm 1.5cm, height=1.6cm]{figures/more_vis/540_rendering.jpg}
    &\includegraphics[height=1.2cm]{figures/more_vis/540_ipdf.jpg}\\
    
    \includegraphics[height=1.6cm]{figures/more_vis/900.jpg}
    &\includegraphics[clip,trim=4.5cm 4cm 4.5cm 1.5cm, height=1.6cm]{figures/more_vis/900_rendering.jpg}
    &\includegraphics[height=1.2cm]{figures/more_vis/900_ipdf.jpg}
    \hspace{4mm}
    &\includegraphics[height=1.6cm]{figures/more_vis/840.jpg}
    &\includegraphics[clip,trim=4.5cm 4cm 4.5cm 1.5cm, height=1.6cm]{figures/more_vis/840_rendering.jpg}
    &\includegraphics[height=1.2cm]{figures/more_vis/840_ipdf.jpg}\\
    
    \includegraphics[height=1.6cm]{figures/more_vis/1070.jpg}
    &\includegraphics[clip,trim=4.5cm 4cm 4.5cm 1.5cm, height=1.6cm]{figures/more_vis/1070_rendering.jpg}
    &\includegraphics[height=1.2cm]{figures/more_vis/1070_ipdf.jpg}
    \hspace{4mm}
    &\includegraphics[height=1.6cm]{figures/more_vis/1380.jpg}
    &\includegraphics[clip,trim=4.5cm 4cm 4.5cm 1.5cm, height=1.6cm]{figures/more_vis/1380_rendering.jpg}
    &\includegraphics[height=1.2cm]{figures/more_vis/1380_ipdf.jpg}\\
    
    \includegraphics[height=1.6cm]{figures/more_vis/1696.jpg}
    &\includegraphics[clip,trim=4.5cm 4cm 4.5cm 1.5cm, height=1.6cm]{figures/more_vis/1696_rendering.jpg}
    &\includegraphics[height=1.2cm]{figures/more_vis/1696_ipdf.jpg}
    \hspace{4mm}
    &\includegraphics[height=1.6cm]{figures/more_vis/1230.jpg}
    &\includegraphics[clip,trim=4.5cm 4cm 4.5cm 1.5cm, height=1.6cm]{figures/more_vis/1230_rendering.jpg}
    &\includegraphics[height=1.2cm]{figures/more_vis/1230_ipdf.jpg}\\
    
    \small{Input image} & {\tiny\makecell{Distribution visual.\\\cite{mohlin2020probabilistic}}} & {\tiny\makecell{Distribution visual.\\\cite{murphy2021implicit}}}  \hspace{4mm} &
    \small{Input image} & {\tiny\makecell{Distribution visual.\\\cite{mohlin2020probabilistic}}} & {\tiny\makecell{Distribution visual.\\\cite{murphy2021implicit}}}
    \end{tabular}
    % \vspace{-3mm}
    \caption{\small \ree{Visual results on Pascal3D+ dataset. We adopt the distribution visualization methods in \cite{mohlin2020probabilistic} and \cite{murphy2021implicit}. For input images and visualizations with \cite{mohlin2020probabilistic}, predicted rotations are shown with thick lines and the ground truths are with thin lines. For visualizations with \cite{murphy2021implicit}, ground truths are shown by solid circles.}}
    \vspace{-2mm}
	\label{fig:vis_pascal}
\end{figure*}

}
