# Supplementary material for: Towards Robust Probabilistic Modeling on SO(3) via Rotation Laplace Distribution
Source: arXiv:2305.10465 source file (2025-02-21)
Supplement: Supplementary file 2 [file exp_wahba.tex]

\subsection{Experiments on the Instance-level Wahba's Problem}

\jiangran{To further investigate the behavior of our distribution in scenarios with few outliers and easy optimization, we conduct a simpler experiment on the instance-level Wahba's problem.}
Unlike the category-level setting in our previous manuscript, which is trained on thousands of airplane point clouds with random rotations (similar to \cite{zhou2019continuity, peretroukhin2020smooth}), this instance-level experiment focuses only on a single instance. Specifically, we choose an airplane point cloud from the ShapeNet dataset and apply random rotations in both the training and evaluation phases. The training process involves 10k iterations using the Adam optimizer, with a batch size of 100, and we experiment with different learning rates. The test errors throughout the learning process are depicted in Fig. \ref{fig:wahba_instance}. We set $\epsilon=1e-8$ for the rotation Laplace distribution.

For this simple task with perfectly annotated ground truth, our rotation Laplace distribution does not exhibit superiority. As shown in Fig. \ref{fig:wahba_instance}, our distribution achieves nearly identical performance to the matrix Fisher distribution and is slightly inferior to 10D \cite{peretroukhin2020smooth} in most cases. 
\jiangran{This simple Wahba's problem reveals that the rotation Laplace distribution is more suitable for scenarios with noticeable outliers.}

\jiangran{Furthermore, the rotation Laplace distribution does not suffer from oscillation in the learning process, which may be attributed to the difficulty of the predicted mode being accurate enough to trigger instability.}

\begin{figure*}[th]
    \centering
    \begin{tabular}{cc}
    \includegraphics[width=0.35\linewidth]{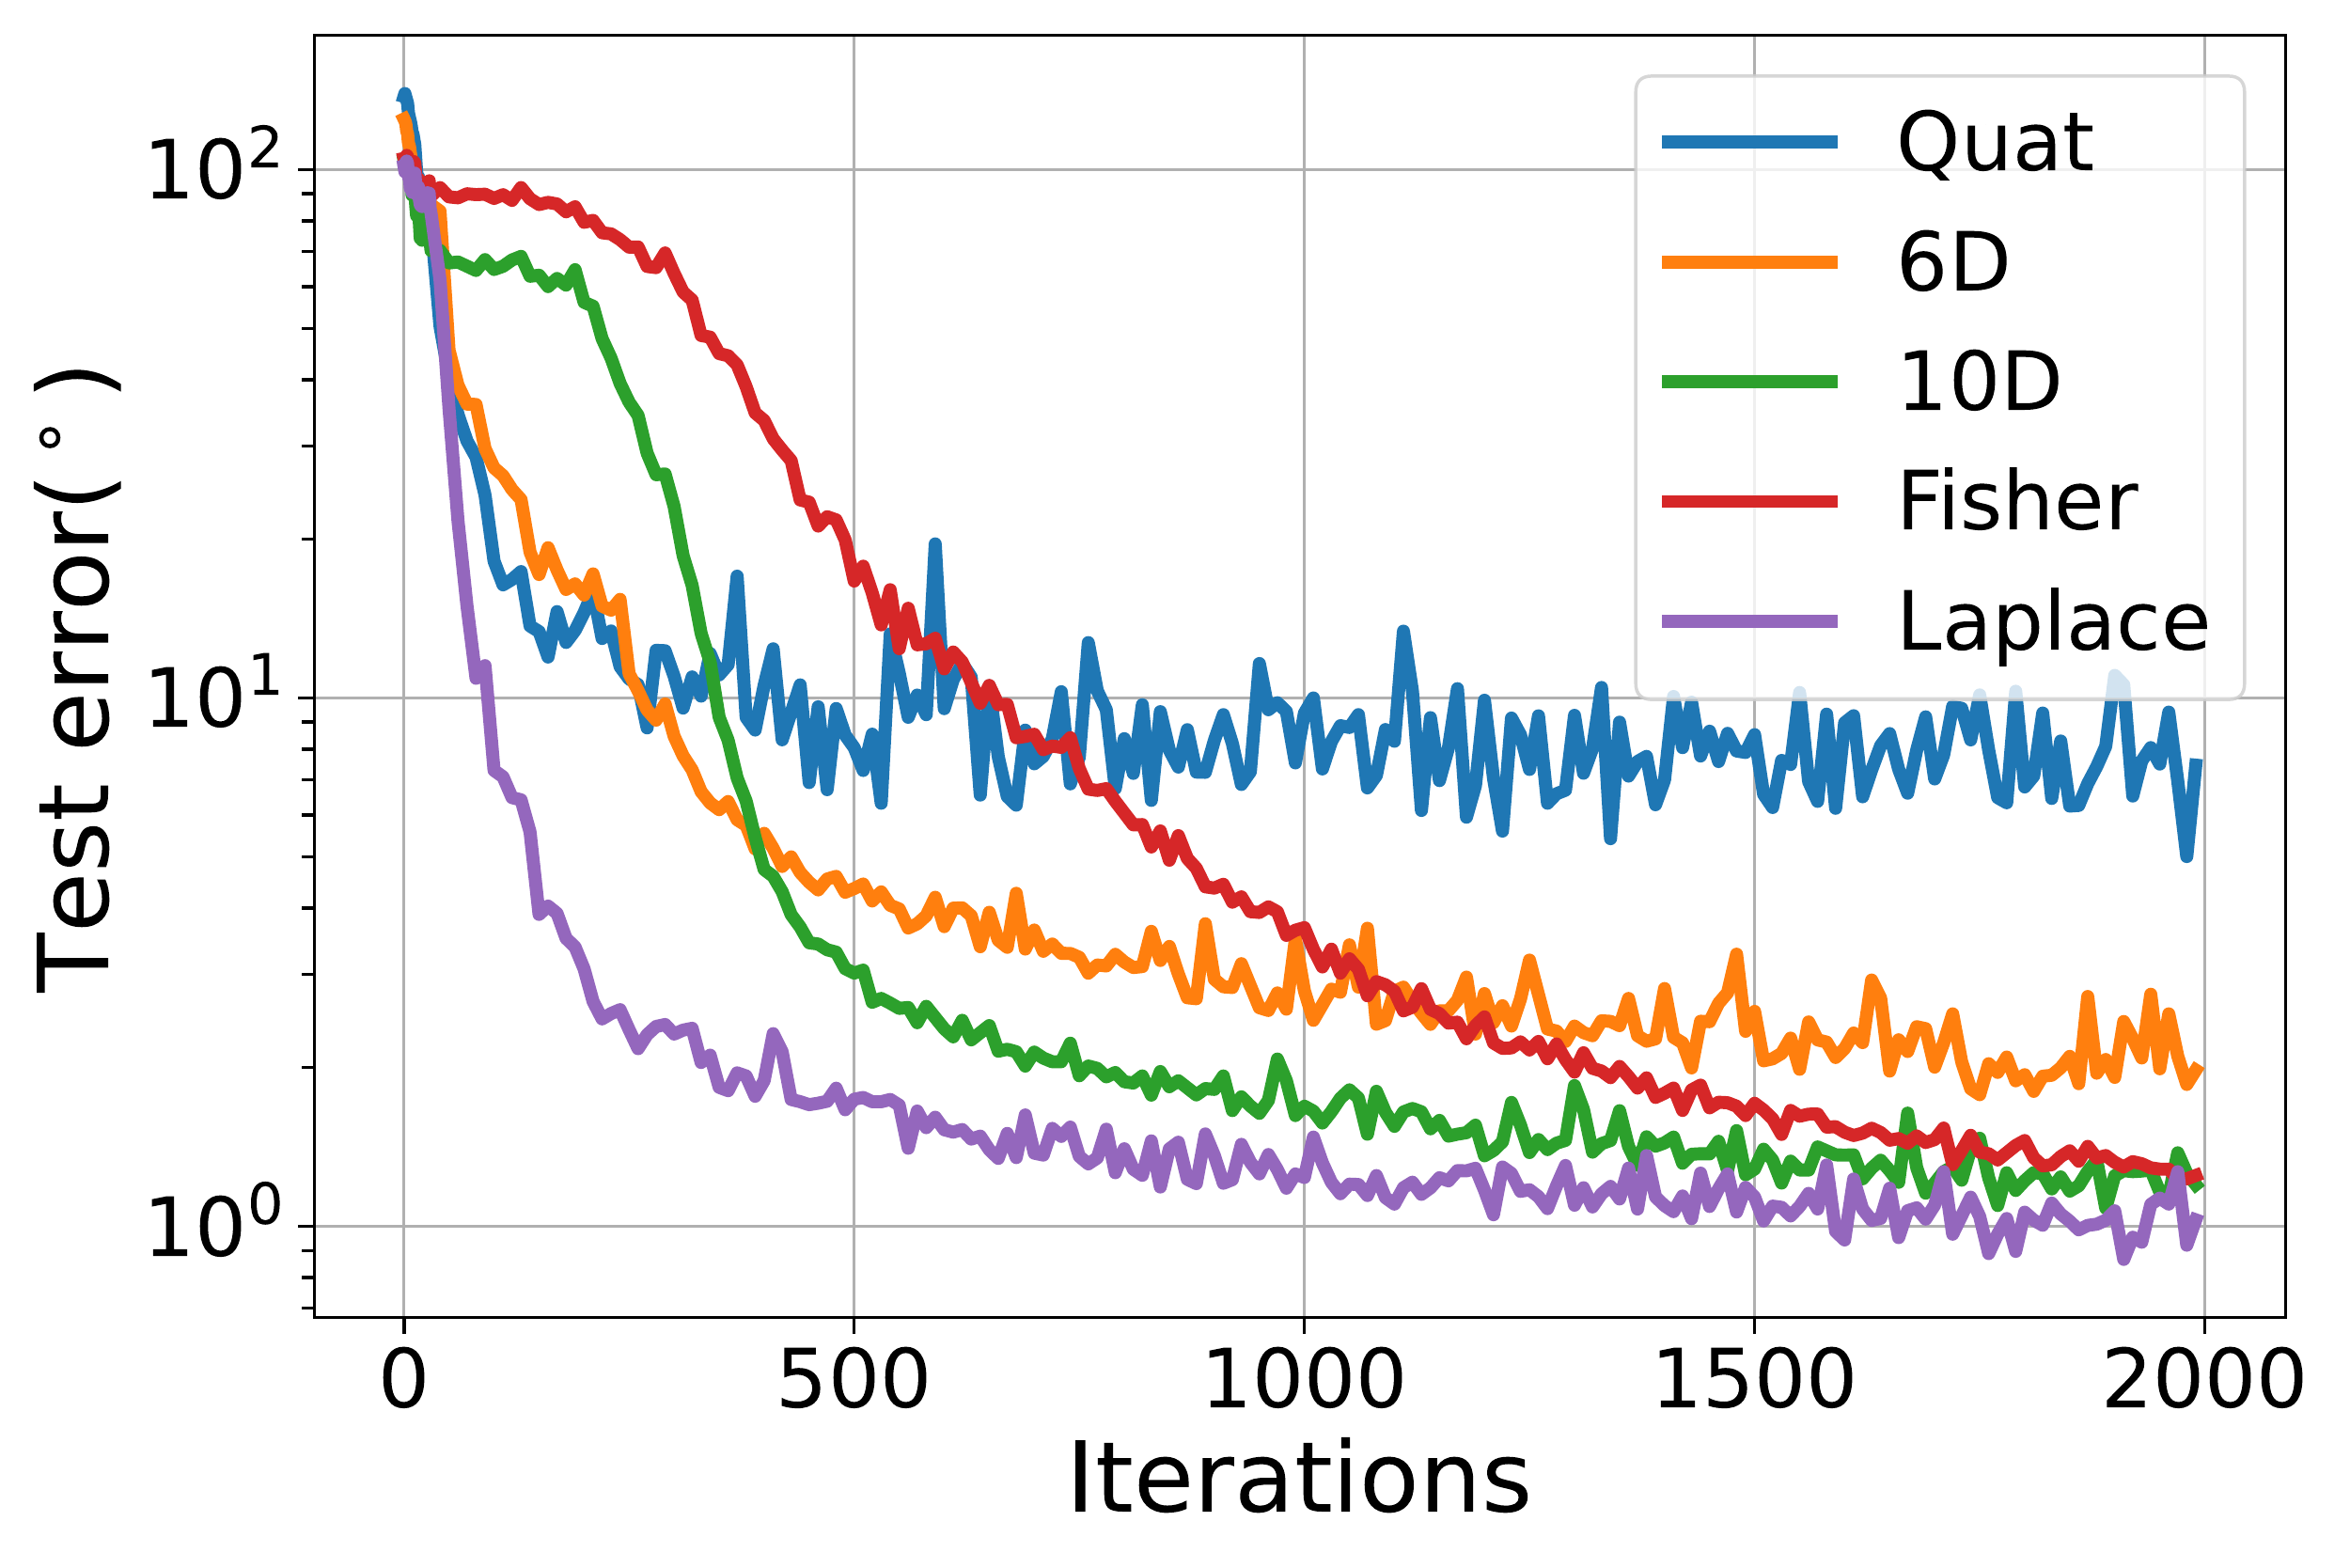} \hspace{2mm} &
    \includegraphics[width=0.35\linewidth]{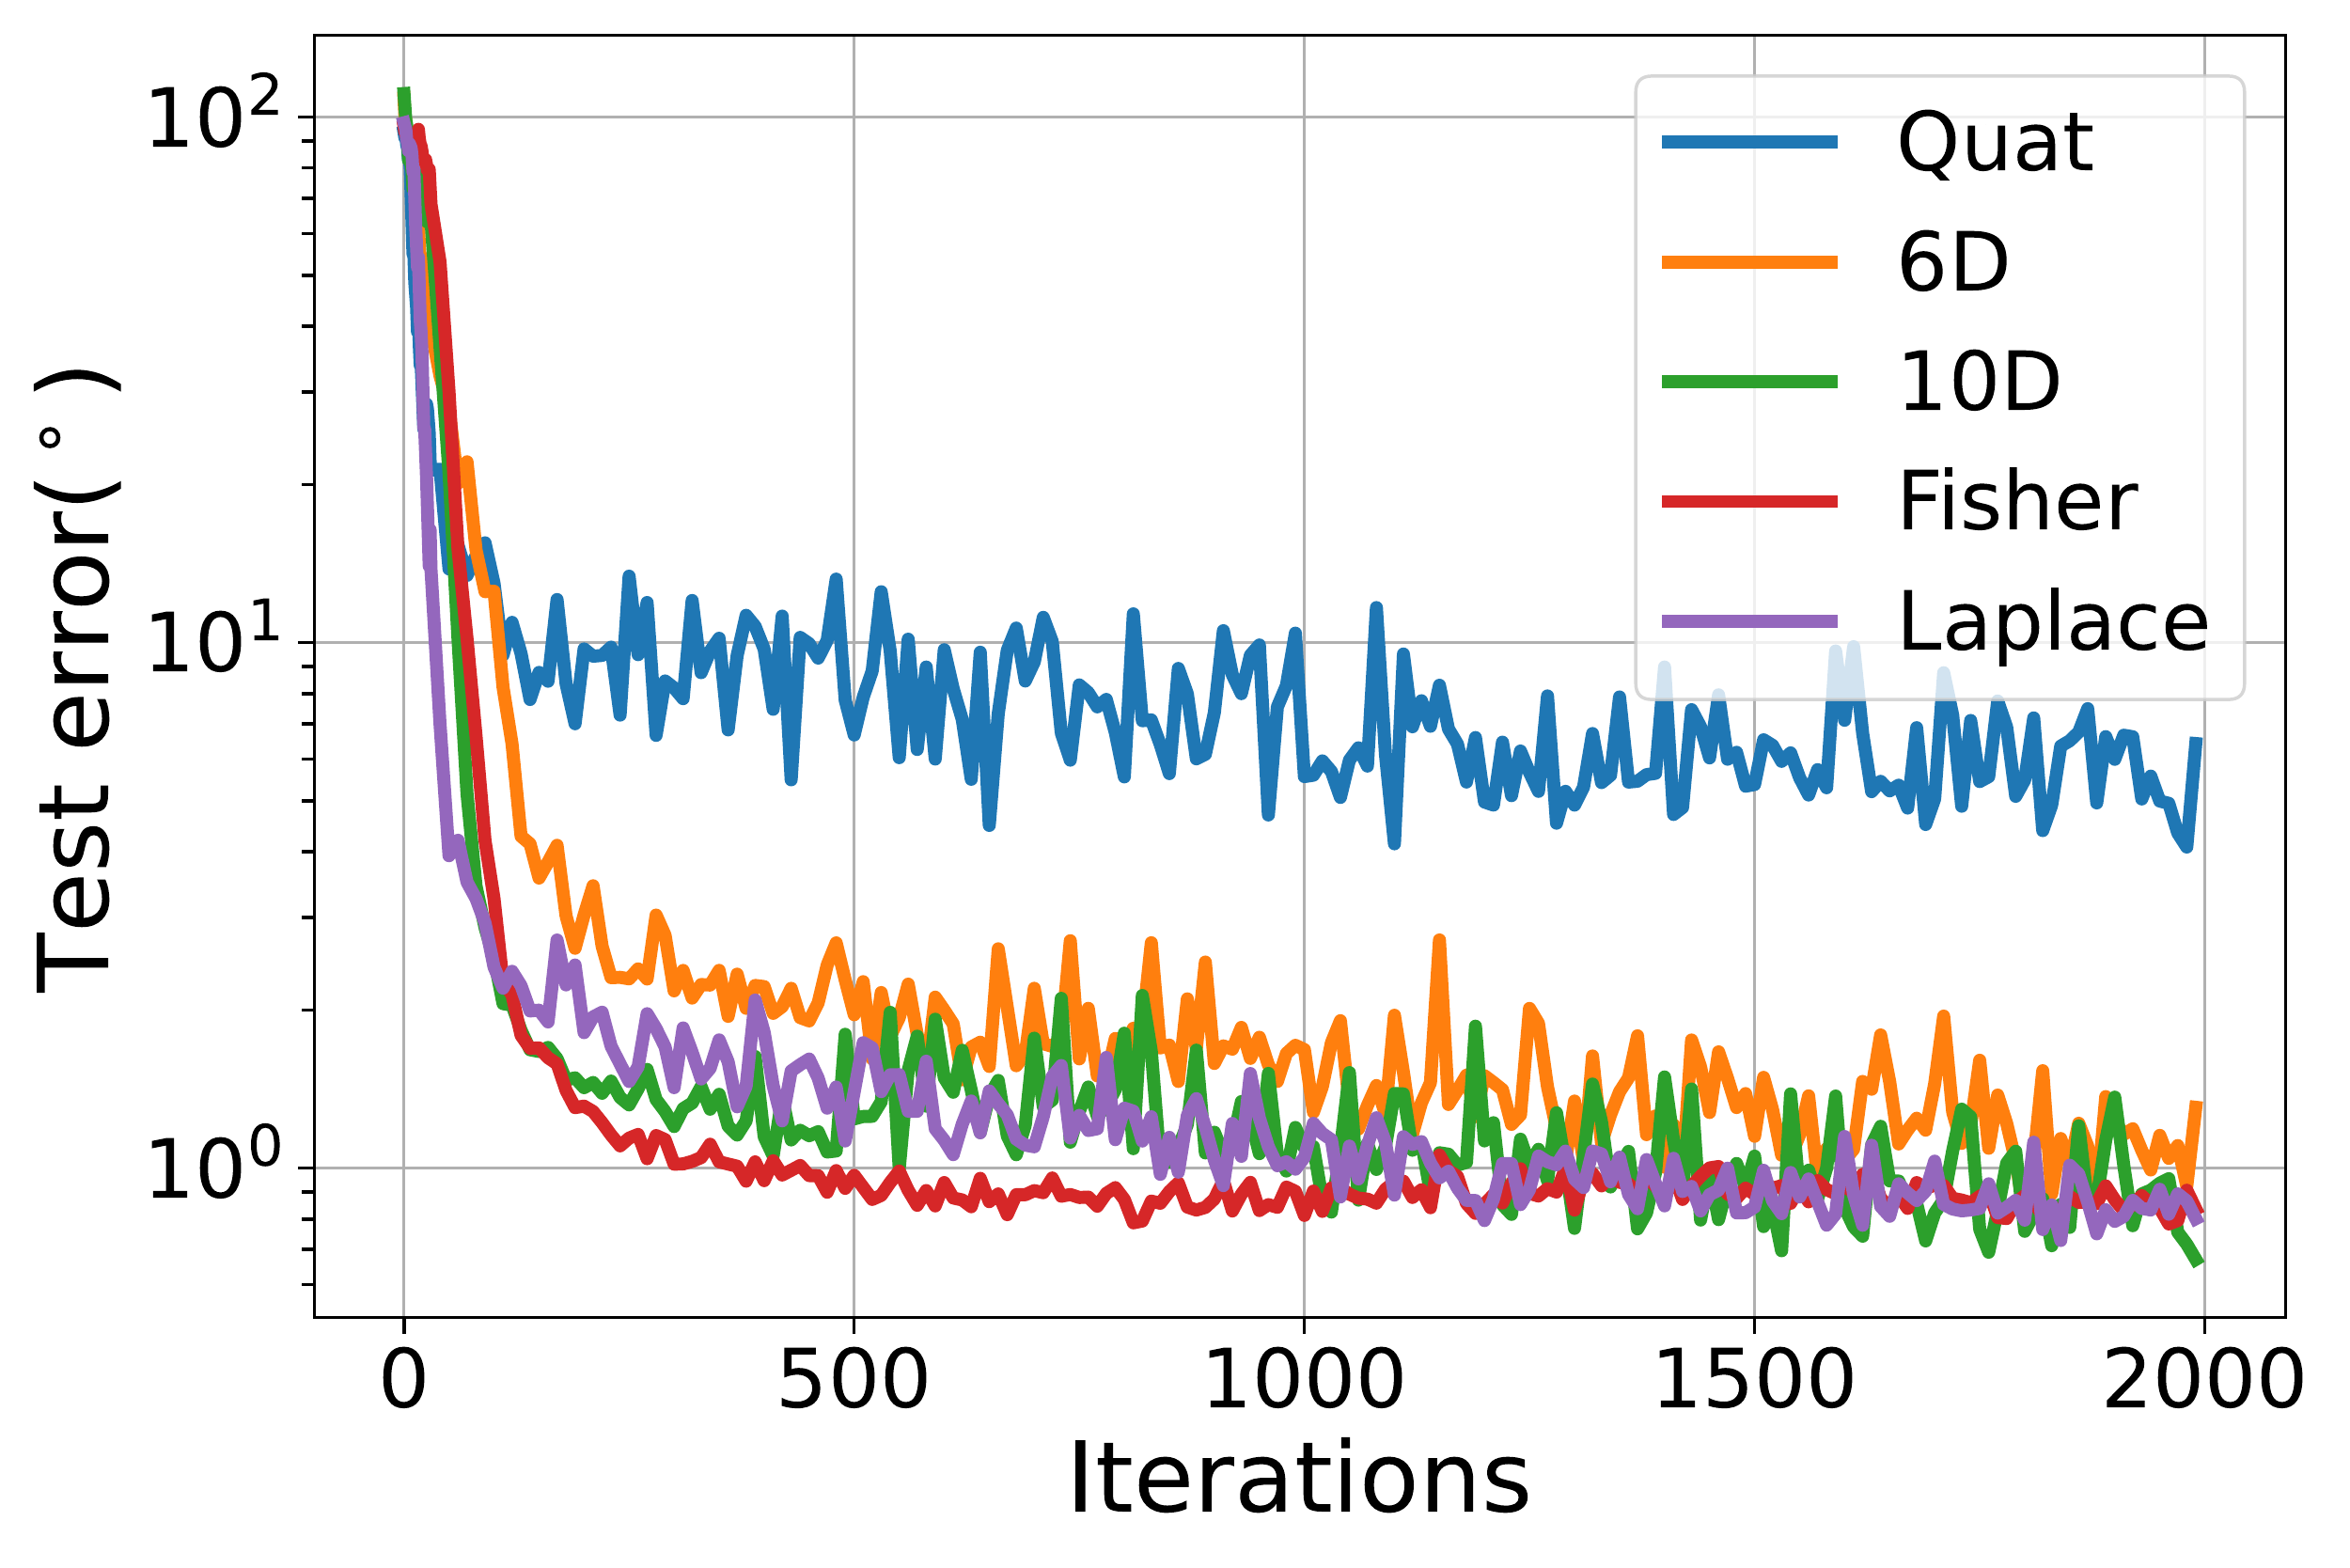} 
    \vspace{-2mm}    \\ 
    lr=$1e-5$  \hspace{2mm} &  lr=$1e-4$ \\
    \includegraphics[width=0.35\linewidth]{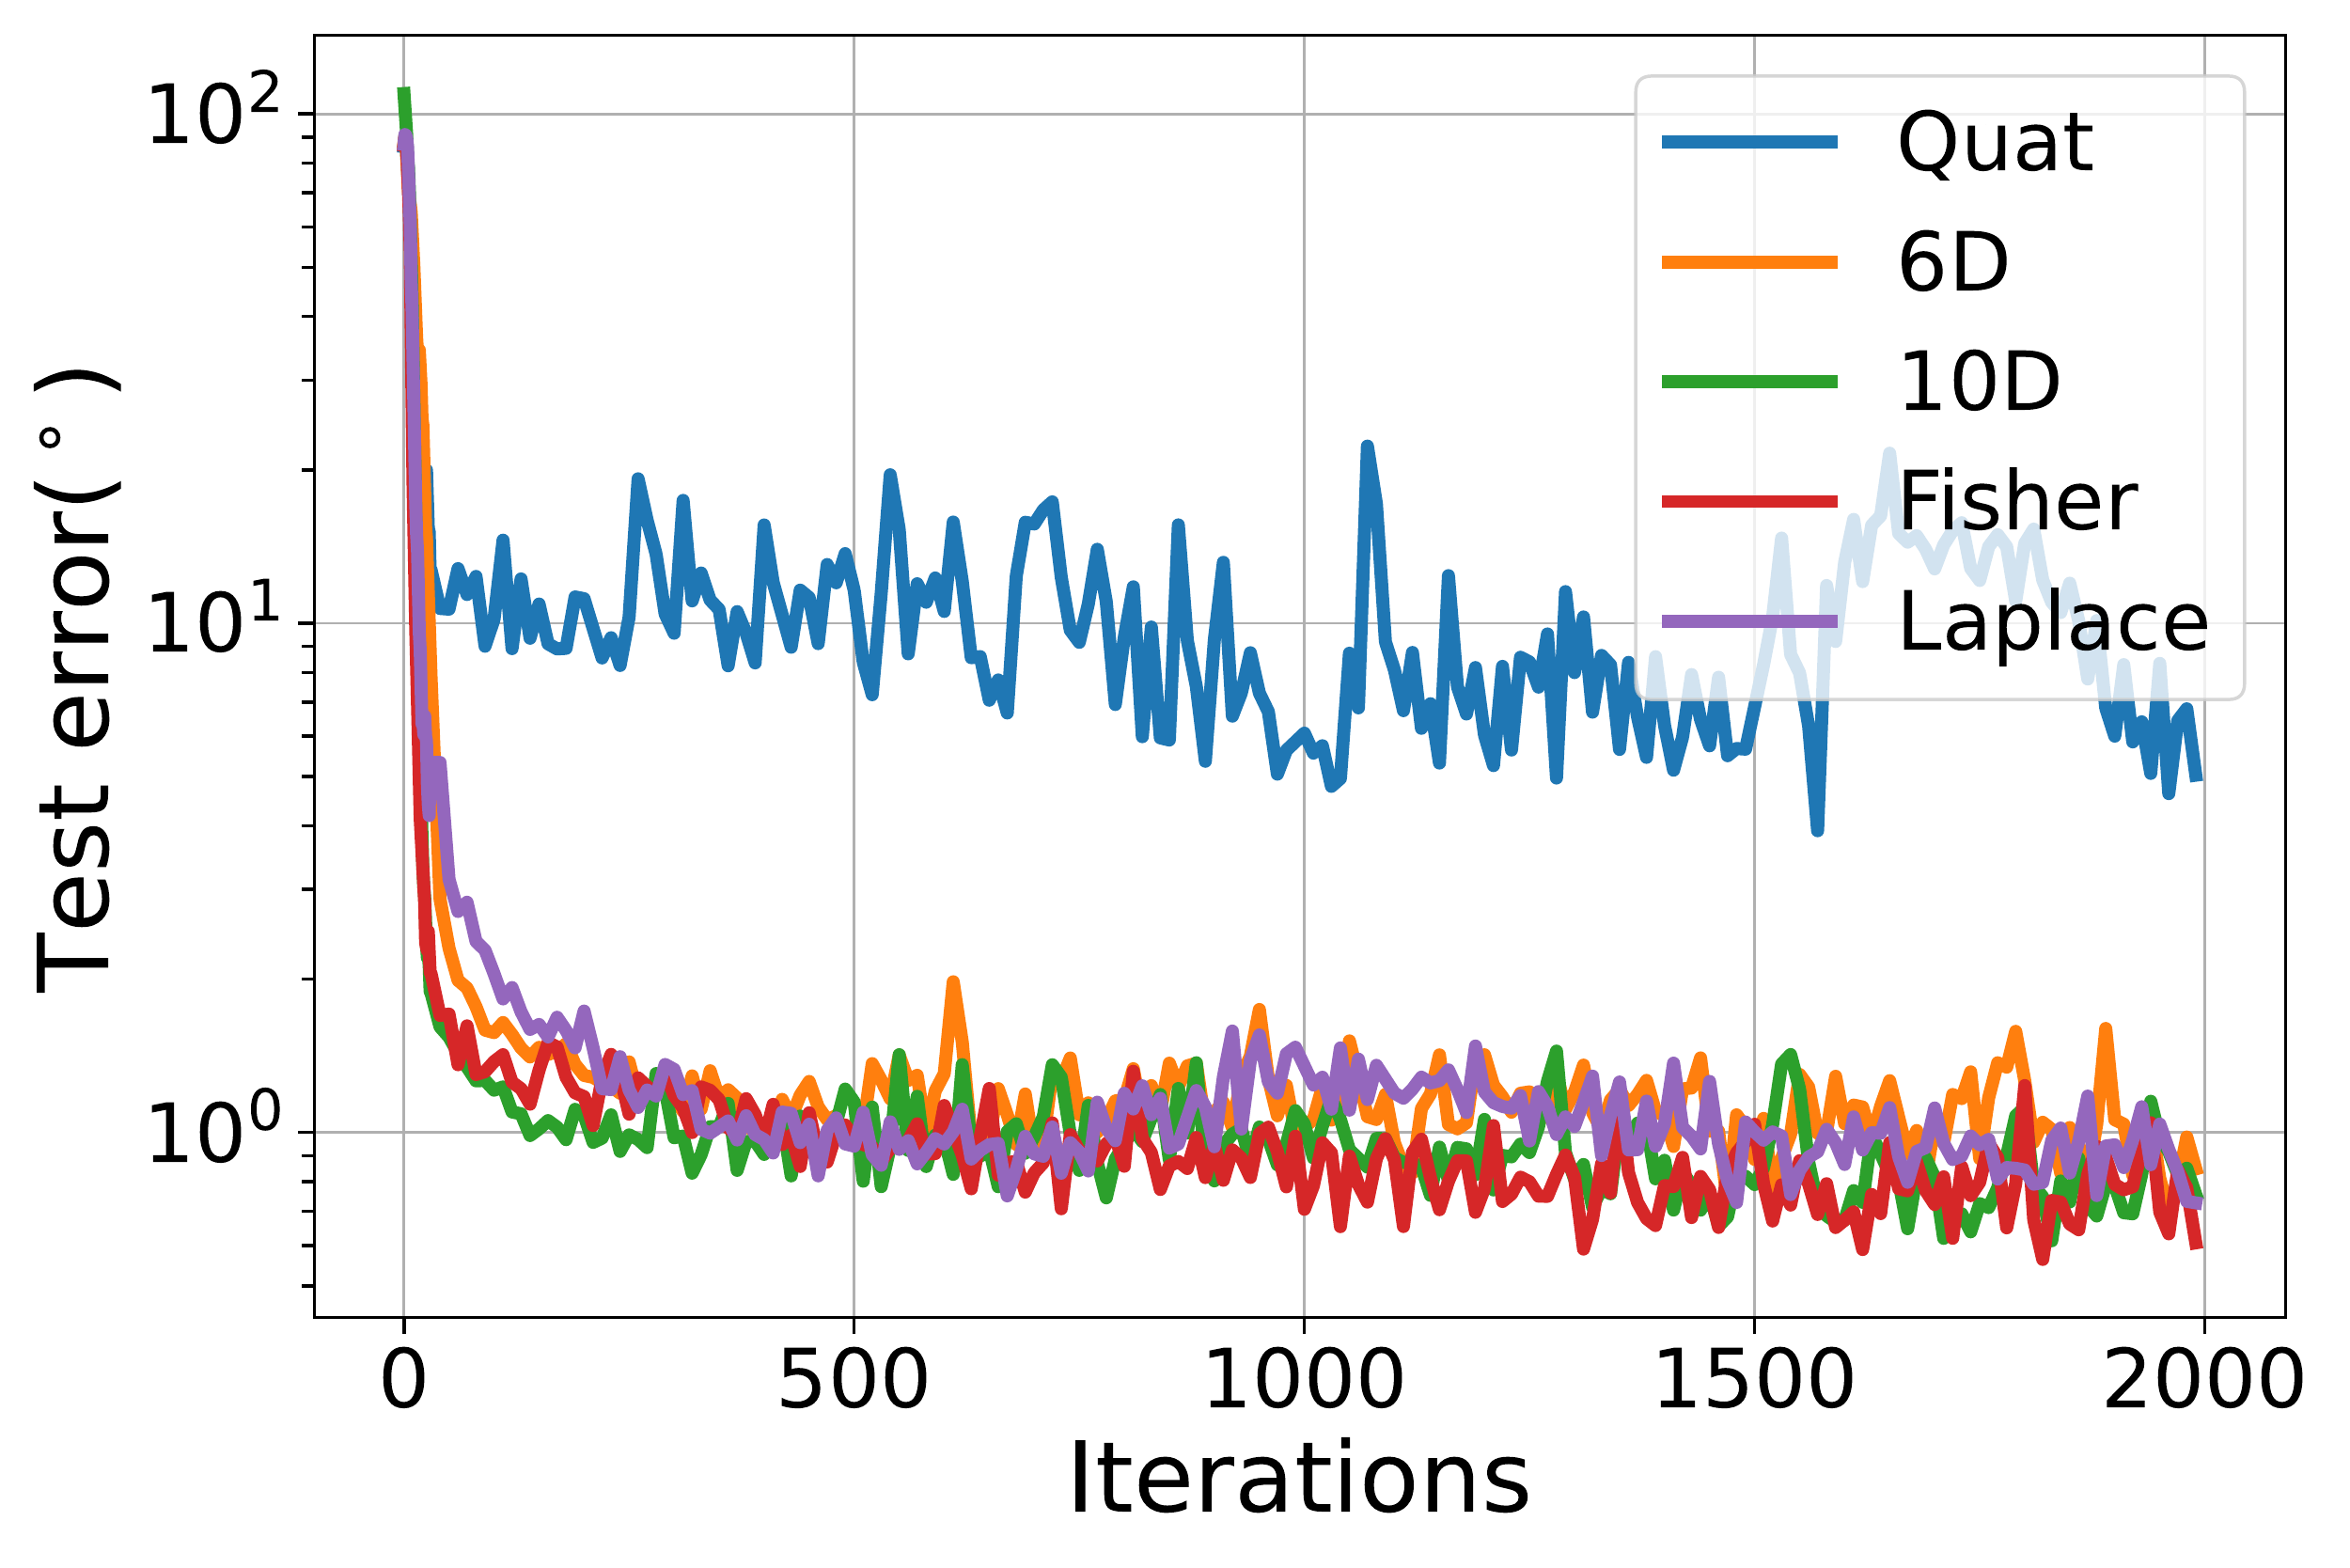} \hspace{2mm} &
    \includegraphics[width=0.35\linewidth]{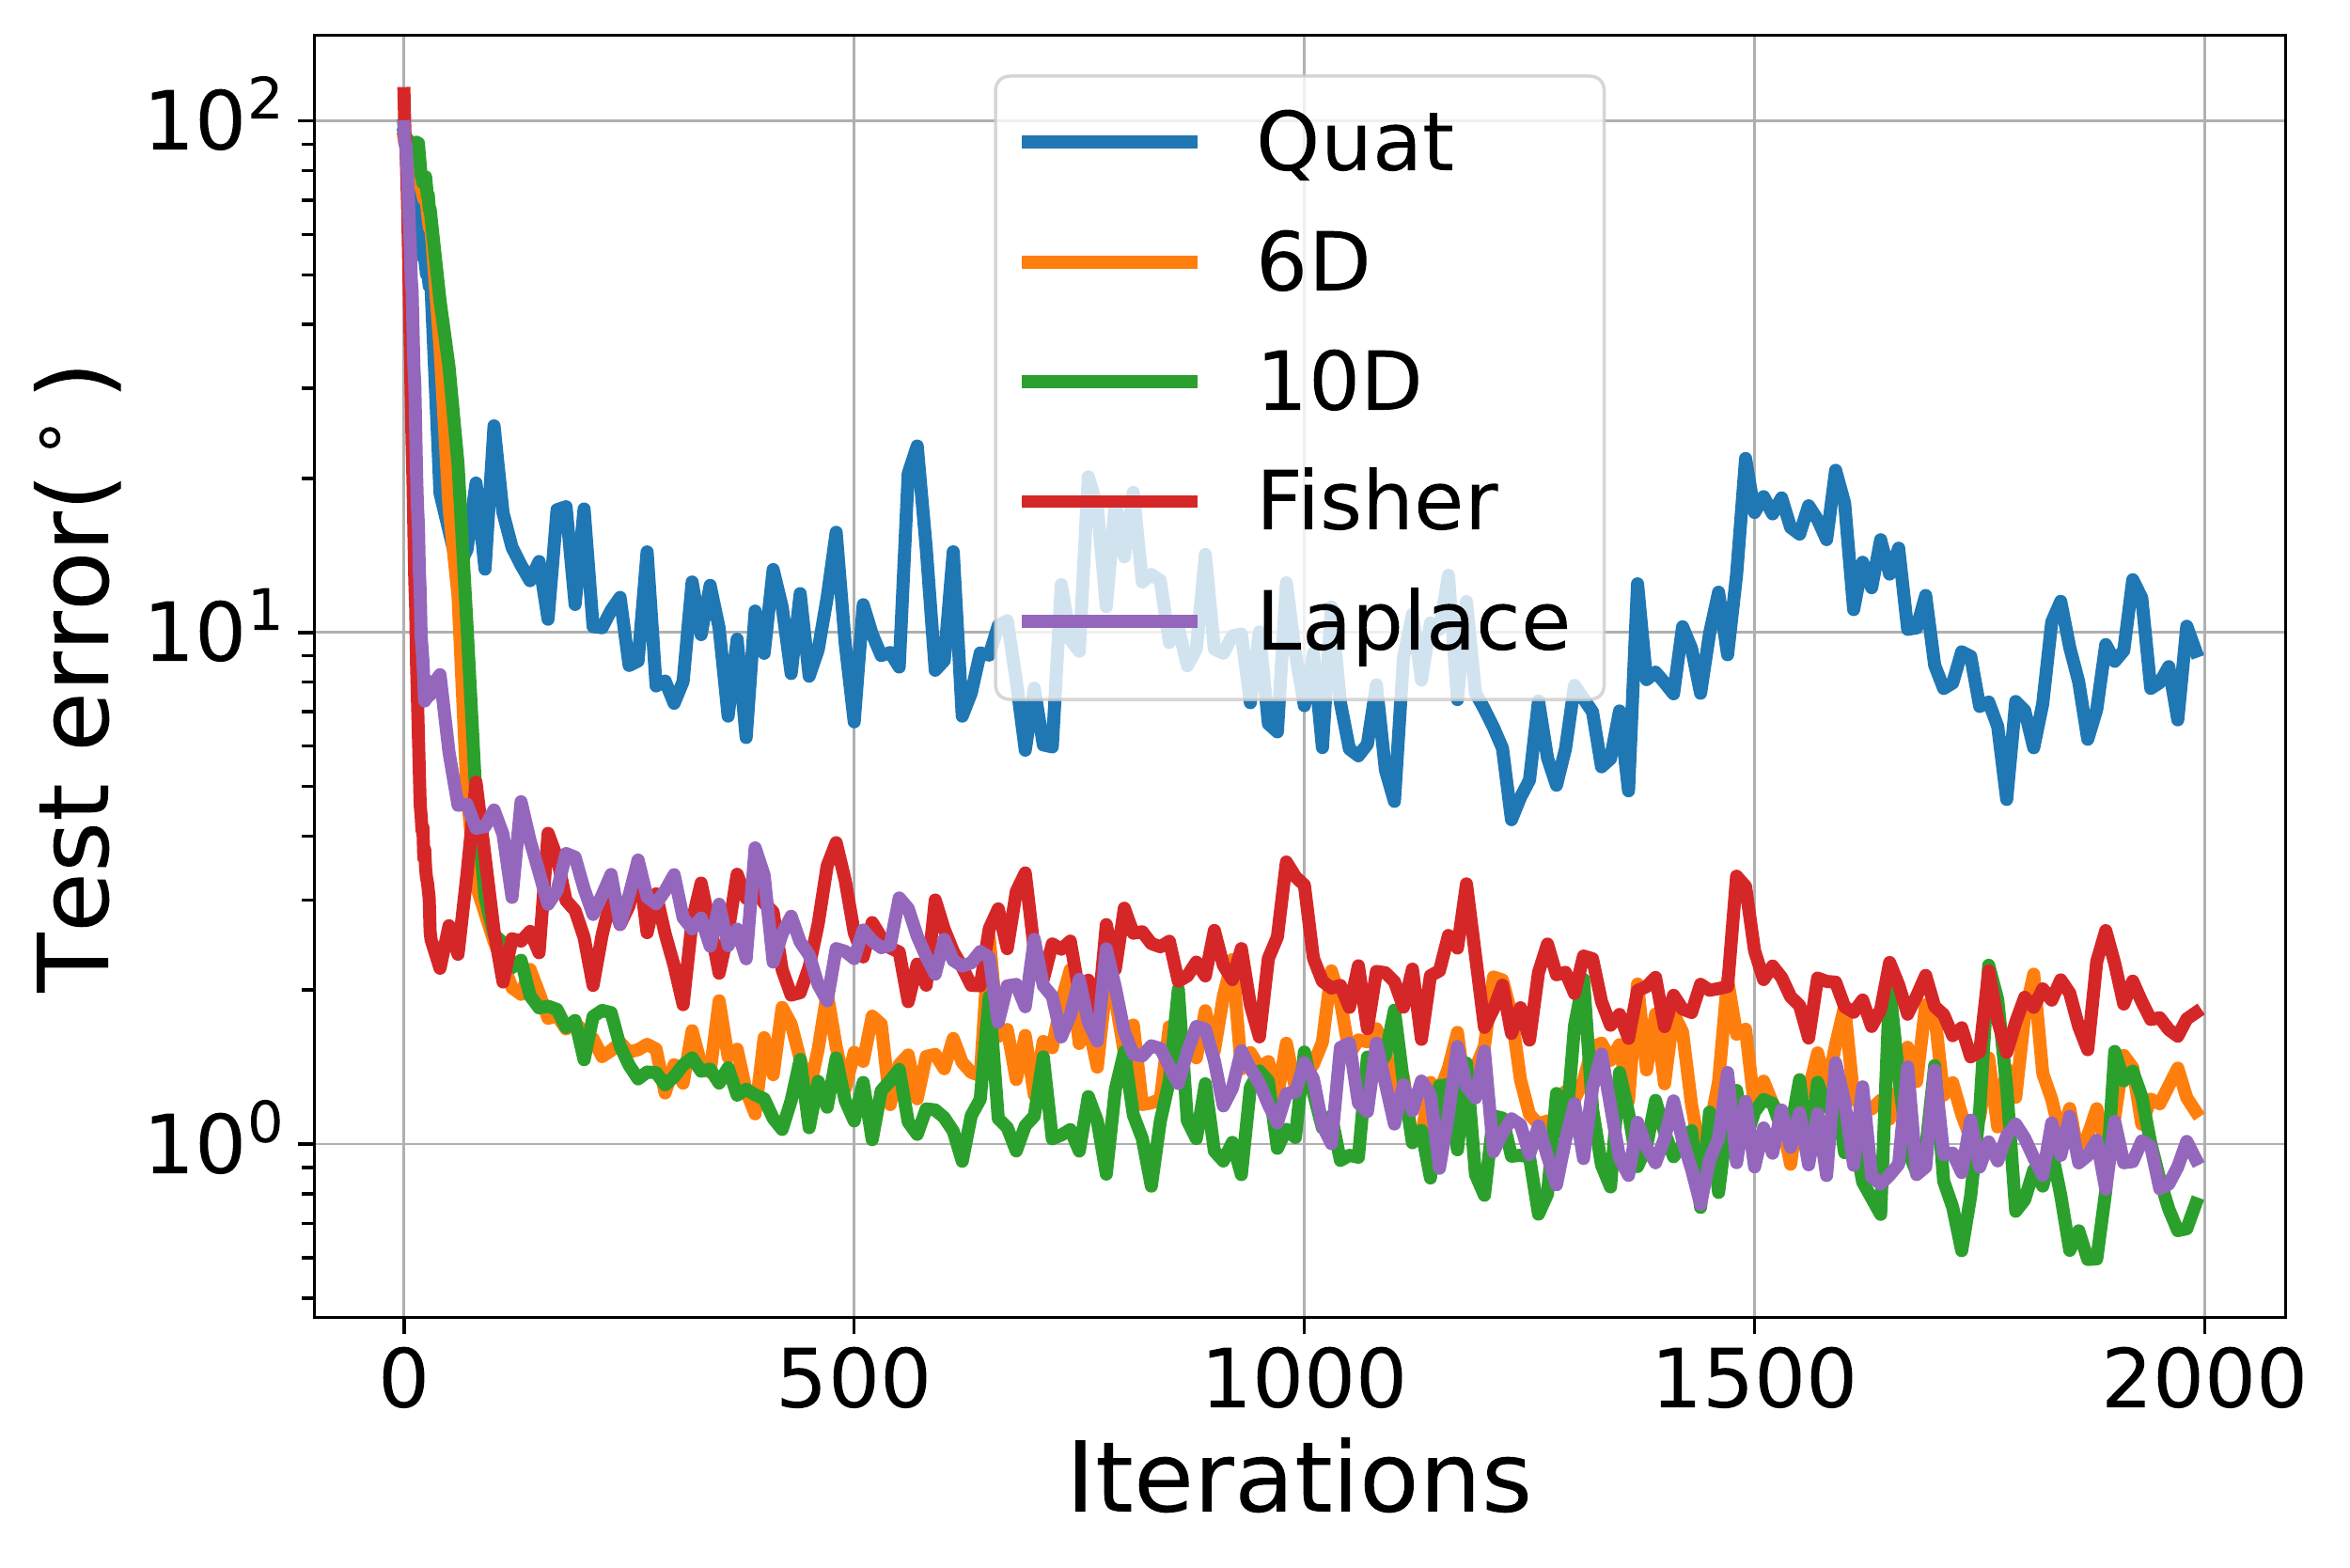} 
    \vspace{-2mm}    \\ 
    lr=$1e-3$  \hspace{2mm} &  lr=$1e-2$ \\     
    \end{tabular}
    \caption{\textbf{Visualization of the learning curves for instance-level Wahba's Problem.}}
    \label{fig:wahba_instance}
\end{figure*}
