# Supplementary material for: Towards Robust Probabilistic Modeling on SO(3) via Rotation Laplace Distribution
Source: arXiv:2305.10465 source file (2025-02-21)
Supplement: Supplementary file 3 [file math_mean.tex]

\textbf{Chordal Mean.} We define the \textit{chordal mean} \cite{hartley2013rotation,sarlette2009consensus,moakher2002means} of the distribution under the chordal metrics over $\SO$:
% . Given N rotations sampled from rotation Laplace distribution, the \textit{mean} of the distribution is defined as
\begin{equation}
% \footnotesize
    \Bar{\mathbf{R}} = \argmin_{\mathbf{R}\in \SO} \int_{\mathbf{R}^* \in \SO} p(\mathbf{R}^*) d_{\text{chord}}(\mathbf{R}, \mathbf{R}^*) \mathrm{d}\mathbf{R}^*
    % \| \mathbf{R} - \mathbf{R}^* \|^2
    \label{eq:definition}
\end{equation}
where $d_{\text{chord}}(\cdot, \cdot)$ denotes the L2 chordal metrics of two rotations:
\begin{equation}
    d_{\text{chord}}(\mathbf{R}_1, \mathbf{R}_2) = \| \mathbf{R}_1 - \mathbf{R}_2 \|_F^2
    % \arccos\left( \frac{\tr{\mathbf{R}_1^T\mathbf{R}_2}-1}{2} \right)
\end{equation}

The mean of our distribution under the chordal metrics is:
\begin{equation}
% \footnotesize
    \Bar{\mathbf{R}} = \mathbf{UV}^T
\end{equation}

% \begin{preliminary}
%     \begin{equation}
%         d_g(\mathbf{R}_1, \mathbf{R}_2) \propto \|\mathbf{R}_1 - \mathbf{R}_2\|
%     \end{equation}
%     \label{pre:distance}
% \end{preliminary}

% \begin{proof}
%     \todo{}
% \end{proof}

% The mean of our distribution under the chordal metrics is:
% \begin{equation}
% % \footnotesize
%     \Bar{\mathbf{R}} = \mathbf{UV}^T
% \end{equation}

\begin{proof}
    % Considering Eq. \ref{eq:definition} and Preliminary \ref{pre:distance},
    \begin{equation}
    \footnotesize
    \begin{aligned}
        % \Bar{\mathbf{R}} &= \argmin_{\mathbf{R}\in \SO} \int_{\mathbf{R}^* \in \SO} p(\mathbf{R}^*) d_g(\mathbf{R}, \mathbf{R}^*) \mathrm{d}\mathbf{R}^* \\
        \Bar{\mathbf{R}}&= \argmin_{\mathbf{R}\in \SO} \int_{\mathbf{R}^* \in \SO} p(\mathbf{R}^*) \| \mathbf{R} - \mathbf{R}^* \|^2_F \mathrm{d}\mathbf{R}^*
    \end{aligned}
    \end{equation}
    With Preliminary \ref{pre:norm},
    \begin{equation}
    \tiny
    \begin{aligned}
        \Bar{\mathbf{R}} 
        &= \argmin_{\mathbf{R}\in\SO} \left(-\int_{\mathbf{R}^* \in \SO} p(\mathbf{R}^*) \gamma^{-1}(\mathbf{R} )^T \gamma^{-1}(\mathbf{R}^*) \gamma^{-1}(\mathbf{R}^*)^T \gamma^{-1}(\mathbf{R}) \mathrm{d}\mathbf{R}^* \right) \\
        &= \argmin_{\mathbf{R}\in\SO} \left( -\gamma^{-1}(\mathbf{R})^T
        \left( \int_{\mathbf{R}^*\in\SO} p(\mathbf{R}^*) \gamma^{-1}(\mathbf{R}^*) \gamma^{-1}(\mathbf{R}^*) \mathrm{d}\mathbf{R}^* \right)  \gamma^{-1}(\mathbf{R})\right)
    \end{aligned}
    \end{equation}
    Let $\Bar{\mathbf{q}} = \gamma^{-1}(\Bar{\mathbf{R}})$, we have 
    \begin{equation}
    \footnotesize
        \Bar{\mathbf{q}} = \argmin_{\mathbf{q}\in \mathcal{S}^3}\left( -{\mathbf{q}}^T \left( \int_{\mathbf{q}^*\in \mathcal{S}^3} p(\mathbf{q}^*) \mathbf{q}^* \mathbf{q}^{*T} \mathrm{d}\mathbf{q}^*  \right) {\mathbf{q}} \right)
    \end{equation}
    We define
    \begin{equation}
    \footnotesize
    \footnotesize
        \mathcal{L}(\mathbf{q}) = -\mathbf{q}^{T} \left(
        \int_{\mathbf{q}^*\in \mathcal{S}^3} p(\mathbf{q}^*) \mathbf{q}^* \mathbf{q}^{*T} \mathrm{d}\mathbf{q}^*
        \right) \mathbf{q}
    \end{equation}
    then
    \begin{equation}
    \footnotesize
        \Bar{\mathbf{q}} = (\Bar{w}, \Bar{x}, \Bar{y}, \Bar{z}) = \argmin_{\mathbf{q}\in \mathcal{S}^3} \mathcal{L}(\mathbf{q})
    \end{equation}

    % We first consider the simple case when $\mathbf{A}=\mathbf{S}=\operatorname{diag}(s1, s2, s3)$. Otherwise, we apply a transformation $\mathbf{R}'=\mathbf{V}^T\mathbf{R}\mathbf{U}$.
    For rotation Laplace distribution,
    \begin{equation}
    \footnotesize
    \begin{aligned}
        p(\mathbf{R}; \mathbf{A}) 
        &= \frac{1}{F(\mathbf{A})} \frac{\exp\left(-\sqrt{\operatorname{tr}\left(\mathbf{S} - \mathbf{A}^T \mathbf{R}\right)}\right)}
        {\sqrt{\operatorname{tr}\left(\mathbf{S} -\mathbf{A}^T \mathbf{R}\right)}} \\ 
        & = \frac{1}{F(\mathbf{A})} \frac{\exp\left(-\sqrt{\operatorname{tr}(\mathbf{S}-\mathbf{S}\mathbf{U}^T\mathbf{R}\mathbf{V})}\right)}{\sqrt{\operatorname{tr}(\mathbf{S}-\mathbf{S}\mathbf{U}^T\mathbf{R}\mathbf{V})}} \\
        & \xlongequal{\mathbf{R}'=\mathbf{U}^T\mathbf{R}\mathbf{V}}  \frac{1}{F(\mathbf{A})} \frac{\exp\left(-\sqrt{\operatorname{tr}\left(\mathbf{S} - \mathbf{S}\mathbf{R}'\right)}\right)}
        {\sqrt{\operatorname{tr}\left(\mathbf{S} -\mathbf{S}\mathbf{R}'\right)}} 
    \end{aligned}
    \end{equation}

    Below we first consider the geodesic mean of  $\mathbf{R}'$, denoted as $\Bar{\mathbf{R}}'$, and then 
    \begin{equation}
        \Bar{\mathbf{R}} = \mathbf{U}\Bar{\mathbf{R}}'\mathbf{V}^T
        \label{eq:rprime}
    \end{equation}
    
    % We consider the simple case when $\mathbf{A}=\mathbf{S}$. Otherwise, we apply a transformation $\mathbf{R}'=\mathbf{V}^T\mathbf{R}\mathbf{U}$, such that the distribution follows the simple case.
    
    % Given $\mathbf{R}'=\mathbf{U}^T\mathbf{R}\mathbf{V}$, and c
    Considering the transformation between rotation matrix and unit quaternion Eq. \ref{eq:r_to_q},  we have 
    \begin{equation}
    \begin{aligned}
    \footnotesize
        &p(w,x,y,z;\mathbf{A}) \\
        =& \frac{1}{F(\mathbf{A})} \frac{\exp\left(
        -\sqrt{2(s_2+s_3) x^2 + 2(s_1+s_3) y^2 + 2(s_1+s_2)z^2}
        \right)}{\sqrt{2(s_2+s_3) x^2 + 2(s_1+s_3) y^2 + 2(s_1+s_2)z^2}}
        \label{eq:pdf_q}
    \end{aligned}
    \end{equation}

    Given the even function property of Eq. \ref{eq:pdf_q}, we have
    \begin{equation}
    \footnotesize
        p(w,x,y,z) = p(w,-x,y,z) = p(w,x,-y,z) = p(w,x,y,-z)
    \end{equation}
    and 
    \begin{equation}
    \footnotesize
        \mathcal{L}(w,x,y,z) = \mathcal{L}(w,-x,y,z) = \mathcal{L}(w,x,-y,z) = \mathcal{L}(w,x,y,-z)
    \end{equation}
    and thus the four quaternions should all be the mean of the distribution: 
    $(\Bar{w}, \Bar{x}, \Bar{y}, \Bar{z})$, $(\Bar{w}, -\Bar{x}, \Bar{y}, \Bar{z})$, $(\Bar{w}, \Bar{x}, -\Bar{y}, \Bar{z})$, $(\Bar{w}, \Bar{x}, \Bar{y}, -\Bar{z})$.
    % $(w^*, -x^*, y^*, z^*)$, $(w^*, x^*, -y^*, z^*)$, $(w^*, x^*, y^*, -z^*)$
    Due to the uniqueness of the mean, the four quaternions should be identical, and thus $(\Bar{w}, \Bar{x}, \Bar{y}, \Bar{z})$ must be an item in the set $\mathcal{Q}=\{(1, 0, 0, 0)$, $(0, 1, 0, 0)$, $(0, 0, 1, 0)$, $(0, 0, 0, 1)\}$, i.e.,
    % one of the four values: $(1, 0, 0, 0)$, $(0, 1, 0, 0)$, $(0, 0, 1, 0)$, $(0, 0, 0, 1)$.
    % Since the mean of the distribution is unique, we denote it as $(w^*, x^*, y^*, z^*)$. 
    % Then $(w^*, -x^*, y^*, z^*)$, $(w^*, x^*, -y^*, z^*)$, $(w^*, x^*, y^*, -z^*)$ should be the same unit quaternion as $(w^*, x^*, y^*, z^*)$.
    % Therefore, $(w^*, x^*, y^*, z^*)$ must be one of the four values: $(1, 0, 0, 0)$, $(0, 1, 0, 0)$, $(0, 0, 1, 0)$, $(0, 0, 0, 1)$.
    \begin{equation}
    \footnotesize
        \Bar{\mathbf{q}} = (\Bar{w}, \Bar{x}, \Bar{y}, \Bar{z}) = \argmin_{\mathbf{q}\in \mathcal{Q}}
        \mathcal{L}(\mathbf{q})
    \end{equation}

    Now we compare $\mathcal{L}(1, 0, 0, 0)$, $\mathcal{L}(0, 1, 0, 0)$

    \begin{equation}
    \footnotesize
    \begin{aligned}
        \mathcal{L}(1, 0, 0, 0) 
        &= -(1, 0, 0, 0)\int_{\mathcal{S}^3}p(\mathbf{q}) \mathbf{q} \mathbf{q}^T \mathrm{d}\mathbf{q}
        \begin{pmatrix}
      1  \\
      0\\
      0 \\
      0
        \end{pmatrix}\\
        % &\xlongequal{\mathbf{q} = (w, x, y, z)}
        % &\overset{q = (w, x, y, z)}{=} 
        &=
        -\int_{\mathcal{S}^3}w^2  p(w,x,y,z) \mathrm{d}(w,x,y,z) \\
        &= -\frac{1}{2} \int_{\mathcal{S}^3} (w^2 p(w, x,y,z) + x^2 p(x, w,y,z) )
         \mathrm{d}(w, x, y,z) 
        \end{aligned}
        \end{equation}
    
    Similarly,
    \begin{equation}
    \footnotesize
    \begin{aligned}
         \mathcal{L}(0, 1, 0, 0) &=
         -\int_{\mathcal{S}^3}x^2  p(w,x,y,z) \mathrm{d}(w,x,y,z) \\
         &= -\frac{1}{2} \int_{\mathcal{S}^3} (x^2 p(w,x,y,z) +w^2 p(x,w,y,z)) 
         \mathrm{d}(w, x, y,z) 
    \end{aligned}
    \end{equation}

    Therefore,
    \begin{equation}
    \footnotesize
    \begin{aligned}
        &\mathcal{L}(0, 1, 0, 0) - \mathcal{L}(1, 0, 0, 0)  \\ =&
        \frac{1}{2} \int_{\mathcal{S}^3} ((w^2 p(w, x,y,z) + x^2 p(x, w,y,z) \\
        &- x^2 p(w,x,y,z) -w^2 p(x,w,y,z))
         \mathrm{d}(w, x, y,z) 
        \\ =& \frac{1}{2} \int_{\mathcal{S}^3}
        (w^2-x^2)(p(w,x,y,z) - p(x, w, y,z)) \mathrm{d}(w,x,y,z) 
    \end{aligned}
    \end{equation}

    Considering Eq. \ref{eq:pdf_q},  $p(w,x,y,z)$ monotonically decreases wrt.
    $2(s_2 + s_3)x^2 + 2(s_1 + s_3)y^2 + 2(s_1 + s_2)z^2$.
    We have
    \begin{equation}
    \footnotesize
    \begin{aligned}
        & x^2 \le w^2 \\
        \Leftrightarrow & 2(s_2 + s_3)x^2 + 2(s_1 + s_3)y^2 + 2(s_1 + s_2)z^2 \\
        &\le 2(s_2 + s_3)w^2 + 2(s_1 + s_3)y^2 + 2(s_1 + s_2)z^2\\
        \Leftrightarrow & p(w,x,y,z) \ge p(x,w,y,z)
    \end{aligned}
    \end{equation}
    Therefore, $(w^2-x^2)$ and $(p(w,x,y,z) - p(x, w, y,z))$ have the same sign, i.e.,
    \begin{equation}
    \footnotesize
        (w^2-x^2)(p(w,x,y,z) - p(x, w, y,z)) \ge 0
    \end{equation}
    and 
    \begin{equation}
    \footnotesize
        \mathcal{L}(0,1,0,0) \ge \mathcal{L}(1,0,0,0)
    \end{equation}
    % Therefore, $w^2 \ge x^2 \Leftrightarrow p(w,x,y,z) \ge p(x, w, y, z)$
    % and $L(0,1,0,0) \ge L(1,0,0,0).$
    Similarly, $\mathcal{L}(0,0,1,0) \ge \mathcal{L}(1,0,0,0)$ and $\mathcal{L}(0,0,0,1) \ge \mathcal{L}(1,0,0,0)$.

    Therefore, $\mathcal{L}(1,0,0,0)$ has the minimum value, and $\Bar{\mathbf{q}}=(1,0,0,0)$, $\Bar{\mathbf{R}}'=\mathbf{I}$. 
    
    Finally, considering Eq. \ref{eq:rprime},
    \begin{equation}
    % \footnotesize
        \Bar{\mathbf{R}} = \mathbf{UIV}^T = \mathbf{UV}^T
    \end{equation}
    
\end{proof}

\begin{preliminary}
    Denote the transformation between rotation matrix and unit quaternion as $\mathbf{R}=\gamma(\mathbf{q})$.
    For rotations $\mathbf{R}_1$ and $\mathbf{R}_2$, we have 
    \begin{equation}
    \footnotesize
        \|\mathbf{R}_1 - \mathbf{R}_2\|^2_F = 8(1-\gamma^{-1}(\mathbf{R}_1)^T \gamma^{-1}(\mathbf{R}_2) \gamma^{-1}(\mathbf{R}_2)^T \gamma^{-1}(\mathbf{R}_1))
    \end{equation}
    \label{pre:norm}
\end{preliminary}

\begin{proof}
    Let $\gamma^{-1}(\mathbf{R}_1) = (w_1, x_1, y_1, z_1)$, $\gamma^{-1}(\mathbf{R}_2) = (w_2, x_2, y_2, z_2)$, $\gamma^{-1}(\mathbf{R}_1^T\mathbf{R}_2) = (w', x', y', z')$, then 
    \begin{equation}
    \footnotesize
        \mathbf{R}_1^T \mathbf{R}_2 = \begin{pmatrix} 1-2y'^2-2z'^2 & 2x'y'-2z'w' & 2x'z'+2y'w' \\ 2x'y'+2z'w' & 1-2x'^2-2z'^2 & 2y'z'-2x'w' \\ 2x'z'-2y'w' & 2y'z'+2x'w' & 1-2x'^2-2y'^2 \end{pmatrix}
    \end{equation}

    % \begin{equation}
    % \footnotesize
    %     \| \mathbf{R}_1 - \mathbf{R}_2 \|^2_F = \| \mathbf{R}_1^T (\mathbf{R}_1 - \mathbf{R}_2) \|^2_F = \| \mathbf{I} - \mathbf{R}_1^T\mathbf{R}_2 \|^2_F
    % \end{equation}

    Therefore, 
    \begin{equation}
    \footnotesize
    \begin{aligned}
        &\| \mathbf{R}_1 - \mathbf{R}_2 \|^2_F \\
        = &\| \mathbf{R}_1^T (\mathbf{R}_1 - \mathbf{R}_2) \|^2_F \\ =& \| \mathbf{I} - \mathbf{R}_1^T\mathbf{R}_2 \|^2_F \\ =& \left\| \mathbf{I} - \begin{pmatrix} 1-2y'^2-2z'^2 & 2x'y'-2z'w' & 2x'z'+2y'w' \\ 2x'y'+2z'w' & 1-2x'^2-2z'^2 & 2y'z'-2x'w' \\ 2x'z'-2y'w' & 2y'z'+2x'w' & 1-2x'^2-2y'^2 \end{pmatrix} \right\|^2_F \\
         =&8(1-w'^2)
    \end{aligned}
    \end{equation}
Since $\mathrm{conj}\left(\gamma^{-1}(\mathbf{R}_1)\right) \times \gamma^{-1}(\mathbf{R}_2)=\gamma^{-1}(\mathbf{R}_1^T\mathbf{R}_2)$, we have 
\begin{equation}
\footnotesize
\begin{aligned}
    w' &= -w_1w_2-x_1x_2-y_1y_2-z_1z_2 \\
    &=-\gamma^{-1}(\mathbf{R}_1)^T \gamma^{-1}(\mathbf{R}_2)
\end{aligned}
\end{equation}
Therefore,
\begin{equation}
\footnotesize
    \begin{aligned}
        &8(1-w'^2) \\
        =& 8(1-(\gamma^{-1}(\mathbf{R}_1)^T\gamma^{-1}(\mathbf{R}_2))^2) \\
        =& 8(1-\gamma^{-1}(\mathbf{R}_1)^T \gamma^{-1}(\mathbf{R}_2) \gamma^{-1}(\mathbf{R}_2)^T \gamma^{-1}(\mathbf{R}_1))
    \end{aligned}
\end{equation}
\end{proof}

We did not find a proper definition of higher order moments under the chordal metrics.
