# Supplementary material for: Towards Robust Probabilistic Modeling on SO(3) via Rotation Laplace Distribution
Source: arXiv:2305.10465 source file (2025-02-21)
Supplement: Supplementary file 4 [file mode_uniqueness.tex]

\section{Mode Uniqueness}
The mode of our distribution may not be unique depending on the singular values. The detailed study is shown as below:

For rotation Laplace distribution
\begin{equation}
    p(\mathbf{R}; \mathbf{A})
    = \frac{1}{F(\mathbf{A})} \frac{\exp\left(-\sqrt{\operatorname{tr}\left(\mathbf{S} - \mathbf{A}^T \mathbf{R}\right)}\right)}
    {\sqrt{\operatorname{tr}\left(\mathbf{S} -\mathbf{A}^T \mathbf{R}\right)}},
\end{equation}
let $s_1, s_2, s_3$ be the proper singular values of the parameter $\mathbf{A}$,
the mode of the distribution is computed as
\begin{equation*}
    \mathbf{R}_0 = \begin{cases} 
        \mathbf{UV}^T,  &\text{case1}
        % s_2 + s_3 > 0 
        \\ 
        \mathbf{U} \left(\begin{smallmatrix} 1 & 0 & 0 \\ 0 & 1-2x^2 & -2xw \\ 0 & 2xw & 1-2x^2 \end{smallmatrix}\right) \mathbf{V}^T,  &\text{case2}
        % s_2+s_3=0, s_1+s_3>0 
        \\
        \mathbf{U} \left(\begin{smallmatrix} 1-2y^2 & 2xy & 2yw \\ 2xy & 1-2x^2 & -2xw \\ -2yw & 2xw & 1-2x^2-2y^2 \end{smallmatrix} \right) \mathbf{V}^T, 
        &\text{case3}
        % s_2+s_3=0, s_1+s_3=0, s_1+s_2>0 
        \\
        \text{ill-defined}, &\text{case4}
        % s_2+s_3=0, s_1+s_3=0, s_1+s_2=0
\end{cases}
\end{equation*}

\begin{equation*}
\begin{aligned}
    &\text{case1:} s_2 + s_3 > 0 \\
    &\text{case2:} s_2+s_3=0, s_1+s_3>0 \\
    &\text{case3:} s_2+s_3=0, s_1+s_3=0, s_1+s_2>0 \\
    &\text{case4:} s_2+s_3=0, s_1+s_3=0, s_1+s_2=0
\end{aligned}
\end{equation*}
where $\mathbf{q}'=(w, x, y, z)$ is the corresponding unit quaternion of the rotation matrix $\mathbf{U}^T\mathbf{RV}$ (see Eq.\ref{eq:r_to_q}).

With the help of the visualization method \cite{murphy2021implicit}, we show the modes in different cases in Figure \ref{fig:unique_vis}.

% \yingda{We noticed that matrix Fisher distribution has the similar mode uniqueness property with ours.}

\begin{figure*}[h]
    \centering
    \begin{tabular}{ccc}
    \includegraphics[width=0.3\linewidth]{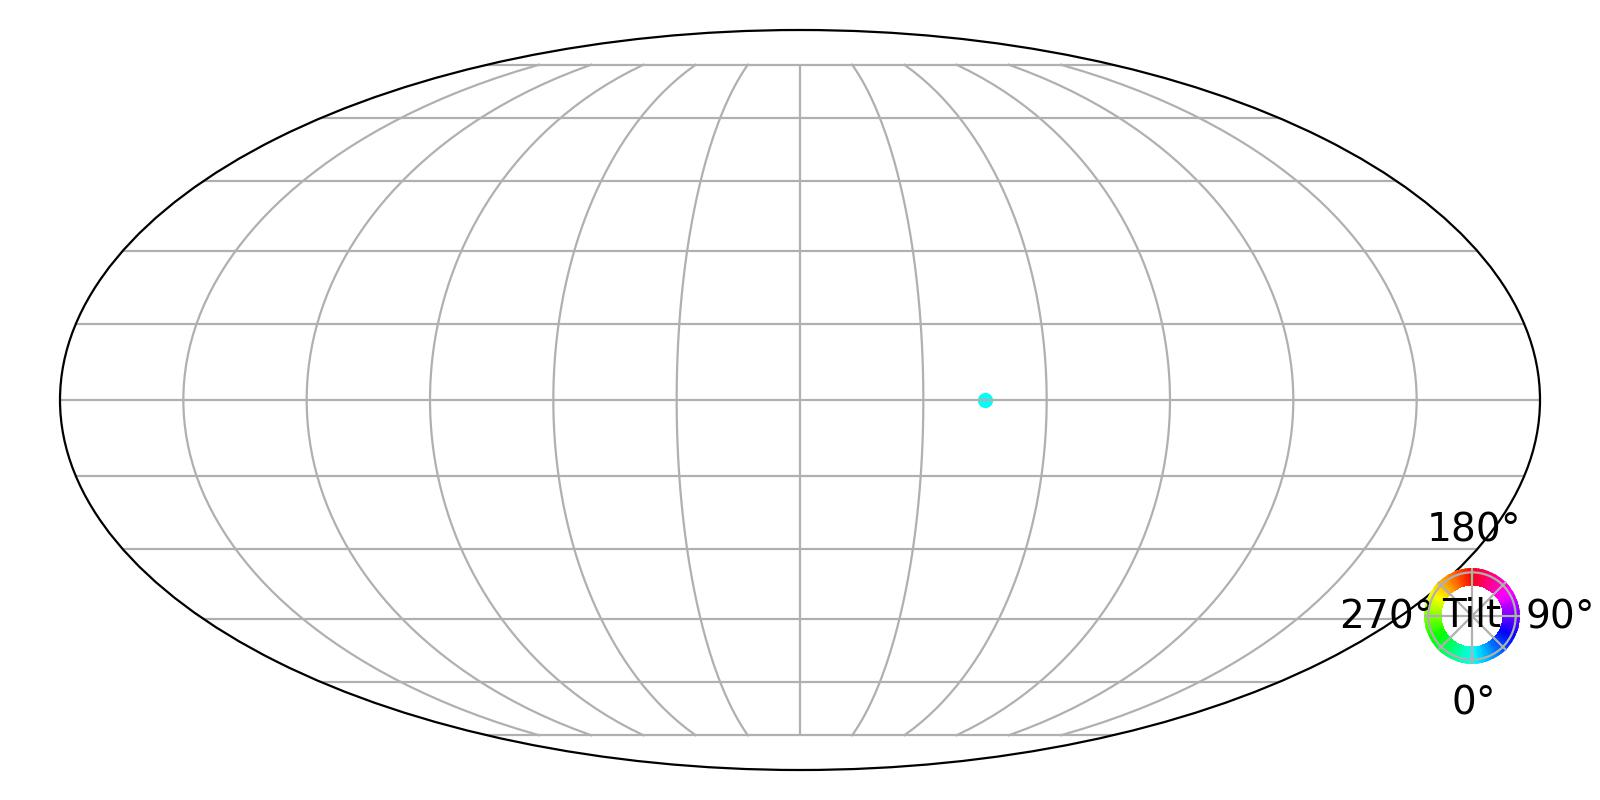}
    &\includegraphics[width=0.3\linewidth]{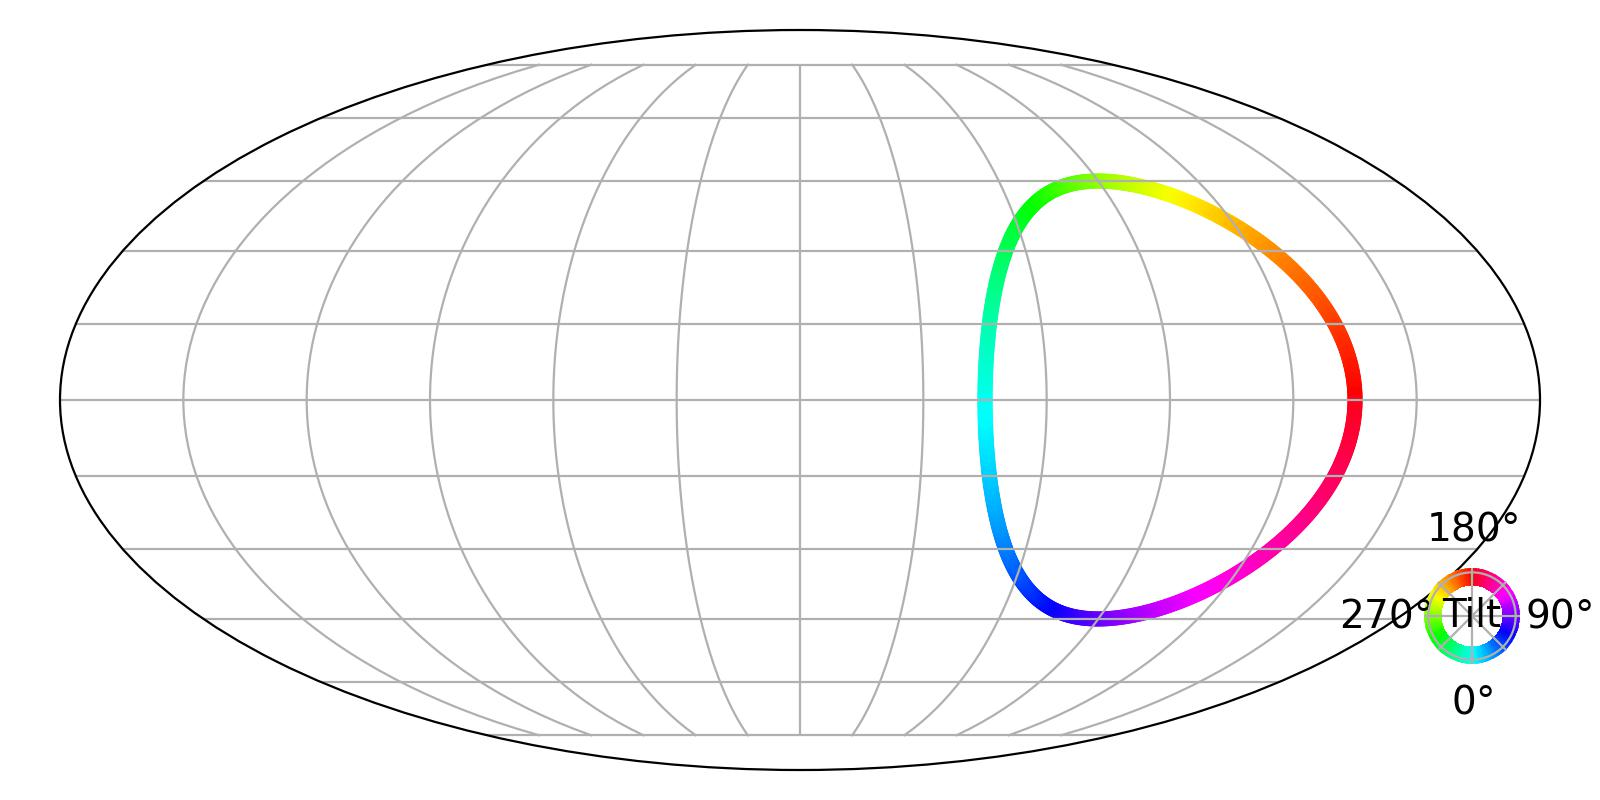}
    &\includegraphics[width=0.3\linewidth]{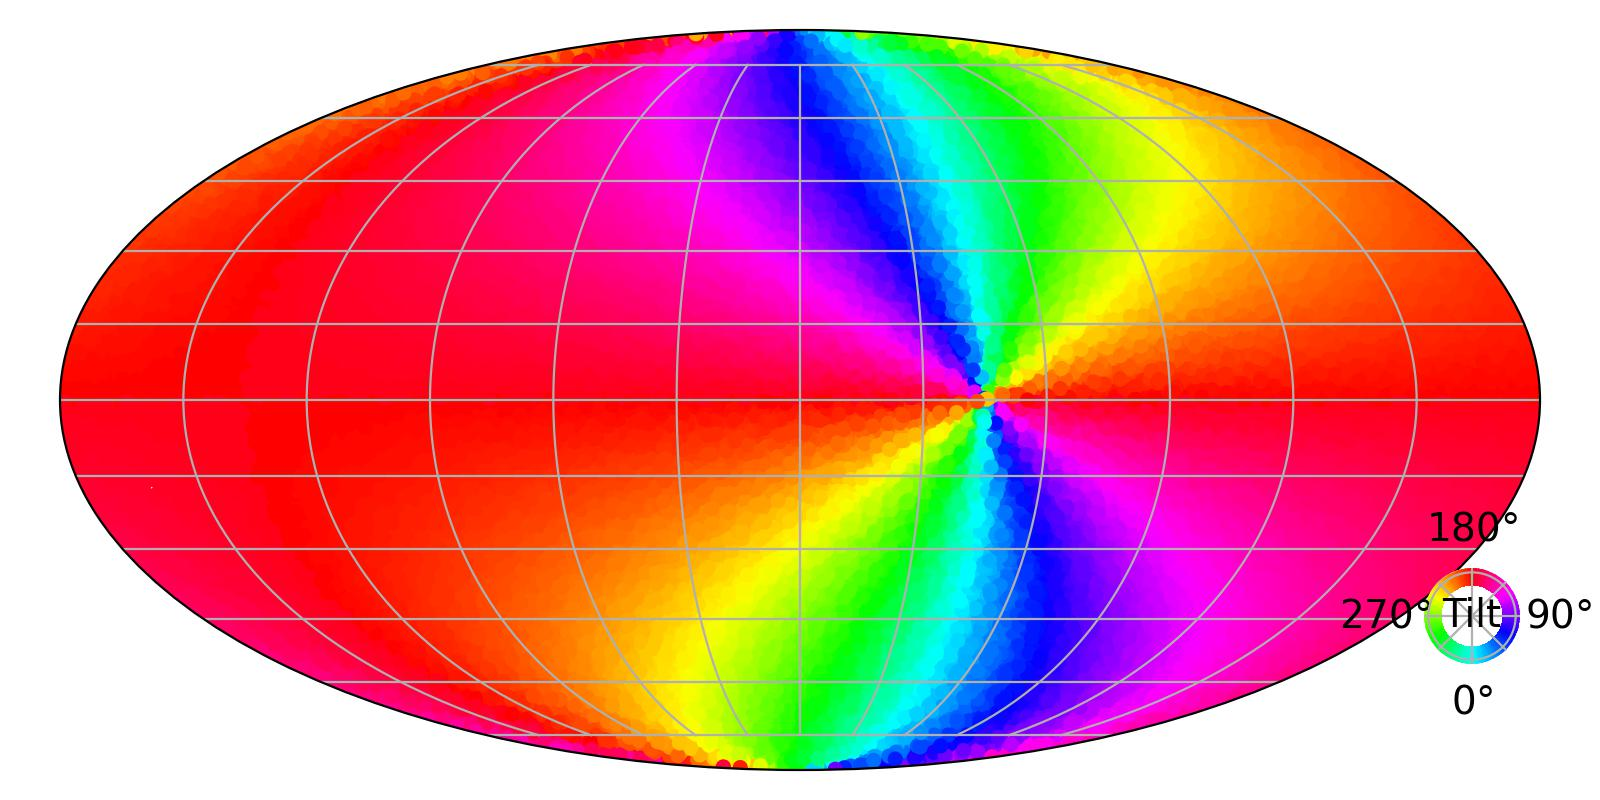}
    \\
    \small{case1: $\mathbf{A}=\operatorname{diag}(1, 1, 1)$} &
    \small{case2: $\mathbf{A}=\operatorname{diag}(1, 0, 0)$} &
    \small{case3: $\mathbf{A}=\operatorname{diag}(1, 1, -1)$}
    \\    
    \end{tabular}
    \caption{\small \textbf{Visualization of the modes of rotation Laplace distribution with different parameters.} We use the visualization method in \cite{murphy2021implicit}.}
    \label{fig:unique_vis}
\end{figure*}

% \todo{Fisher also has the same problem.}

\begin{proof}
    For rotation Laplace distribution
    \begin{equation}
    \footnotesize
    \begin{aligned}
        p(\mathbf{R}; \mathbf{A}) 
        &= \frac{1}{F(\mathbf{A})} \frac{\exp\left(-\sqrt{\operatorname{tr}\left(\mathbf{S} - \mathbf{A}^T \mathbf{R}\right)}\right)}
        {\sqrt{\operatorname{tr}\left(\mathbf{S} -\mathbf{A}^T \mathbf{R}\right)}} \\ 
        & = \frac{1}{F(\mathbf{A})} \frac{\exp\left(-\sqrt{\operatorname{tr}(\mathbf{S}-\mathbf{S}\mathbf{U}^T\mathbf{R}\mathbf{V})}\right)}{\sqrt{\operatorname{tr}(\mathbf{S}-\mathbf{S}\mathbf{U}^T\mathbf{R}\mathbf{V})}} \\
        & \xlongequal{\mathbf{R}'=\mathbf{U}^T\mathbf{R}\mathbf{V}}  \frac{1}{F(\mathbf{A})} \frac{\exp\left(-\sqrt{\operatorname{tr}\left(\mathbf{S} - \mathbf{S}\mathbf{R}'\right)}\right)}
        {\sqrt{\operatorname{tr}\left(\mathbf{S} -\mathbf{S}\mathbf{R}'\right)}} 
    \end{aligned}
    \end{equation}

    Below we first consider the mode of  $\mathbf{R}'$, denoted as ${\mathbf{R}_0}'$, and then the mode of $\mathbf{R}$ is given as
    \begin{equation}
        {\mathbf{R}_0} = \mathbf{U}{\mathbf{R}}_0'\mathbf{V}^T
        \label{eq:rprime}
    \end{equation}

    % We consider the simple case when $\mathbf{A}=\mathbf{S}$. Otherwise, we apply a transformation $\mathbf{R}'=\mathbf{V}^T\mathbf{R}\mathbf{U}$, such that the distribution follows the simple case.
    
    % Given $\mathbf{R}'=\mathbf{U}^T\mathbf{R}\mathbf{V}$, and c
    Considering the transformation $\gamma$ between rotation matrix and unit quaternion
    \begin{equation}
    \footnotesize
        \mathbf{R}' = \gamma(\mathbf{q'}) = \begin{pmatrix} 1-2y^2-2z^2 & 2xy-2zw & 2xz+2yw \\ 2xy+2zw & 1-2x^2-2z^2 & 2yz-2xw \\ 2xz-2yw & 2yz+2xw & 1-2x^2-2y^2 \end{pmatrix},
    \label{eq:r_to_q}
    \end{equation}
    we have 
    % $\mathbf{R}'=\gamma(w, x, y, z)$, then
    \begin{equation}
    \footnotesize
        p(w,x,y,z;\mathbf{A}) = \frac{1}{F(\mathbf{A})} \frac{\exp\left(
        -\sqrt{2(s_2+s_3) x^2 + 2(s_1+s_3) y^2 + 2(s_1+s_2)z^2}
        \right)}{\sqrt{2(s_2+s_3) x^2 + 2(s_1+s_3) y^2 + 2(s_1+s_2)z^2}}
        \label{eq:pdf_q}
    \end{equation}

    Therefore, $p(w,x,y,z)$ monotonically decreases wrt.
    $2(s_2 + s_3)x^2 + 2(s_1 + s_3)y^2 + 2(s_1 + s_2)z^2$.
    % Since $2(s_2 + s_3)x^2 + 2(s_1 + s_3)y^2 + 2(s_1 + s_2)z^2 \ge 0$, 
    Since
    \begin{equation}
        s_1 + s_2 \ge s_1 + s_3 \ge s_2 + s_3 \ge 0,
        \label{eq:property_svd}
    \end{equation}
    we have 
    \begin{equation}
    \begin{aligned}
         &\mathbf{R}' \text{ is mode } &\\
        \Leftrightarrow 
         (s_2 + s_3)x^2 = 0  \text{ and } & (s_1 + s_3)y^2 = 0 \text{ and } (s_1 + s_2)z^2 = 0        
    \end{aligned}
    \end{equation}

    We discuss the values of $s_1 + s_2, s_1 + s_3, s_2 + s_3$ to determine the mode of the distribution.
    
    \begin{itemize}
    \item \textbf{Case 1: } $s_2+s_3>0$ \\
    According to Eq. \ref{eq:property_svd},
    \begin{equation}
    \begin{aligned}
        & \mathbf{R}' \text{ is mode } 
        \Leftrightarrow 
         x = 0 \text{ and } y = 0 \text{ and } z = 0        
    \end{aligned}
    \end{equation}
    Therefore, ${\mathbf{R}_0}' = \mathbf{I}$ is the unique mode for $\mathbf{R}'$, and ${\mathbf{R}_0} = \mathbf{U}\mathbf{V}^T$ is the unique mode for $\mathbf{R}$.
    
    \item \textbf{Case 2: } $s_2+s_3=0$, but $s_1+s_3>0$ \\
    We have
    \begin{equation}
    \begin{aligned}
        & \mathbf{R}' \text{ is mode } 
        \Leftrightarrow 
         y = 0 \text{ and } z = 0        
    \end{aligned}
    \end{equation}
    Therefore, given Eq. \ref{eq:r_to_q}, the modes of $\mathbf{R}'$ are 
    \begin{equation}
    \footnotesize
        \begin{pmatrix} 1 & 0 & 0 \\ 0 & 1-2x^2 & -2xw \\ 0 & 2xw & 1-2x^2 \end{pmatrix},
    \end{equation}
    and the modes of $\mathbf{R}$ have the form of 
    \begin{equation}
    \footnotesize
        \mathbf{U} \begin{pmatrix} 1 & 0 & 0 \\ 0 & 1-2x^2 & -2xw \\ 0 & 2xw & 1-2x^2 \end{pmatrix} \mathbf{V}^T,
    \end{equation}

    \item \textbf{Case 3: } $s_2+s_3=0$, $s_1+s_3=0$, but $s_1+s_2>0$ \\
    We have
    \begin{equation}
    \begin{aligned}
        & \mathbf{R}' \text{ is mode } 
        \Leftrightarrow 
         z = 0        
    \end{aligned}
    \end{equation}

    Therefore, given Eq. \ref{eq:r_to_q}, the modes of $\mathbf{R}'$ are 
    \begin{equation}
    \footnotesize
        \begin{pmatrix} 1-2y^2 & 2xy & 2yw \\ 2xy & 1-2x^2 & -2xw \\ -2yw & 2xw & 1-2x^2-2y^2 \end{pmatrix},
    \end{equation}
    and the modes of $\mathbf{R}$ have the form of 
    \begin{equation}
    \footnotesize
        \mathbf{U} \begin{pmatrix} 1-2y^2 & 2xy & 2yw \\ 2xy & 1-2x^2 & -2xw \\ -2yw & 2xw & 1-2x^2-2y^2 \end{pmatrix}\mathbf{V}^T,
    \end{equation}

    \item \textbf{Case 4: } $s_2+s_3=0$, $s_1+s_3=0$, $s_1+s_2=0$
    
    We have $s_1=s_2=s_3=0$, therefore, the denominator of $p(w,x,y,z)$ is zero for all $(w,x,y,z)$ and the distribution is ill-defined.
    
    \end{itemize}

\end{proof}
