# Supplementary material for: Towards Robust Probabilistic Modeling on SO(3) via Rotation Laplace Distribution
Source: arXiv:2305.10465 source file (2025-02-21)
Supplement: Supplementary file 5 [file normalization_constant.tex]

% \todo{we have verified the equations by sampling?}
\textbf{Normalization Constant.}
We firstly show that the normalization factor depends only on $\mathbf{S}$.
\begin{proof}
\begin{equation}
\footnotesize
\begin{aligned}
    F(\mathbf{A}) 
    &= \int_{\SO} \frac{\exp\left(-\sqrt{\operatorname{tr}\left(\mathbf{S} - \mathbf{A}^T \mathbf{R}\right)}\right)}
    {\sqrt{\operatorname{tr}\left(\mathbf{S} -\mathbf{A}^T \mathbf{R}\right)}} \mathrm{d}\mathbf{R}\\ 
    & = \int_{\SO} \frac{\exp\left(-\sqrt{\operatorname{tr}(\mathbf{S}-\mathbf{S}\mathbf{U}^T\mathbf{R}\mathbf{V})}\right)}{\sqrt{\operatorname{tr}(\mathbf{S}-\mathbf{S}\mathbf{U}^T\mathbf{R}\mathbf{V})}} \mathrm{d}\mathbf{R} \\
    & \xlongequal{\mathbf{R}'=\mathbf{U}^T\mathbf{R}\mathbf{V}}  \int_{\SO} \frac{\exp\left(-\sqrt{\operatorname{tr}\left(\mathbf{S} - \mathbf{S}\mathbf{R}'\right)}\right)}
    {\sqrt{\operatorname{tr}\left(\mathbf{S} -\mathbf{S}\mathbf{R}'\right)}} \mathrm{d}\mathbf{R}'\
\end{aligned}
\end{equation}
\end{proof}

We then try to derive analytical expression of the normalization factor. We have verified our solutions by comparing with numerical results via discretization.

We denote $s_1, s_2, s_3$ as the singular values of $\mathbf{A}$.
Considering the transformation between rotation matrix and unit quaternion
    \begin{equation}
    \footnotesize
        \mathbf{R}' = \gamma(\mathbf{q}) = \begin{pmatrix} 1-2y^2-2z^2 & 2xy-2zw & 2xz+2yw \\ 2xy+2zw & 1-2x^2-2z^2 & 2yz-2xw \\ 2xz-2yw & 2yz+2xw & 1-2x^2-2y^2 \end{pmatrix},
    \label{eq:r_to_q}
    \end{equation}
we define 
% $t_1=2(s_2+s_3)$, $t_2=2(s_3+s_1)$, $t_3=2(s_1+s_2)$ and $k=t_1x_0^2+t_2y_0^2+t_3z_0^2$
\begin{equation}
    \footnotesize
    \begin{aligned}
        t_1&=2(s_2+s_3) \\
        t_2&=2(s_3+s_1) \\
        t_3&=2(s_1+s_2) \\
        %k&=t_1x_0^2+t_2y_0^2+t_3z_0^2 \\
    \end{aligned}
    \label{eq:t123}
\end{equation}
the normalizing factor can be expressed as a one-dimensional integration:
    \begin{equation}
    \footnotesize
    \begin{aligned}
        F(\mathbf{A})=&\frac{2}{\pi}\left(\int_{t_1}^{t_2}\frac{\left(\mathbf{L}_{-1}(\sqrt{k})-\mathbf{I}_{1}(\sqrt{k})\right)\mathbf{K}\left(\frac{(k-t_1)(t_3-t_2)}{(t_1-t_2)(k-t_3)}\right)}{\sqrt{k(t_2-t_1)(t_3-k)}}\mathrm{d}k \right.\\
        &\left.+ \int_{t_2}^{t_3}\frac{\left(\mathbf{L}_{-1}(\sqrt{k})-\mathbf{I}_{1}(\sqrt{k})\right)\mathbf{K}\left(\frac{(k-t_3)(t_1-t_2)}{(t_3-t_2)(k-t_1)}\right)}{\sqrt{k(t_2-t_3)(t_1-k)}}\mathrm{d}k\right)
    \end{aligned}
    \end{equation}
where $\mathbf{L}$ is the modified Struve function, $\mathbf{I}$ is the modified Bessel function of the first kind, and $\mathbf{K}$ is the complete elliptic integral of the first kind.

Specifically, when $s_1 = s_2 = s_3 = s$, it can be simplified as 
\begin{equation}
\footnotesize
    F(\mathbf{A})=\frac{\mathbf{L}_{-1}(2\sqrt{s})-\mathbf{I}_1(2\sqrt{s})}{\sqrt{s}}
\end{equation}
%where $_0\tilde{\mathbf{F}}_1$ is regularized confluent hypergeometric function.

\begin{proof}
    Given $\mathbf{R}'=\mathbf{U}^T\mathbf{R}\mathbf{V}$, and considering Eq. \ref{eq:r_to_q}
    we have
    \begin{equation}
    \footnotesize
        \operatorname{tr}(\mathbf{S}-\mathbf{S}\mathbf{R}')=2(s_2+s_3)x^2+2(s_1+s_3)y^2+2(s_1+s_2)z^2
    \end{equation}
    Define $\theta$ as the rotation angle, and then the quaternion $(w,x,y,z)$ can be expressed as 
    \begin{equation}
        \footnotesize
        (w,x,y,z) = (\cos\theta, \sin\theta x_0, \sin\theta y_0, \sin\theta z_0)
    \end{equation}
    satisfying $x_0^2+y_0^2+z_0^2=1$. Thus we can first integrate over $\theta$, then integrate over $a=(x_0, y_0, z_0)\in\mathcal{S}^2$.
    Considering Eq. \ref{eq:t123}, we have
    \begin{equation}
    \scriptsize
    \begin{aligned}
        &F(\mathbf{A})\\
        =&\frac{1}{2\pi^2}\int_{\SO} \frac{\exp\left(-\sqrt{2(s_2+s_3)x^2+2(s_1+s_3)y^2+2(s_1+s_2)z^2}\right)}{\sqrt{2(s_2+s_3)x^2+2(s_1+s_3)y^2+2(s_1+s_2)z^2}} \\
        =&\frac{1}{2\pi^2}\int_{\SO}\frac{\exp\left(-\sin{\theta}\sqrt{2(s_2+s_3)x_0^2+2(s_1+s_3)y_0^2+2(s_1+s_2)z_0^2}\right)}{\sin{\theta}\sqrt{2(s_2+s_3)x_0^2+2(s_1+s_3)y_0^2+2(s_1+s_2)z_0^2}} \\
    \end{aligned}
    \end{equation}
    By defining
    \begin{equation}
    \footnotesize
        k=t_1x_0^2+t_2y_0^2+t_3z_0^2
    \end{equation}
    we have
    \begin{equation}
    \footnotesize
    \begin{aligned}
        F(\mathbf{A})&=\frac{1}{2\pi^2}\int_{\SO}\frac{\exp\left(-\sqrt{k}\sin{\theta}\right)}{\sqrt{k}\sin{\theta}} \\
        =&\frac{1}{2\pi^2}\int_{\mathcal{S}^2} \frac{1}{\sqrt{k}} \int_{0}^{\pi} \sin{\theta}\exp\left(-\sqrt{k}\sin{\theta}\right) \mathrm{d}\theta \mathrm{d}a \\
        =&\frac{1}{2\pi}\int_{\mathcal{S}^2} \frac{\mathbf{L}{-1}(\sqrt{k})-\mathbf{I}_{1}(\sqrt{k})}{\sqrt{k}} \mathrm{d}a \\
        =&\frac{1}{2\pi}\left(\int_{t_1}^{t_2}S_1(k)\frac{\mathbf{L}_{-1}(\sqrt{k})-\mathbf{I}_{1}(\sqrt{k})}{\sqrt{k}}\mathrm{d}k\right.\\
        &\left.+\int_{t_2}^{t_3}S_2(k)\frac{\mathbf{L}_{-1}(\sqrt{k})-\mathbf{I}_{1}(\sqrt{k})}{\sqrt{k}}\mathrm{d}k\right)
    \end{aligned}
    \label{eq:f_to_s}
    \end{equation}
where $S_1(k)$  is computed as 
    \begin{equation}
    \footnotesize
    \begin{aligned}
        S_1(k)&=\int_0^{\sqrt{\frac{k-t_1}{t_2-t_1}}}\frac{4}{(t_3-t_1)xz}\mathrm{d}y \\
        &= \int_0^{\sqrt{\frac{k-t_1}{t_2-t_1}}}\frac{4}{\sqrt{k-t_1+t_1y^2-t_2y^2}\sqrt{-k+t_3-t_3y^2+t_2y^2}}\mathrm{d}y \\
        &=  \frac{4\mathbf{K}(\frac{(k-t_1)(t_3-t_2)}{(t_1-t_2)(k-t_3)})}{\sqrt{(t_2-t_1)(t_3-k)}} 
    \end{aligned}
    \label{eq:s1}
    \end{equation}
    Similarily, we have 
    \begin{equation}
    \footnotesize
    \begin{aligned}
        S_2(k)&=\frac{4\mathbf{K}(\frac{(k-t_3)(t_1-t_2)}{(t_3-t_2)(k-t_1)})}{\sqrt{(t_2-t_3)(t_1-k)}}
    \end{aligned}
    \label{eq:s2}
    \end{equation}
    Combining Eq. \ref{eq:f_to_s}, Eq. \ref{eq:s1}, and \ref{eq:s2} together, we have
        \begin{equation}
    \footnotesize
    \begin{aligned}
        F(\mathbf{A})=&\frac{2}{\pi}\left(\int_{t_1}^{t_2}\frac{\left(\mathbf{L}_{-1}(\sqrt{k})-\mathbf{I}_{1}(\sqrt{k})\right)\mathbf{K}\left(\frac{(k-t_1)(t_3-t_2)}{(t_1-t_2)(k-t_3)}\right)}{\sqrt{k(t_2-t_1)(t_3-k)}}\mathrm{d}k \right.\\
        &\left.+ \int_{t_2}^{t_3}\frac{\left(\mathbf{L}_{-1}(\sqrt{k})-\mathbf{I}_{1}(\sqrt{k})\right)\mathbf{K}\left(\frac{(k-t_3)(t_1-t_2)}{(t_3-t_2)(k-t_1)}\right)}{\sqrt{k(t_2-t_3)(t_1-k)}}\mathrm{d}k\right)
    \end{aligned}
    \end{equation}

Specifically, when $s_1=s_2=s_3=s$, 
\begin{equation}
    \footnotesize
    \begin{aligned}
        t_1&=2(s_2+s_3)=4s \\
        t_2&=2(s_3+s_1)=4s \\
        t_3&=2(s_1+s_2)=4s \\
        k&=t_1x_0^2+t_2y_0^2+t_3z_0^2=4s(x_0^2+y_0^2+z_0^2)=4s \\
    \end{aligned}
\end{equation}
    Thus with Eq. \ref{eq:f_to_s} we have,
    \begin{equation}
    \footnotesize
    \begin{aligned}
        F(\mathbf{A})&=\frac{1}{2\pi}\int_{\mathcal{S}^2} \frac{\mathbf{L}{-1}(\sqrt{k})-\mathbf{I}_{1}(\sqrt{k})}{\sqrt{k}} \mathrm{d}a \\
        &=\frac{1}{4\pi}\int_{\mathcal{S}^2} \frac{\mathbf{L}_{-1}(2\sqrt{s})-\mathbf{I}_{1}(2\sqrt{s})}{\sqrt{s}} \mathrm{d}a \\
        &=\frac{\mathbf{L}_{-1}(2\sqrt{s})-\mathbf{I}_1(2\sqrt{s})}{\sqrt{s}}
    \end{aligned}
    \end{equation}
\end{proof}
