# Supplementary material for: Towards Robust Probabilistic Modeling on SO(3) via Rotation Laplace Distribution
Source: arXiv:2305.10465 source file (2025-02-21)
Supplement: Supplementary file 6 [file proof_fisher.tex]

\begin{prop1}
    Let $\boldsymbol{\Phi} = \log \mathbf{\widetilde{R}} \in \mathfrak{so}(3)$ and $\boldsymbol{\phi} = {\boldsymbol{\Phi}^\vee} \in \mathbb{R}^3$. For rotation matrix $\mathbf{R} \in \SO$ following \emph{matrix Fisher distribution}, when 
    % $\mathbf{R}\rightarrow \mathbf{R}_0$
    \ree{$\|\mathbf{R} - \mathbf{R}_0 \| \rightarrow 0$}
    , $\boldsymbol{\phi}$ follows zero-mean \emph{multivariate Gaussian distribution}.
\end{prop1}
\begin{proof}
For $\mathbf{R}\sim \mathcal{MF}(\mathbf{A})$, we have
\begin{equation}
% \label{eq:prdr}
\footnotesize
\begin{aligned}
    p(\mathbf{R})\mathrm{d}\mathbf{R} &\propto \exp\left(\tr{\mathbf{A}^T\mathbf{R}}\right)\mathrm{d}\mathbf{R}   
    % =\exp(\tr{\mathbf{VSU^T}\mathbf{\hat{\mathbf{R}}\widetilde{R}}})\mathrm{d}\mathbf{\widetilde{R}}
    = \exp\left(\tr{\mathbf{S}\mathbf{V}^T\mathbf{\widetilde{R}}\mathbf{V}}\right)\mathrm{d}\mathbf{\widetilde{R}}
\end{aligned}
\end{equation}
Considering Eq.5 in the main paper, we have
\begin{equation}
\label{eq:tr}
\footnotesize
\begin{aligned}
    \tr{\mathbf{S}\mathbf{V}^T\mathbf{\widetilde{R}}\mathbf{V}} 
    &= \tr{\mathbf{S}} + \sum_{(i,j,k)\in I}-\frac{1}{2}(s_j+s_k)\mu_i^2+O({\len {\boldsymbol{\phi}}}^3) \\
    &=\tr{\mathbf{S}} -\frac{1}{2}\boldsymbol{\phi}^T\mathbf{V}
    % \operatorname{diag}(s_2+s_3,s_3+s_1,s_1+s_2)
    \left[\begin{smallmatrix}
        s_2 + s_3 &  &  \\
        & s_1 + s_3 &  \\
        &  & s_1 + s_2
        \end{smallmatrix}\right]
    \mathbf{V}^T\boldsymbol{\phi}
\end{aligned}
\end{equation}
Thus
\begin{equation}
\footnotesize
\label{eq:gauss}
\begin{aligned}
    p(\mathbf{R})\mathrm{d}\mathbf{R} &\propto \exp\left(\tr{\mathbf{A}^T\mathbf{R}}\right)\mathrm{d}\mathbf{R}\\  
    % = \left(\frac{1}{8\pi^2}+O({\len {\boldsymbol{\phi}}}^2)\right)\exp\left(\tr{\mathbf{S}}\right)\exp\left(\sum_{(i,j,k)\in I}-\frac{1}{2}(s_j+s_k)\mu_i^2+O({\len {\boldsymbol{\phi}}}^3)\right)\mathrm{d}\boldsymbol{\phi} \\
    % % &= (\frac{1}{8\pi^2}\exp(\tr{S})\exp(-\frac{1}{2}(\mathbf{V}^T\boldsymbol{\phi})^T\operatorname{diag}(s_2+s_3,s_3+s_1,s_1+s_2)(\mathbf{V}^T\boldsymbol{\phi}) + O({\len {\boldsymbol{\phi}}}^2))d\boldsymbol{\phi} \\
    % &= \frac{1}{8\pi^2}
    % \exp(\tr{S})
    % \exp\left(-\frac{1}{2}\boldsymbol{\phi}^T\mathbf{V}
    % % \operatorname{diag}(s_2+s_3,s_3+s_1,s_1+s_2)
    % \left[\begin{smallmatrix}
    %     s_2 + s_3 &  &  \\
    %     & s_1 + s_3 &  \\
    %     &  & s_1 + s_2
    %     \end{smallmatrix}\right]
    % \mathbf{V}^T\boldsymbol{\phi}\right)+ O({\len {\boldsymbol{\phi}}}^2)\mathrm{d}\boldsymbol{\phi} \\
    &= \frac{\exp(\tr{\mathbf{S}})}{8\pi^2}\exp\left(-\frac{1}{2}\boldsymbol{\phi}^T\boldsymbol{\Sigma} ^{-1}\boldsymbol{\phi}\right) \left(1 + O({\len {\boldsymbol{\phi}}}^2)\right)\mathrm{d}\boldsymbol{\phi}
\end{aligned}
\end{equation}
When 
% $\mathbf{R}\rightarrow \mathbf{R}_0$
\ree{$\|\mathbf{R} - \mathbf{R}_0\| \rightarrow 0$}
, we have 
% $\mathbf{\widetilde{R}} \rightarrow \mathbf{I}$ 
\ree{$\|\mathbf{\widetilde{R}} - \mathbf{I}\|  \rightarrow 0$ }
and $\boldsymbol{\phi} \rightarrow \mathbf{0}$, so Eq. \ref{eq:gauss} follows the multivariate Gaussian distribution 
with the covariance matrix as $\boldsymbol{\Sigma}$, where $\boldsymbol{\Sigma} = \mathbf{V}\operatorname{diag}(\frac{1}{s_2+s_3},\frac{1}{s_1+s_3},\frac{1}{s_1+s_2})\mathbf{V}^T$.
\end{proof}
