# Supplementary material for: Towards Robust Probabilistic Modeling on SO(3) via Rotation Laplace Distribution
Source: arXiv:2305.10465 source file (2025-02-21)
Supplement: Supplementary file 7 [file proof_laplace.tex]

\begin{prop2}
Let $\boldsymbol{\Phi} = \log \mathbf{\widetilde{R}} \in \mathfrak{so}(3)$ and $\boldsymbol{\phi} = {\boldsymbol{\Phi}^\vee} \in \mathbb{R}^3$. For rotation matrix $\mathbf{R} \in \SO$ following \emph{rotation Laplace distribution}, when
% $\mathbf{R}\rightarrow \mathbf{R}_0$
\ree{$\|\mathbf{R} - \mathbf{R}_0\|\rightarrow 0$}
, $\boldsymbol{\phi}$ follows zero-mean \emph{multivariate Laplace distribution}.

\end{prop2}
\begin{proof}

Apply proper SVD to matrix $\mathbf{A}$ as $\mathbf{A} = \mathbf{USV}^T$.
For $\mathbf{R}\sim \mathcal{RL}(\mathbf{A})$ , we have
\begin{equation}
\label{eq:prdr}
\scriptsize
\begin{aligned}
    p(\mathbf{R})\mathrm{d}\mathbf{R} &\propto 
    \frac{\exp\left(-\sqrt{\tr{\mathbf{S}-{\mathbf{A}^T\mathbf{R}}}}\right)}{\sqrt{\tr{\mathbf{S}-{\mathbf{A}^T\mathbf{R}}}}} \mathrm{d}\mathbf{R}
    = \frac{\exp\left(-\sqrt{\operatorname{tr}(\mathbf{S}-\mathbf{V}\mathbf{S}\mathbf{U}^T\mathbf{R})}\right)}{\sqrt{\operatorname{tr}(\mathbf{S}-\mathbf{V}\mathbf{S}\mathbf{U}^T\mathbf{R})}} \mathrm{d}\mathbf{R} \\
 &= \frac{\exp\left(-\sqrt{\operatorname{tr}(\mathbf{S}-\mathbf{S}\mathbf{U}^T\mathbf{R}\mathbf{V})}\right)}{\sqrt{\operatorname{tr}(\mathbf{S}-\mathbf{S}\mathbf{U}^T\mathbf{R}\mathbf{V})}} \mathrm{d}\mathbf{R} \\
    &= \frac{\exp\left(-\sqrt{\tr{\mathbf{S}-\mathbf{S}\mathbf{V}^T\mathbf{\widetilde{R}}\mathbf{V}}}\right)}{\sqrt{\tr{\mathbf{S}-\mathbf{S}\mathbf{V}^T\mathbf{\widetilde{R}}\mathbf{V}}}} \mathrm{d}\mathbf{R}
\end{aligned}
\end{equation}

% \jiangran{\input{sections_supp/elaboration.tex}}

With $\boldsymbol{\phi}  = (\log{\mathbf{\widetilde{R}}})^\vee \in \mathbb{R}^3$,
$\mathbf{\widetilde{R}}$ can be parameterized as 
{\footnotesize\begin{equation*}
    \mathbf{\widetilde{R}}(\boldsymbol{\phi} )= 
    \exp(\hat{\boldsymbol{\phi}}) = 
    \mathbf{I}+\frac{\sin\len {\boldsymbol{\phi}}  }{\len {\boldsymbol{\phi}}}\hat{\boldsymbol{\phi}}
    + \frac{1-\cos\len {\boldsymbol{\phi}}}{{\len {\boldsymbol{\phi}}}^2}{\hat{\boldsymbol{\phi}}}^2
\end{equation*}
}\ree{We follow the common practice \cite{mohlin2020probabilistic,lee2018bayesian} that the Haar measure $\mathrm{d}\mathbf{R}$ is scaled such that $\int_{SO(3)} \mathrm{d} \mathbf{R}=1$} and thus the Haar measure is given by
% and the Haar measure \ree{\cite{mohlin2020probabilistic,lee2018bayesian} is given by}
\begin{equation}
\footnotesize
\label{eq:d_rwave}
    \mathrm{d}\mathbf{\widetilde{R}} 
    = \frac{1- \cos \len {\boldsymbol{\phi}}}{{4\pi^2 \len {\boldsymbol{\phi}}}^2}\mathrm{d}\boldsymbol{\phi}
    = \left(\frac{1}{8\pi^2}+O(\len {\boldsymbol{\phi}})^2\right)\mathrm{d}\boldsymbol{\phi}.
\end{equation}
Also, $\mathbf{\widetilde{R}}$ expanded at $\boldsymbol{\phi}=\mathbf{0}$ is computed as 
{\small$\mathbf{\widetilde{R}} = \mathbf{I}+\hat{\boldsymbol{\phi}}+\frac{1}{2}\hat{\boldsymbol{\phi}}^2+O({\len {\boldsymbol{\phi}} }^3)$},
% {\scriptsize\begin{equation*}
%     \mathbf{\widetilde{R}} = \mathbf{I}+\hat{\boldsymbol{\phi}}+\frac{1}{2}\hat{\boldsymbol{\phi}}^2+O({\len {\boldsymbol{\phi}} }^3)\\ 
% \end{equation*}}
we have 
\begin{equation}
\label{eq:vtrv}
\scriptsize
\begin{aligned}
    \mathbf{V}^T\mathbf{\widetilde{R}}\mathbf{V} &= \mathbf{I} + \mathbf{V}^T\hat{\boldsymbol{\phi}}\mathbf{V} + \frac{1}{2}\mathbf{V}^T\hat{\boldsymbol{\phi}}^2\mathbf{V}+O(\len{\boldsymbol{\phi}}^3)\\
    &= \mathbf{I}+\widehat{\mathbf{V}^T\boldsymbol{\phi}}+\frac{1}{2}\widehat{\mathbf{V}^T\boldsymbol{\phi}}^2+O({\len {\boldsymbol{\phi}} }^3)\\
    &= \left[\begin{array}{ccc}
        1-\frac{1}{2}(\mu_2^2+\mu_3^2) & \frac{1}{2}{\mu_1}{\mu_2}-\mu_3 & \frac{1}{2}{\mu_1}{\mu_3}+\mu_2 \\
        \frac{1}{2}{\mu_1}{\mu_2}+\mu_3 & 1-\frac{1}{2}(\mu_3^2+\mu_1^2) & \frac{1}{2}{\mu_2}{\mu_3}-\mu_1 \\
        \frac{1}{2}{\mu_1}{\mu_3}-\mu_2 & \frac{1}{2}{\mu_2}{\mu_3}+\mu_1 & 1-\frac{1}{2}(\mu_1^2+\mu_2^2)
        \end{array}\right] \\ &+ O({\len {\boldsymbol{\phi}}}^3), 
\end{aligned}
\end{equation}
where $(\mu_1,\mu_2,\mu_3)^T = \mathbf{V}^T\boldsymbol{\phi}$, 
and
\begin{equation}
\label{eq:tr_laplace}
\footnotesize
\begin{aligned}
    \tr{\mathbf{S}-\mathbf{S}\mathbf{V}^T\mathbf{\widetilde{R}}\mathbf{V}} 
    &=\sum_{(i,j,k)\in I}\frac{1}{2}(s_j+s_k)\mu_i^2+O({\len {\boldsymbol{\phi}}}^3)\\ 
    % &=\frac{1}{2}(\mathbf{V}^T\phi)^T\operatorname{diag}(s_2+s_3,s_3+s_1,s_1+s_2)(\mathbf{V}^T\phi))+O({\len {\boldsymbol{\phi}}}^3) \\
    &=\frac{1}{2}\boldsymbol{\phi}^T\mathbf{V}
    % \operatorname{diag}(s_2+s_3,s_3+s_1,s_1+s_2)
    \left[\begin{smallmatrix}
        s_2 + s_3 &  &  \\
        & s_1 + s_3 &  \\
        &  & s_1 + s_2
        \end{smallmatrix}\right]
    \mathbf{V}^T\boldsymbol{\phi}+O({\len {\boldsymbol{\phi}}}^3)
\end{aligned}
\end{equation}
Considering Eq. \ref{eq:prdr}, \ref{eq:d_rwave} and \ref{eq:tr_laplace}, we have
\begin{equation}
\label{eq:laplace}
\footnotesize
\begin{aligned}
    p(\mathbf{R})\mathrm{d}\mathbf{R} &\propto \frac{\exp\left(-\sqrt{\tr{\mathbf{S}-{\mathbf{A}^T\mathbf{R}}}}\right)}{\sqrt{\tr{\mathbf{S}-{\mathbf{A}^T\mathbf{R}}}}} \mathrm{d}\mathbf{R}\\
    % = (\frac{1}{8\pi^2} + O({\len {\boldsymbol{\phi}}}^2))\frac{\exp(-\sqrt{\frac{1}{2}
    % \boldsymbol{\phi}^T\mathbf{V}
    % % \operatorname{diag}(s_2+s_3,s_3+s_1,s_1+s_2)
    % \left[\begin{smallmatrix}
    %     s_2 + s_3 &  &  \\
    %     & s_1 + s_3 &  \\
    %     &  & s_1 + s_2
    %     \end{smallmatrix}\right]
    % \mathbf{V}^T\boldsymbol{\phi}
    % +O({\len {\boldsymbol{\phi}}}^3)})}{\sqrt{\frac{1}{2}
    % \boldsymbol{\phi}^T\mathbf{V}
    % % \operatorname{diag}(s_2+s_3,s_3+s_1,s_1+s_2)
    % \left[\begin{smallmatrix}
    %     s_2 + s_3 &  &  \\
    %     & s_1 + s_3 &  \\
    %     &  & s_1 + s_2
    %     \end{smallmatrix}\right]
    % \mathbf{V}^T\boldsymbol{\phi}
    % +O({\len {\boldsymbol{\phi}}}^3)}}d\boldsymbol{\phi} \\
    &= \frac{1}{8\pi^2}\frac{\exp\left(-\sqrt{2\boldsymbol{\phi}^T\boldsymbol{\Sigma} ^{-1}\boldsymbol{\phi}}\right)}{\sqrt{2\boldsymbol{\phi}^T\boldsymbol{\Sigma} ^{-1}\boldsymbol{\phi}}}\left(1+ O({\len {\boldsymbol{\phi}}}^2)\right) \mathrm{d}\boldsymbol{\phi} \\
\end{aligned}
\end{equation}
When 
% $\mathbf{R}\rightarrow \mathbf{R}_0$
\ree{$\|\mathbf{R} - \mathbf{R}_0\| \rightarrow 0$}
, we have 
% $\mathbf{\widetilde{R}} \rightarrow \mathbf{I}$ 
\ree{$\|\mathbf{\widetilde{R}} - \mathbf{I}\|  \rightarrow 0$ }
and $\boldsymbol{\phi} \rightarrow \mathbf{0}$, so Eq. \ref{eq:laplace} follows the multivariate Laplace distribution 
with the covariance matrix as $\boldsymbol{\Sigma}$, where $\boldsymbol{\Sigma} = 4 \mathbf{V}\operatorname{diag}(\frac{1}{s_2+s_3},\frac{1}{s_1+s_3},\frac{1}{s_1+s_2})\mathbf{V}^T$.
\end{proof}
