# Supplementary material for: Towards Robust Probabilistic Modeling on SO(3) via Rotation Laplace Distribution
Source: arXiv:2305.10465 source file (2025-02-21)
Supplement: Supplementary file 8 [file proof_quat.tex]

\begin{prop3}
    Denote $\mathbf{q}_0$ as the mode of qauternion Laplace distribution. Let $\pi$ be the tangent space of $\mathbb{S}^3$  at $\mathbf{q}_0$, and $\pi(\mathbf{x}) \in \mathbb{R}^4$ be the projection of $\mathbf{x} \in \mathbb{R}^4$ on $\pi$.
    For quaternion $\mathbf{q} \in \mathbb{S}^3$ following \emph{Bingham distribution} / \emph{qauternion Laplace distribution}, when $\mathbf{q}\rightarrow\mathbf{q}_0$, $\pi(\mathbf{q})$ follows zero-mean \emph{multivariate Gaussian distribution} / zero-mean \emph{multivariate Laplace distribution}.
    % For quaternion $\mathbf{q} \in \mathbb{S}^3$ following qauternion Laplace distribution, when $\mathbf{q}\rightarrow\mathbf{q}_0$, $\pi(\mathbf{q})$ follows zero-mean multivariate Laplace distribution.
\end{prop3}
\begin{proof}
Denote $\mathbf{q_I}=(1,0,0,0)^T$ as the identity quaternion. 
Define $\mathbf{M}$ as an orthogonal matrix such that $\mathbf{M}^T\mathbf{q}_0=\mathbf{q_I}$.
Given $\pi(\mathbf{q}) = \mathbf{q}-(\mathbf{q}\cdot \mathbf{q}_0)\mathbf{q}_0$,
we have
\begin{equation}
\footnotesize
\begin{aligned}
    \mathbf{M}^T\pi(\mathbf{q}) &= \mathbf{M}^T\mathbf{q} - ((\mathbf{M}^T\mathbf{q})\cdot(\mathbf{M}^T\mathbf{q}_0))\mathbf{q_I} 
    = \mathbf{M}^T\mathbf{q} - w\mathbf{q_I},
\end{aligned}
\end{equation}
where $\mathbf{M}^T\mathbf{q}=(w,x,y,z)^T$.
Let $(\mathbf{e}_0,\mathbf{e}_1,\mathbf{e}_2,\mathbf{e}_3)$ be the column vectors of $\mathbf{I}_{4\times4}$,
we have 
\begin{equation}
\footnotesize
    (\mathbf{M}\mathbf{e}_i)\cdot \mathbf{q}_0 = \mathbf{e}_i\cdot \mathbf{q_I} = 0
\end{equation}
for $i=1,2,3$.
Therefore, $\mathbf{M}\mathbf{e}_i (i=1,2,3)$ form an orthogonal basis of $\pi$.

Given $\mathbf{M}^T\mathbf{q}=w\mathbf{e}_0+x\mathbf{e}_1+y\mathbf{e}_2+z\mathbf{e}_3,$ we have
\begin{equation}
\footnotesize
    \mathbf{q} = w(\mathbf{M}\mathbf{e}_0)+x(\mathbf{M}\mathbf{e}_1)+y(\mathbf{M}\mathbf{e}_2)+z(\mathbf{M}\mathbf{e}_3)
\end{equation}
Therefore, $\boldsymbol{\eta} = (x,y,z)$ is the coordinate of $\pi(\mathbf{q})$ in $\pi$ under the basis of $\mathbf{M}\mathbf{e}_i$.

The Jacobian of the transformation $\mathbf{q}\rightarrow\boldsymbol{\eta}$ is given by
\begin{equation}
\footnotesize
\begin{aligned}
    \mathbf{J} &= \frac{\partial \mathbf{q}}{\partial \boldsymbol{\eta}} 
    = \mathbf{M}\frac{\partial \left(\mathbf{M}^T\mathbf{q}\right)}{\partial \boldsymbol{\eta}} \\
    &= \mathbf{M}\left[\begin{array}{cccc}
        -{x}/{w} & 1 & 0 & 0 \\
        -{y}/{w} & 0 & 1 & 0 \\
        -{z}/{w} & 0 & 0 & 0
        \end{array}\right]
\end{aligned}
\end{equation}
Therefore, the scaling factor from $\boldsymbol{\eta}$ to $\mathbf{q}$ is given by 
\begin{equation}
\footnotesize
    \frac{\mathrm{d}\mathbf{q}}{\mathrm{d}\boldsymbol{\eta}} = \operatorname{det}(\mathbf{J}\mathbf{J}^T)
    = 1+\frac{x^2+y^2+z^2}{w^2}+O(\len \eta^4)
    = 1+O(\len \eta^2).
\end{equation}
Thus
\begin{equation}
\scriptsize
\begin{aligned}
    \mathbf{q}^T\mathbf{MZM}^T \mathbf{q} 
    &= \left[\begin{array}{cccc}
        w & x & y & z
        \end{array}\right]
        \left[\begin{array}{cccc}
         0 &  &  &  \\
         & z_1 &  &  \\
         &  & z_2 &  \\
         &  &  & z_3 \\
        \end{array}\right]
        \left[\begin{array}{c}
        w \\  x \\ y \\ z
        \end{array}\right]\\
    &= \left[\begin{array}{ccc}
         x & y & z
        \end{array}\right]
        \left[\begin{array}{ccc}
          z_1 &  &  \\
           & z_2 &  \\
           &  & z_3 \\
        \end{array}\right]
        \left[\begin{array}{c}
        x \\ y \\ z
        \end{array}\right]\\
        &= \boldsymbol{\eta} \mathbf{\widetilde{Z}}\boldsymbol{\eta}
\end{aligned}
\end{equation}
where we define $\mathbf{\widetilde{Z}} = \operatorname{diag}(z_1, z_2, z_3)$.

For Bingham distribution, we have
\begin{equation}
\footnotesize
\begin{aligned}
    p(\mathbf{q})\mathrm{d}\mathbf{q} &\propto
    \exp\left(\mathbf{q}^T\mathbf{M}\mathbf{Z}\mathbf{M}^T\mathbf{q}\right)\mathrm{d}\mathbf{q} \\
    &= \exp\left(\boldsymbol{\eta}^T\mathbf{\widetilde{Z}}\boldsymbol{\eta}\right)(1+O(\len {\boldsymbol \eta}^2))\mathrm{d}\boldsymbol{\eta}\\
    &= \exp\left(-\boldsymbol{\eta}^T\boldsymbol{\Sigma}^{-1}\boldsymbol{\eta}\right)(1+O(\len {\boldsymbol \eta}^2))\mathrm{d}\boldsymbol{\eta}
\end{aligned}
\end{equation}
which follows the multivariate Gaussian distribution with the covariance matrix as $\boldsymbol{\Sigma}$, where $\boldsymbol{\Sigma}=-\operatorname{diag}(\frac{1}{z_1},\frac{1}{z_2},\frac{1}{z_3})$

For qauternion Laplace distribution, we have
\begin{equation}
\footnotesize
\begin{aligned}
    p(\mathbf{q})\mathrm{d}\mathbf{q} &\propto \frac{\exp\left(-\sqrt{-{\mathbf{q}^T\mathbf{M}\mathbf{Z}\mathbf{M}^T\mathbf{q}}}\right)}{\sqrt{-{\mathbf{q}^T\mathbf{M}\mathbf{Z}\mathbf{M}^T\mathbf{q}}}}\mathrm{d}\mathbf{q} \\
    % =\exp(\tr{\mathbf{VSU^T}\mathbf{\hat{\mathbf{R}}\widetilde{R}}})\mathrm{d}\mathbf{\widetilde{R}}
    &= \frac{1}{\sqrt{2}}\frac{\exp\left(-\sqrt{-\boldsymbol{\eta}^T\mathbf{\widetilde{Z}}\boldsymbol{\eta}}\right)}{\sqrt{-\boldsymbol{\eta}^T\mathbf{\widetilde{Z}}\boldsymbol{\eta}}}(1+O(\len {\boldsymbol{\eta}}^2))\mathrm{d}\boldsymbol{\eta}\\
    &= \frac{1}{\sqrt{2}}\frac{\exp\left(-\sqrt{2\boldsymbol{\eta}^T\boldsymbol{\Sigma}^{-1}\boldsymbol{\eta}}\right)}{\sqrt{2\boldsymbol{\eta}^T\boldsymbol{\Sigma}^{-1}\boldsymbol{\eta}}}(1+O(\len {\boldsymbol{\eta}}^2))\mathrm{d}\boldsymbol{\eta}
\end{aligned}
\end{equation}
which follows the multivariate Laplace distribution 
with the covariance matrix as $\boldsymbol{\Sigma}$, where $\boldsymbol{\Sigma} = -2\operatorname{diag}(\frac{1}{z_1},\frac{1}{z_2},\frac{1}{z_3})$.
\end{proof}
