# Supplementary material for: Towards Robust Probabilistic Modeling on SO(3) via Rotation Laplace Distribution
Source: arXiv:2305.10465 source file (2025-02-21)
Supplement: Supplementary file 10 [file supp_tab_multimodal_modelnet.tex]

\begin{table*}[ht]
\centering
% \scriptsize
\fontsize{7.5}{10}\selectfont
\caption{Per-category results on multimodal probabilistic distributions with top-k metrics on ModelNet10-SO3 dataset.}
\resizebox{0.99\textwidth}{!}{
\begin{tabular}{c@{}ll@{\hskip 0.3in}c@{\hskip 16pt}cccccccccc}
\toprule
       &                                     & & {avg.}     & {bathtub}  & {bed}      & {chair}    & {desk}     & {dresser}  & {tv}       & {n. stand} & {sofa}     & {table}    & {toilet}   \\
\midrule
\multirow{12}{*}{Top-2} 
&\multirow{4}{*}{Acc@15\textdegree$\uparrow$}                   
       & Deng \textit{et al.}\cite{deng2022deep}            &  0.863 & 0.768 & 0.945 & 0.923 & 0.779 & 0.775 & 0.877 & 0.702 &\bgl 0.963 &\bgl 0.935 & 0.967   \\     
       && Mohlin \textit{et al.}\cite{mohlin2020probabilistic}            &    0.864 &\bgl 0.769 &\bgl 0.946 &\bgd 0.933 & 0.776 & 0.788 & 0.881 & 0.693 & 0.955 & 0.920 &\bgl 0.980  \\     
       && Murphy \textit{et al.}\cite{murphy2021implicit}          &\bgl  0.868 & 0.735 &\bgl 0.946 & 0.900 &\bgl 0.803 &\bgl 0.810 &\bgl 0.883 &\bgl 0.756 & 0.959 & 0.932 & 0.960\\     
       && rotation Laplace            &    \bgd 0.900 &\bgd 0.831 &\bgd 0.959 &\bgl 0.932 &\bgd 0.852 &\bgd 0.847 &\bgd 0.903 &\bgd 0.770 &\bgd 0.965 &\bgd 0.951 &\bgd 0.987\\     
\cmidrule{2-14}
& \multirow{4}{*}{Acc@30\textdegree$\uparrow$}                   
       & Deng \textit{et al.}\cite{deng2022deep}            &    0.897 & 0.818 & 0.958 & 0.961 & 0.839 & 0.820 & 0.918 & 0.742 &\bgd 0.975 &\bgl 0.955 & 0.980  \\     
       && Mohlin \textit{et al.}\cite{mohlin2020probabilistic}            &\bgl  0.903 &\bgl 0.829 &\bgl 0.961 &\bgd 0.964 &\bgl 0.842 &\bgl 0.839 &\bgl 0.935 & 0.758 &\bgl 0.971 & 0.946 &\bgd 0.990 \\     
       && Murphy \textit{et al.}\cite{murphy2021implicit}            &    0.888 & 0.770 & 0.953 & 0.946 & 0.825 & 0.812 & 0.918 &\bgl 0.762 & 0.968 & 0.945 & 0.982  \\     
       && rotation Laplace            &\bgd   0.918 &\bgd 0.859 &\bgd 0.966 &\bgl 0.959 &\bgd 0.881 &\bgd 0.863 &\bgd 0.946 &\bgd 0.786 &\bgl 0.971 &\bgd 0.961 &\bgl 0.988 \\     
\cmidrule{2-14}
&\multirow{4}{*}{\shortstack{Median \\ Error ($^\circ$)$\downarrow$}} 
       & Deng \textit{et al.}\cite{deng2022deep}            &\bgl      3.8 &\bgl 5.5 &\bgl 2.7 & 3.8 &\bgl 4.7 &\bgl 3.6 & 4.0 &\bgl 4.7 &\bgl 2.4 &\bgl 3.1 & 3.0  \\     
       && Mohlin \textit{et al.}\cite{mohlin2020probabilistic}            &\bgl  3.8 & 5.9 &\bgl 2.7 &\bgl 3.5 & 5.0 &\bgl 3.6 &\bgl 3.9 & 4.9 & 2.6 & 3.5 &\bgl 2.8 \\     
       && Murphy \textit{et al.}\cite{murphy2021implicit}            &     4.9 & 6.8 & 4.1 & 5.5 & 5.3 & 4.9 & 5.3 & 5.1 & 3.9 & 3.7 & 4.8  \\     
       && rotation Laplace            &\bgd   2.3 &\bgd 3.5 &\bgd 1.7 &\bgd 3.0 &\bgd 2.6 &\bgd 1.8 &\bgd 2.7 &\bgd 2.0 &\bgd 1.6 &\bgd 1.8 &\bgd 2.2\\     
\midrule
\multirow{12}{*}{Top-4} 
&\multirow{4}{*}{Acc@15\textdegree$\uparrow$}                   
       & Deng \textit{et al.}\cite{deng2022deep}            &     0.875 & 0.804 & 0.951 & 0.928 & 0.776 & 0.781 & 0.881 & 0.743 & 0.961 & 0.952 & 0.969  \\     
       && Mohlin \textit{et al.}\cite{mohlin2020probabilistic}            &   0.882 & 0.799 & 0.956 &\bgd 0.942 & 0.801 & 0.813 &\bgl 0.899 & 0.730 & 0.957 & 0.938 &\bgl 0.984   \\     
       && Murphy \textit{et al.}\cite{murphy2021implicit}            &\bgl   0.904 &\bgl 0.806 &\bgd 0.966 & 0.905 &\bgl 0.862 &\bgl 0.870 &\bgl 0.899 &\bgd 0.842 &\bgl 0.966 &\bgl 0.956 & 0.963   \\     
       && rotation Laplace            &\bgd  0.919 &\bgd 0.862 &\bgd 0.966 &\bgl 0.941 &\bgd 0.871 &\bgd 0.876 &\bgd 0.914 &\bgl 0.830 &\bgd\bgd 0.970 &\bgd\bgd 0.974 &\bgd\bgd 0.987\\     
\cmidrule{2-14}
& \multirow{4}{*}{Acc@30\textdegree$\uparrow$}                   
       & Deng \textit{et al.}\cite{deng2022deep}            &    0.915 &\bgl 0.881 & 0.966 & 0.964 & 0.842 & 0.833 & 0.920 & 0.809 &\bgd 0.976 &\bgl 0.975 & 0.983  \\     
       && Mohlin \textit{et al.}\cite{mohlin2020probabilistic}            &\bgl  0.926 & 0.868 &\bgl 0.974 &\bgd 0.970 & 0.876 &\bgl 0.874 &\bgl 0.948 & 0.811 & 0.974 & 0.970 &\bgd 0.992  \\     
       && Murphy \textit{et al.}\cite{murphy2021implicit}            &\bgl   0.926 & 0.846 & 0.973 & 0.953 &\bgl 0.889 &\bgl 0.874 & 0.939 &\bgl 0.851 & 0.975 & 0.972 & \bgl 0.988  \\     
       && rotation Laplace            &\bgd    0.940 &\bgd 0.892 &\bgd 0.975 &\bgl 0.965 &\bgd 0.902 &\bgd 0.899 &\bgd 0.956 &\bgd 0.862 &\bgd 0.976 &\bgd 0.986 &\bgl 0.988\\     
\cmidrule{2-14}
&\multirow{4}{*}{\shortstack{Median \\ Error ($^\circ$)$\downarrow$}} 
       & Deng \textit{et al.}\cite{deng2022deep}            &\bgl   3.7 &\bgl 5.4 &\bgl 2.7 & 3.8 &\bgl 4.8 & 3.7 & 4.0 &\bgl 4.5 &\bgl 2.4 &\bgl 3.1 & 3.0    \\     
       && Mohlin \textit{et al.}\cite{mohlin2020probabilistic}            &\bgl    3.7 & 5.8 &\bgl 2.7 &\bgl 3.4 &\bgl 4.8 &\bgl 3.6 &\bgl 3.7 & 4.6 & 2.5 & 3.5 &\bgl 2.7  \\     
       && Murphy \textit{et al.}\cite{murphy2021implicit}            &     4.8 & 6.0 & 4.1 & 5.4 & 5.1 & 4.7 & 5.2 & 4.8 & 3.9 & 3.7 & 4.8  \\     
       && rotation Laplace            &\bgd     2.2 &\bgd 3.3 &\bgd 1.6 &\bgd 2.9 &\bgd 2.5 &\bgd 1.8 &\bgd 2.6 &\bgd 1.9 &\bgd 1.6 &\bgd 1.7 &\bgd 2.1\\   
\bottomrule
\end{tabular}
}
\label{tab:supp_multimodal}
\end{table*}
