# Supplementary material for: Towards Robust Probabilistic Modeling on SO(3) via Rotation Laplace Distribution
Source: arXiv:2305.10465 source file (2025-02-21)
Supplement: Supplementary file 11 [file additional_visual_modelnet.tex]

\begin{figure*}[t]
    \centering
    % \vspace{-6mm}
    % \hspace{-3mm}
    \begin{tabular}{cccccc}
    \includegraphics[height=1.6cm]{figures/more_vis/150.jpg}
    &\includegraphics[clip,trim=4.5cm 4cm 4.5cm 1.5cm, height=1.6cm]{figures/more_vis/150_rendering.jpg}
    &\includegraphics[height=1.2cm]{figures/more_vis/150_ipdf.jpg}
    \hspace{4mm}
    &\includegraphics[height=1.6cm]{figures/more_vis/330.jpg}
    &\includegraphics[clip,trim=4.5cm 4cm 4.5cm 1.5cm, height=1.6cm]{figures/more_vis/330_rendering.jpg}
    &\includegraphics[height=1.2cm]{figures/more_vis/330_ipdf.jpg}\\
    
    \includegraphics[height=1.6cm]{figures/more_vis/m450.jpg}
    &\includegraphics[clip,trim=4.5cm 4cm 4.5cm 1.5cm, height=1.6cm]{figures/more_vis/m450_rendering.jpg}
    &\includegraphics[height=1.2cm]{figures/more_vis/m450_ipdf.jpg}
    \hspace{4mm}
    &\includegraphics[height=1.6cm]{figures/more_vis/277.jpg}
    &\includegraphics[clip,trim=4.5cm 4cm 4.5cm 1.5cm, height=1.6cm]{figures/more_vis/277_rendering.jpg}
    &\includegraphics[height=1.2cm]{figures/more_vis/277_ipdf.jpg}\\
    
    \includegraphics[height=1.6cm]{figures/more_vis/1815.jpg}
    &\includegraphics[clip,trim=4.5cm 4cm 4.5cm 1.5cm, height=1.6cm]{figures/more_vis/1815_rendering.jpg}
    &\includegraphics[height=1.2cm]{figures/more_vis/1815_ipdf.jpg}
    \hspace{4mm}
    &\includegraphics[height=1.6cm]{figures/more_vis/1170.jpg}
    &\includegraphics[clip,trim=4.5cm 4cm 4.5cm 1.5cm, height=1.6cm]{figures/more_vis/1170_rendering.jpg}
    &\includegraphics[height=1.2cm]{figures/more_vis/1170_ipdf.jpg}\\
    
    \includegraphics[height=1.6cm]{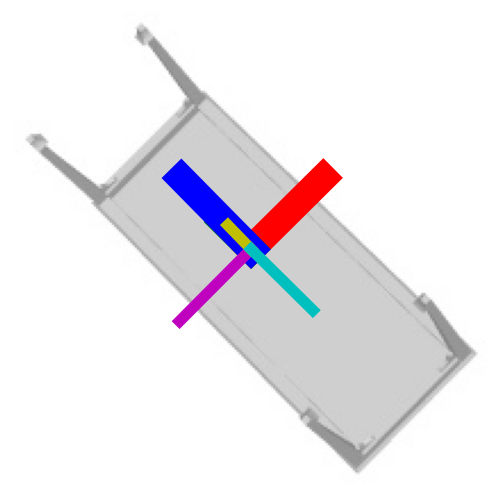}
    &\includegraphics[clip,trim=4.5cm 4cm 4.5cm 1.5cm, height=1.6cm]{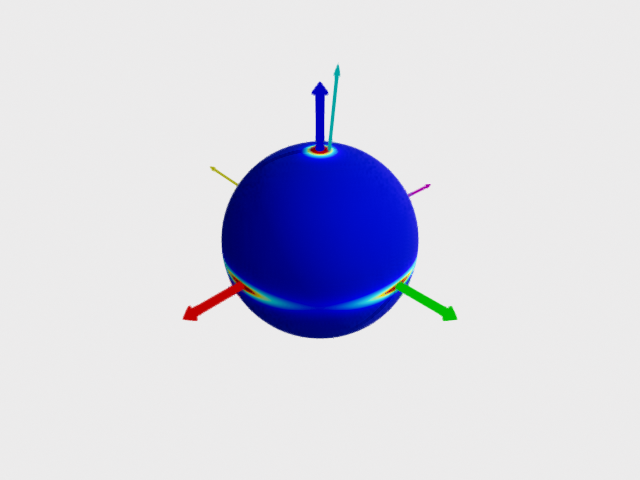}
    &\includegraphics[height=1.2cm]{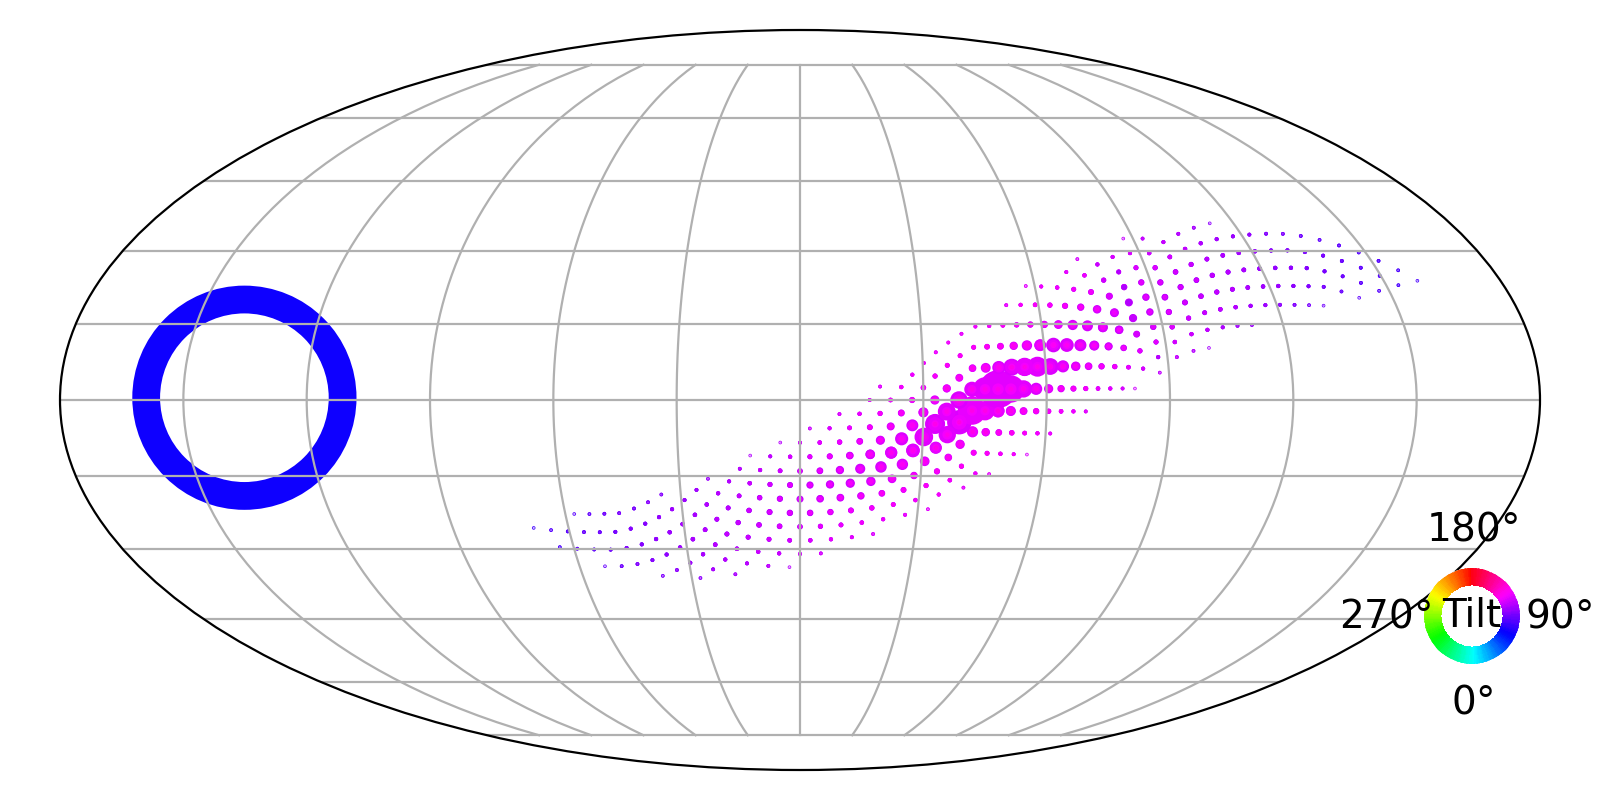}
    \hspace{4mm}
    &\includegraphics[height=1.6cm]{figures/more_vis/93.jpg}
    &\includegraphics[clip,trim=4.5cm 4cm 4.5cm 1.5cm, height=1.6cm]{figures/more_vis/93_rendering.jpg}
    &\includegraphics[height=1.2cm]{figures/more_vis/93_ipdf.jpg}\\
    
    \includegraphics[height=1.6cm]{figures/more_vis/21.jpg}
    &\includegraphics[clip,trim=4.5cm 4cm 4.5cm 1.5cm, height=1.6cm]{figures/more_vis/21_rendering.jpg}
    &\includegraphics[height=1.2cm]{figures/more_vis/21_ipdf.jpg}
    \hspace{4mm}
    &\includegraphics[height=1.6cm]{figures/more_vis/1290.jpg}
    &\includegraphics[clip,trim=4.5cm 4cm 4.5cm 1.5cm, height=1.6cm]{figures/more_vis/1290_rendering.jpg}
    &\includegraphics[height=1.2cm]{figures/more_vis/1290_ipdf.jpg}\\
    
    \includegraphics[height=1.6cm]{figures/more_vis/1255.jpg}
    &\includegraphics[clip,trim=4.5cm 4cm 4.5cm 1.5cm, height=1.6cm]{figures/more_vis/1255_rendering.jpg}
    &\includegraphics[height=1.2cm]{figures/more_vis/1255_ipdf.jpg}
    \hspace{4mm}
    &\includegraphics[height=1.6cm]{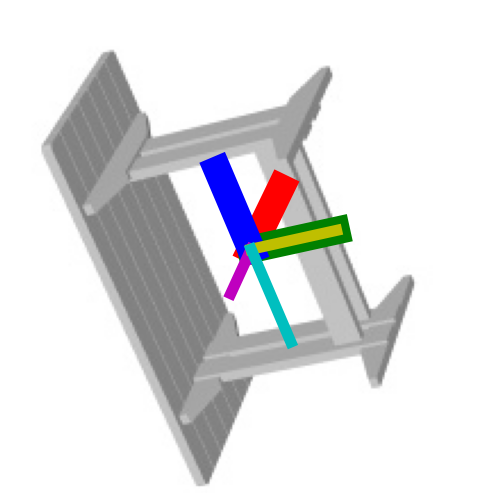}
    &\includegraphics[clip,trim=4.5cm 4cm 4.5cm 1.5cm, height=1.6cm]{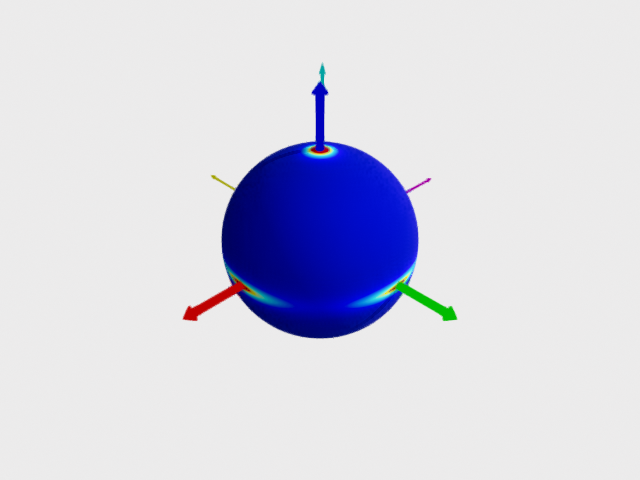}
    &\includegraphics[height=1.2cm]{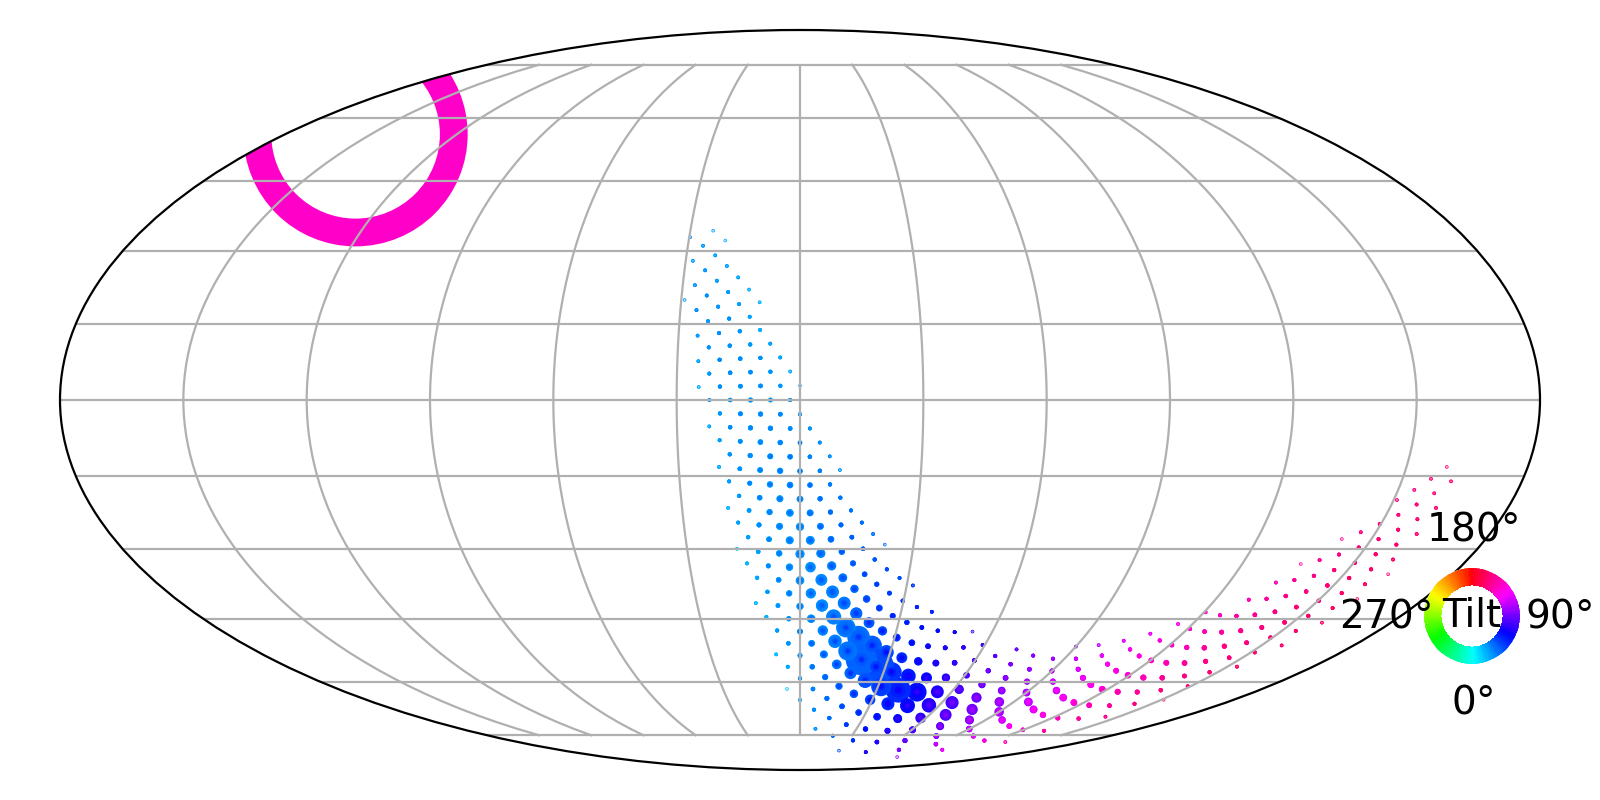}\\
    
    \small{Input image} & {\tiny\makecell{Distribution visual.\\\cite{mohlin2020probabilistic}}} & {\tiny\makecell{Distribution visual.\\\cite{murphy2021implicit}}}  \hspace{4mm} &
    \small{Input image} & {\tiny\makecell{Distribution visual.\\\cite{mohlin2020probabilistic}}} & {\tiny\makecell{Distribution visual.\\\cite{murphy2021implicit}}}
    \end{tabular}
    % \vspace{1mm}
    \caption{\small \ree{Visual results on ModelNet10-SO3 dataset. We adopt the distribution visualization methods in \cite{mohlin2020probabilistic} and \cite{murphy2021implicit}. For input images and visualizations with \cite{mohlin2020probabilistic}, predicted rotations are shown with thick lines and the ground truths are with thin lines. For visualizations with \cite{murphy2021implicit}, ground truths are shown by solid circles.}}
    \vspace{-2mm}
	\label{fig:vis_modelnet}
\end{figure*}
