# Supplementary material for: Towards Robust Probabilistic Modeling on SO(3) via Rotation Laplace Distribution
Source: arXiv:2305.10465 source file (2025-02-21)
Supplement: Supplementary file 12 [file additional_visual_pascal.tex]

\begin{figure*}[t]
    \centering
    % \vspace{-6mm}
    % \hspace{-3mm}
    \begin{tabular}{cccccc}
    \includegraphics[height=1.6cm]{figures/more_vis/30.jpg}
    &\includegraphics[clip,trim=4.5cm 4cm 4.5cm 1.5cm, height=1.6cm]{figures/more_vis/30_rendering.jpg}
    &\includegraphics[height=1.2cm]{figures/more_vis/30_ipdf.jpg}
    \hspace{4mm}
    &\includegraphics[height=1.6cm]{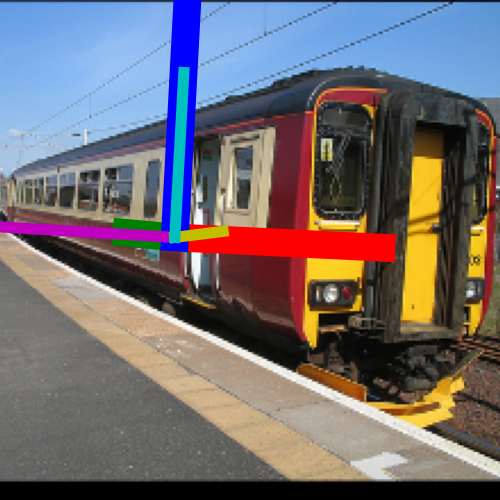}
    &\includegraphics[clip,trim=4.5cm 4cm 4.5cm 1.5cm, height=1.6cm]{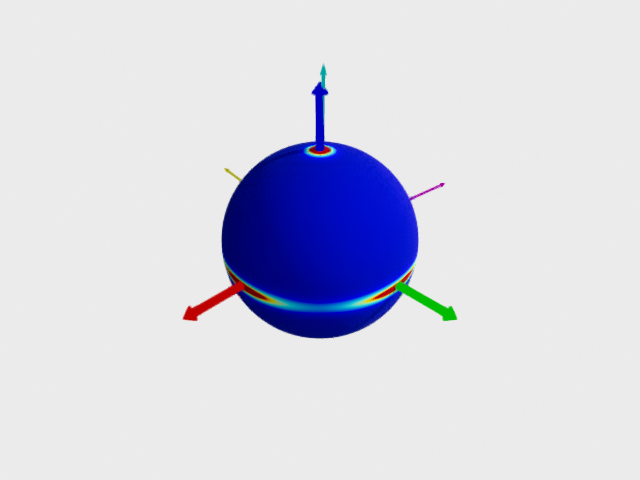}
    &\includegraphics[height=1.2cm]{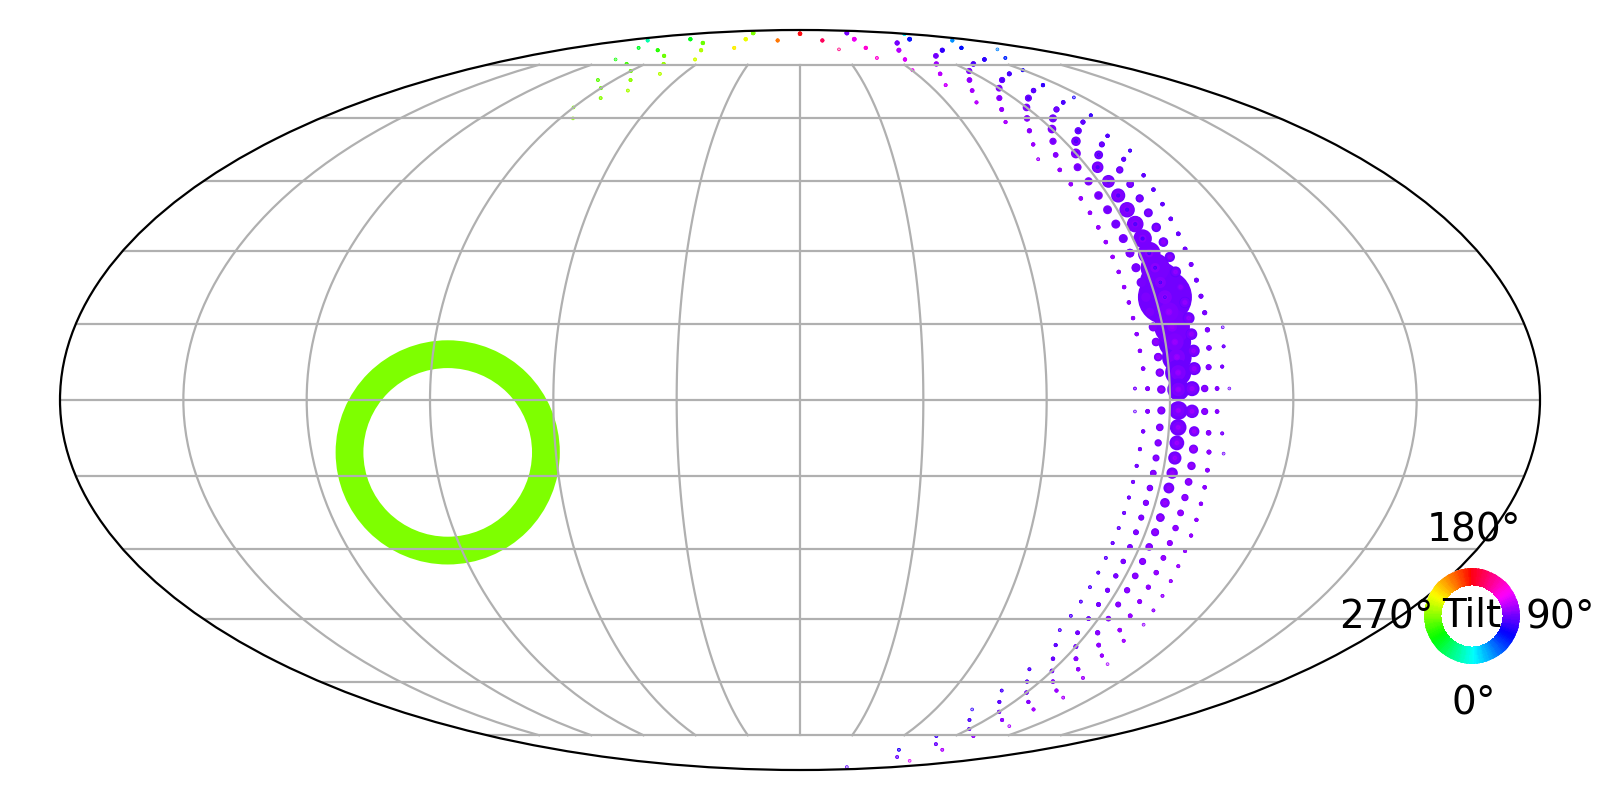}\\
    
    \includegraphics[height=1.6cm]{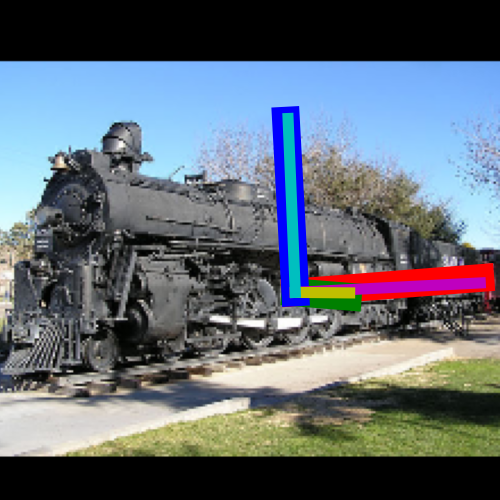}
    &\includegraphics[clip,trim=4.5cm 4cm 4.5cm 1.5cm, height=1.6cm]{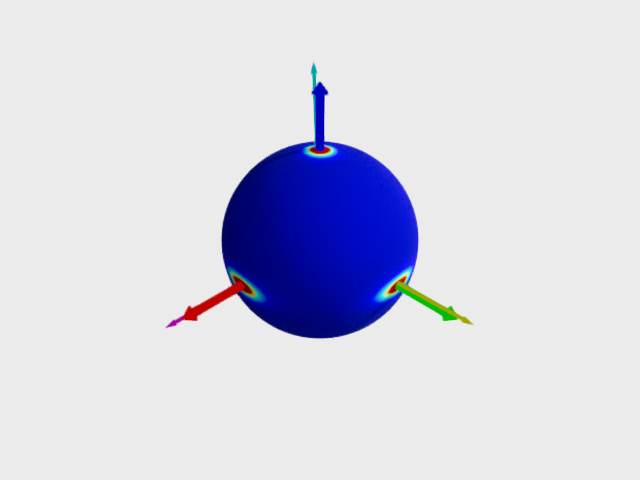}
    &\includegraphics[height=1.2cm]{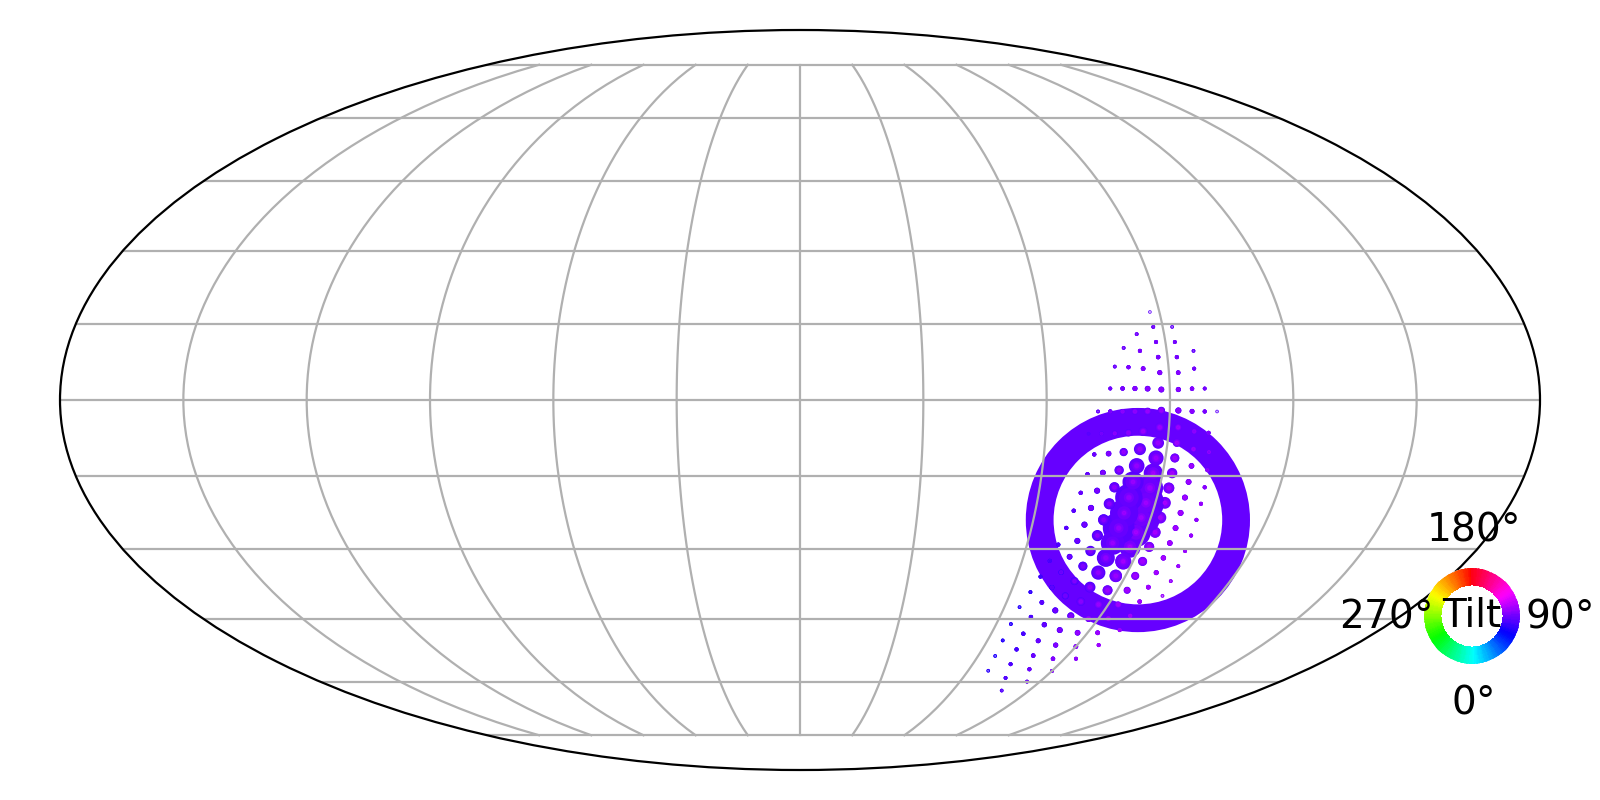}
    \hspace{4mm}
    &\includegraphics[height=1.6cm]{figures/more_vis/450.jpg}
    &\includegraphics[clip,trim=4.5cm 4cm 4.5cm 1.5cm, height=1.6cm]{figures/more_vis/450_rendering.jpg}
    &\includegraphics[height=1.2cm]{figures/more_vis/450_ipdf.jpg}\\
    
    \includegraphics[height=1.6cm]{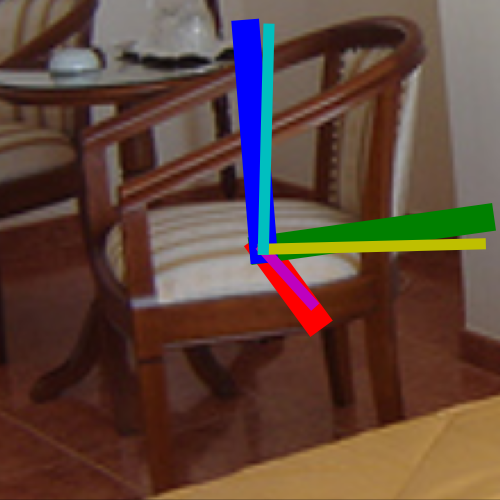}
    &\includegraphics[clip,trim=4.5cm 4cm 4.5cm 1.5cm, height=1.6cm]{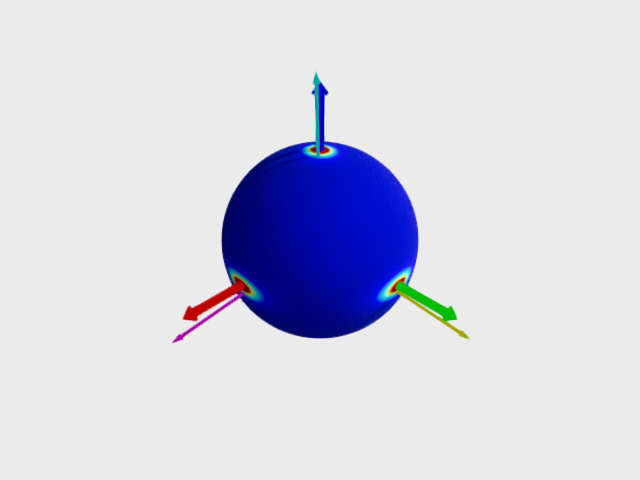}
    &\includegraphics[height=1.2cm]{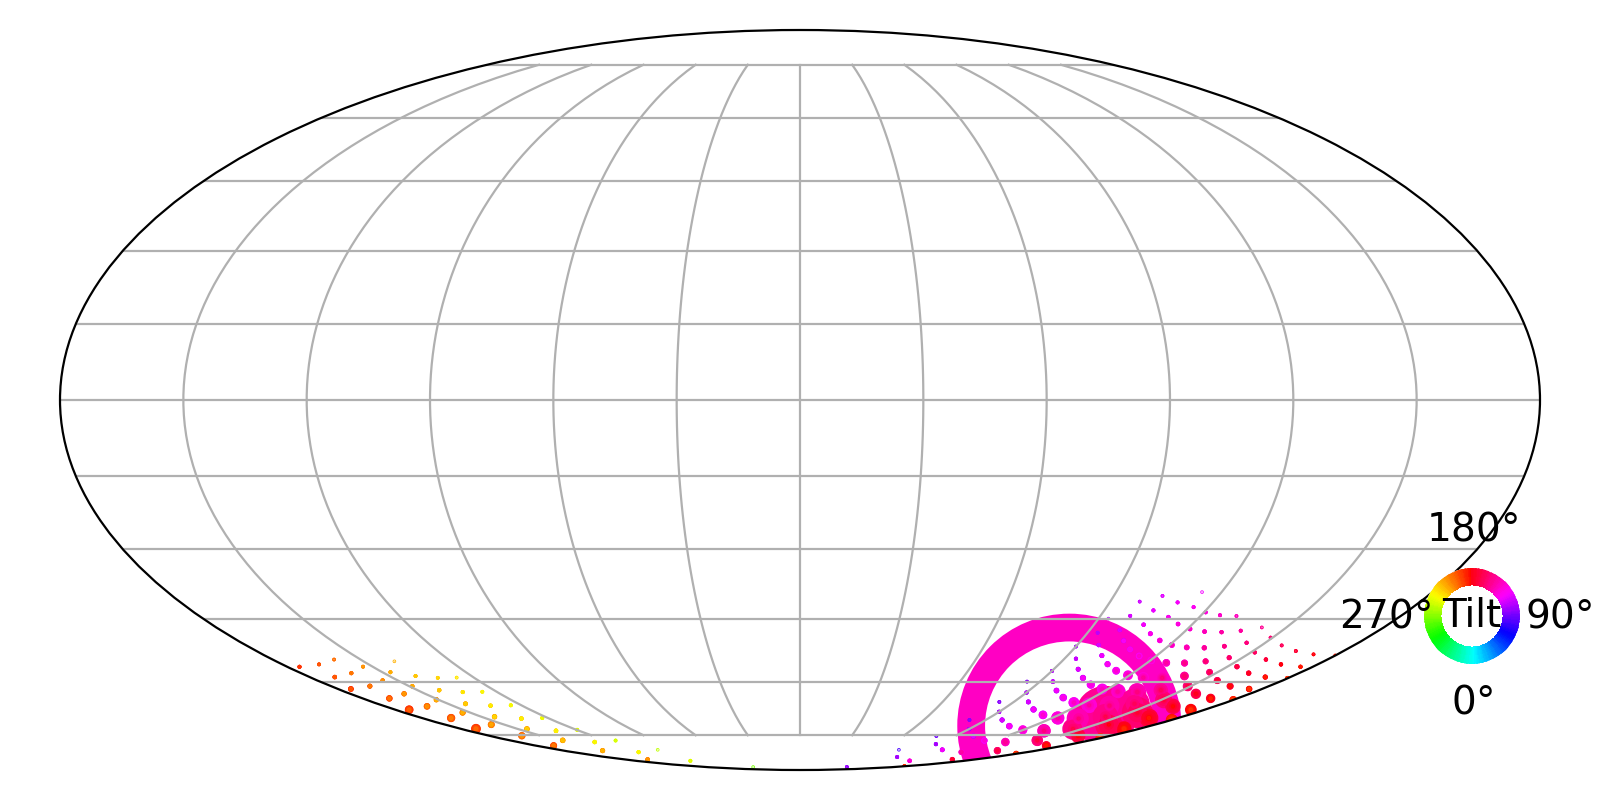}
    \hspace{4mm}
    &\includegraphics[height=1.6cm]{figures/more_vis/540.jpg}
    &\includegraphics[clip,trim=4.5cm 4cm 4.5cm 1.5cm, height=1.6cm]{figures/more_vis/540_rendering.jpg}
    &\includegraphics[height=1.2cm]{figures/more_vis/540_ipdf.jpg}\\
    
    \includegraphics[height=1.6cm]{figures/more_vis/900.jpg}
    &\includegraphics[clip,trim=4.5cm 4cm 4.5cm 1.5cm, height=1.6cm]{figures/more_vis/900_rendering.jpg}
    &\includegraphics[height=1.2cm]{figures/more_vis/900_ipdf.jpg}
    \hspace{4mm}
    &\includegraphics[height=1.6cm]{figures/more_vis/840.jpg}
    &\includegraphics[clip,trim=4.5cm 4cm 4.5cm 1.5cm, height=1.6cm]{figures/more_vis/840_rendering.jpg}
    &\includegraphics[height=1.2cm]{figures/more_vis/840_ipdf.jpg}\\
    
    \includegraphics[height=1.6cm]{figures/more_vis/1070.jpg}
    &\includegraphics[clip,trim=4.5cm 4cm 4.5cm 1.5cm, height=1.6cm]{figures/more_vis/1070_rendering.jpg}
    &\includegraphics[height=1.2cm]{figures/more_vis/1070_ipdf.jpg}
    \hspace{4mm}
    &\includegraphics[height=1.6cm]{figures/more_vis/1380.jpg}
    &\includegraphics[clip,trim=4.5cm 4cm 4.5cm 1.5cm, height=1.6cm]{figures/more_vis/1380_rendering.jpg}
    &\includegraphics[height=1.2cm]{figures/more_vis/1380_ipdf.jpg}\\
    
    \includegraphics[height=1.6cm]{figures/more_vis/1696.jpg}
    &\includegraphics[clip,trim=4.5cm 4cm 4.5cm 1.5cm, height=1.6cm]{figures/more_vis/1696_rendering.jpg}
    &\includegraphics[height=1.2cm]{figures/more_vis/1696_ipdf.jpg}
    \hspace{4mm}
    &\includegraphics[height=1.6cm]{figures/more_vis/1230.jpg}
    &\includegraphics[clip,trim=4.5cm 4cm 4.5cm 1.5cm, height=1.6cm]{figures/more_vis/1230_rendering.jpg}
    &\includegraphics[height=1.2cm]{figures/more_vis/1230_ipdf.jpg}\\
    
    \small{Input image} & {\tiny\makecell{Distribution visual.\\\cite{mohlin2020probabilistic}}} & {\tiny\makecell{Distribution visual.\\\cite{murphy2021implicit}}}  \hspace{4mm} &
    \small{Input image} & {\tiny\makecell{Distribution visual.\\\cite{mohlin2020probabilistic}}} & {\tiny\makecell{Distribution visual.\\\cite{murphy2021implicit}}}
    \end{tabular}
    % \vspace{-3mm}
    \caption{\small \ree{Visual results on Pascal3D+ dataset. We adopt the distribution visualization methods in \cite{mohlin2020probabilistic} and \cite{murphy2021implicit}. For input images and visualizations with \cite{mohlin2020probabilistic}, predicted rotations are shown with thick lines and the ground truths are with thin lines. For visualizations with \cite{murphy2021implicit}, ground truths are shown by solid circles.}}
    \vspace{-2mm}
	\label{fig:vis_pascal}
\end{figure*}
