# Supplementary material for: Towards Robust Probabilistic Modeling on SO(3) via Rotation Laplace Distribution
Source: arXiv:2305.10465 source file (2025-02-21)
Supplement: Supplementary file 13 [file elaboration.tex]

\textbf{Elaboration of Eq. \ref{eq:prdr} in the main paper}

Given $\mathbf{R}_0 = \mathbf{UV}^T$ and $\mathbf{\widetilde{R}}=\mathbf{R}_0^T\mathbf{R}$,
\begin{equation}
\scriptsize
\begin{aligned}
 p(\mathbf{R})\mathrm{d}\mathbf{R} &\propto 
 \frac{\exp\left(\sqrt{\operatorname{tr}(\mathbf{S}-{\mathbf{A}^T\mathbf{R}})}\right)}{\sqrt{\operatorname{tr}(\mathbf{S}-{\mathbf{A}^T\mathbf{R}})}} \mathrm{d}\mathbf{R} 
 = \frac{\exp\left(\sqrt{\operatorname{tr}(\mathbf{S}-\mathbf{V}\mathbf{S}\mathbf{U}^T\mathbf{R})}\right)}{\sqrt{\operatorname{tr}(\mathbf{S}-\mathbf{V}\mathbf{S}\mathbf{U}^T\mathbf{R})}} \mathrm{d}\mathbf{R} \\
 &= \frac{\exp\left(\sqrt{\operatorname{tr}(\mathbf{S}-\mathbf{S}\mathbf{U}^T\mathbf{R}\mathbf{V})}\right)}{\sqrt{\operatorname{tr}(\mathbf{S}-\mathbf{S}\mathbf{U}^T\mathbf{R}\mathbf{V})}} \mathrm{d}\mathbf{R} \\
 &= \frac{\exp\left(\sqrt{\operatorname{tr}(\mathbf{S}-\mathbf{S}\mathbf{U}^T\mathbf{R}_0\mathbf{\widetilde{R}}\mathbf{V})}\right)}{\sqrt{\operatorname{tr}(\mathbf{S}-\mathbf{S}\mathbf{U}^T\mathbf{R}_0\mathbf{\widetilde{R}}\mathbf{V})}} \mathrm{d}\mathbf{R} \\
 &= \frac{\exp\left(\sqrt{\operatorname{tr}(\mathbf{S}-\mathbf{S}\mathbf{V}^T\mathbf{\widetilde{R}}\mathbf{V})}\right)}{\sqrt{\operatorname{tr}(\mathbf{S}-\mathbf{S}\mathbf{V}^T\mathbf{\widetilde{R}}\mathbf{V})}} \mathrm{d}\mathbf{R}
\end{aligned}
\end{equation}
