# Supplementary material for: Towards Robust Probabilistic Modeling on SO(3) via Rotation Laplace Distribution
Source: arXiv:2305.10465 source file (2025-02-21)
Supplement: Supplementary file 14 [file impl_details.tex]

\section{More Implementation Details}
\label{sec:more_detail}
In the experiment of section 5, 6, 7.1, 8, we follow the implementation designs of \cite{mohlin2020probabilistic} and merely change the distribution from matrix Fisher distribution to our rotation Laplace distribution.
We use pretrained ResNet-101 as our backbone, and encode the object class information (for single-model-all-category experiments) by an embedding layer that produces a 32-dim vector. We apply a 512-512-9 MLP as the output layer. 
The batch size is set as 32.
We use the SGD optimizer and start with the learning rate of 0.01.
For ModelNet10-SO3 dataset, we train 50 epochs with learning rate decaying by a factor of 10 at epochs 30, 40, and 45. For Pascal3D+ dataset, we train 120 epochs with the same learning rate decay at epochs 30, 60 and 90.

\jiangran{
For the experiment of semi-supervised learning in Section 7.2, we follow the implementation designs of \cite{yin2022fishermatch} and change the distribution from matrix Fisher distribution to our rotation Laplace distribution. The unsupervised loss weight $\lambda_u$ is set to 1. In the pre-training stage, we train with the
batch size of 32, and for the SSL stage, a training batch is
composed of 32 labeled samples and 128 unlabeled samples.
Both the weak and strong augmentations consist of
random padding, cropping, and resizing operations with different strengths. 
We use MobileNet-V2 as our backbone and the Adam optimizer
with the learning rate as 1e-4 in pre-training stage and 1e-3 in the semi-supervised training stage. The entropy
threshold $\tau$ is set as around -6.3.
}

% \ree{We build a lookup table w.r.t. the proper singular values for computing the normalization factors. For computing  each element in the table, we discretize $\SO$ into about 300k equivolumetric grids. We sample about 5.6M different sets of proper singular values, the storage for which is about 21MB for forward and 63MB for backward.}
