# Supplementary material for: Towards Robust Probabilistic Modeling on SO(3) via Rotation Laplace Distribution
Source: arXiv:2305.10465 source file (2025-02-21)
Supplement: Supplementary file 19 [file supp_tab_modelnet.tex]

\begin{table*}[ht]
\centering
% \scriptsize
\fontsize{7.5}{10}\selectfont
\caption{Per-category results ModelNet10-SO3 dataset.}
\resizebox{0.99\textwidth}{!}{
\begin{tabular}{@{}ll@{\hskip 0.3in}c@{\hskip 16pt}cccccccccc}
\toprule
       &                                      & {avg.}     & {bathtub}  & {bed}      & {chair}    & {desk}     & {dresser}  & {tv}       & {n. stand} & {sofa}     & {table}    & {toilet}   \\
\midrule
\multirow{4}{*}{Acc@15\textdegree$\uparrow$}                   & Deng \textit{et al.}\cite{deng2022deep}            & 0.562      & 0.140      & 0.788      & 0.800      & 0.345      & 0.563      & 0.708      & 0.279      & 0.733      & 0.440      & 0.832      \\      
       & Prokudin \textit{et al.}\cite{prokudin2018deep}        & 0.456      & 0.114      & 0.822      & 0.662      & 0.023      & 0.406      & 0.704      & 0.187      & 0.590      & 0.108      &  0.946 \\
       & Mohlin \textit{et al.}\cite{mohlin2020probabilistic} &  0.693 &  0.322 & \bgl 0.882 & \bgl 0.881 &  0.536 &  0.682 &  0.790 &  0.516 & \bgl 0.919 &  0.446 & \bgl 0.957 \\      
       & Murphy \textit{et al.}\cite{murphy2021implicit}     & \bgl 0.719 & \bgd 0.392 &  0.877 &  0.874 & \bgl 0.615 & \bgl 0.687 & \bgl 0.799 & \bgl 0.567 &  0.914 & \bgd 0.523 & 0.945      \\
       & rotation Laplace               & \bgd 0.741  & \bgl 0.390  & \bgd 0.902  & \bgd 0.909  & \bgd 0.644  & \bgd 0.722  & \bgd 0.815  & \bgd 0.590  & \bgd 0.934  & \bgl 0.521  & \bgd 0.977  \\
\midrule
\multirow{4}{*}{Acc@30\textdegree$\uparrow$}                   & Deng \textit{et al.}\cite{deng2022deep}           & 0.694      & 0.325      & 0.880      & 0.908      & 0.556      & 0.649      & 0.807      & 0.466      & 0.902      & 0.485      & 0.958      \\      
       & Prokudin \textit{et al.}\cite{prokudin2018deep}        & 0.528      & 0.175      & 0.847      & 0.777      & 0.061      & 0.500      & 0.788      & 0.306      & 0.673      & 0.183      & 0.972 \\
       & Mohlin \textit{et al.}\cite{mohlin2020probabilistic} & \bgl 0.757 &  0.403 & \bgl 0.908 & \bgl 0.935 & \bgl 0.674 & \bgl 0.739 & \bgl 0.863 & \bgl 0.614 & \bgl 0.944 & 0.511 & \bgl 0.981 \\      
       & Murphy \textit{et al.}\cite{murphy2021implicit}     & 0.735 & \bgl 0.410 &  0.883 &  0.917 & 0.629 & 0.688 &  0.832 &  0.570 &  0.921 & \bgl 0.531 & 0.967      \\
       & rotation Laplace               & \bgd  0.770  & \bgd 0.430 & \bgd 0.911  & \bgd 0.940 & \bgd 0.698  & \bgd 0.751  & \bgd 0.869 & \bgd 0.625  & \bgd 0.946  & \bgd 0.541  & \bgd 0.986  \\
\midrule
\multirow{4}{*}{\shortstack{Median \\ Error ($^\circ$)$\downarrow$}} & Deng \textit{et al.}\cite{deng2022deep}           & 32.6       & 147.8      & 9.2        & 8.3        & 25.0       & 11.9       & 9.8        & 36.9       & 10.0       & 58.6       & 8.5        \\
       & Prokudin \textit{et al.}\cite{prokudin2018deep}        & 49.3       &  122.8 & \bgl 3.6   & 9.6        & 117.2      & 29.9       & 6.7        & 73.0       & 10.4       & 115.5      &  4.1   \\
       & Mohlin \textit{et al.}\cite{mohlin2020probabilistic} & \bgl 17.1  & \bgl 89.1  &  4.4   & \bgl 5.2   &  13.0  &  6.3   &  5.8   &  13.5  & \bgl 4.0   &  25.8  & \bgl 4.0   \\      
       & Murphy \textit{et al.}\cite{murphy2021implicit}     &  21.5  & 161.0      &  4.4   &  5.5   & \bgl 7.1   & \bgl 5.5   & \bgl 5.7   & \bgl 7.5   &  4.1   & \bgd 9.0   & 4.8        \\
       & rotation Laplace               & \bgd 12.2  & \bgd 85.1  & \bgd 2.3  & \bgd 3.4 & \bgd 5.4 & \bgd 2.7  & \bgd 3.7 & \bgd 4.8  & \bgd 2.1  & \bgl 9.6  & \bgd 2.5  \\
\bottomrule
\end{tabular}
}
\label{tab:supp_modelnet}
\end{table*}
