# Supplementary material for: Towards Robust Probabilistic Modeling on SO(3) via Rotation Laplace Distribution
Source: arXiv:2305.10465 source file (2025-02-21)
Supplement: Supplementary file 20 [file supp_tab_pascal.tex]

\begin{table*}[ht]
\caption{Per-category results on Pascal3D+ dataset.}
  \centering
  \fontsize{7.5}{10}\selectfont
%   \scriptsize
  \resizebox{0.99\textwidth}{!}{
    \begin{tabular}{@{}ll@{\hskip 0.3in}c@{\hskip 16pt}cccccccccccc}
      &                                      & {avg.}     & {aero}  & {bike}      & {boat}    & {bottle}     & {bus}  & {car}       & {chair} & {table}     & {mbike}    & {sofa} & {train}  & {tv} \\
    \midrule
    \multirow{6}{*}{Acc@30\textdegree  $\uparrow$} 
        & Tulsiani \& Malik \cite{tulsiani2015viewpoints}         & 0.808 & 0.81  & 0.77  &  0.59 & 0.93 &  \bgd {0.98} & 0.89 & 0.80 & 0.62 & \bgl 0.88 & 0.82 & 0.80 & 0.80 \\
        & Mahendran \textit{et al.}\cite{mahendran2018mixed}             & \bgl 0.859 & 0.87 & 0.81 &  \bgd {0.64} &  \bgd {0.96} &  0.97 &  0.95 &  \bgd {0.92} & 0.67 & 0.85 & \bgd 0.97 & \bgl 0.82 & \bgl 0.88 \\
        & Liao \textit{et al.}\cite{liao2019spherical}              & 0.819 & 0.82 & 0.77 & 0.55 & 0.93 & 0.95 & 0.94 & 0.85 & 0.61 & 0.80 &  0.95 &  \bgd {0.83} & 0.82     \\   
        & Prokudin \textit{et al.}\cite{liao2019spherical}               &  0.838 &   0.89 &  0.83 & 0.46 &  \bgd {0.96} & 0.93 & 0.90 & 0.80 & \bgl 0.76 & \bgd 0.90 &  {0.90} & \bgl 0.82 &  \bgd {0.91} \\
        & Mohlin \textit{et al.}\cite{mohlin2020probabilistic}        & 0.825 &  \bgd {0.90} & \bgl 0.85 & 0.57 &  0.94 & 0.95 &  \bgd {0.96} & 0.78 & 0.62 & 0.87 & 0.85 & 0.77 & 0.84 \\
        & Murphy \textit{et al.}\cite{murphy2021implicit}             & 0.837 & 0.81 & \bgl 0.85 & 0.56 & 0.93 & 0.95 & 0.94 &  0.87 &  \bgd {0.78} & 0.85 & 0.88 & 0.78 & 0.86  \\
        & rot. Laplace (Ours)                   & \bgd {0.876} & \bgd {0.90}  & \bgd {0.90}  & \bgl 0.60 & \bgd {0.96} & \bgd {0.98} & \bgd {0.96} & \bgl 0.91  & \bgl 0.76  & \bgl 0.88 & \bgd 0.97 &  0.81 & \bgl 0.88  \\
       
    \midrule
    \multirow{6}{*}{\shortstack{Median\\error ($^\circ$)  $\downarrow$}}
        & Tulsiani \& Malik \cite{tulsiani2015viewpoints} & 13.6 & 13.8 & 17.7 & \bgl 21.3 & 12.9 & 5.8 & 9.1 & 14.8 & 15.2 & 14.7 & 13.7 & 8.7 & 15.4 \\
        & Mahendran \textit{et al.}\cite{mahendran2018mixed} &  10.1 &  \bgd {8.5} &  14.8 &  \bgd {20.5} &  7.0 &  3.1 &  5.1 & \bgl 9.3 &  11.3 & 14.2 & 10.2 & \bgl 5.6 & \bgl 11.7 \\
        & Liao \textit{et al.}\cite{liao2019spherical}            & 13.0 & 13.0 & 16.4 & 29.1 & 10.3 & 4.8 & 6.8 & 11.6 & 12.0 & 17.1 & 12.3 & 8.6 & 14.3       \\
        & Prokudin \textit{et al.}\cite{liao2019spherical} & 12.2 &  9.7 & 15.5 & 45.6 &  \bgd {5.4} & \bgl 2.9 &  \bgd {4.5} & 13.1 & 12.6 &  \bgd {11.8} & \bgl 9.1 &  \bgd {4.3} & 12.0 \\
        & Mohlin \textit{et al.}\cite{mohlin2020probabilistic} & 11.5 & 10.1 & 15.6 & 24.3 & 7.8 & 3.3 & 5.3 & 13.5 & 12.5 &  12.9 & 13.8 & 7.4 & \bgl 11.7\\
        & Murphy \textit{et al.}\cite{murphy2021implicit}                        &  10.3 & 10.8 & \bgl 12.9 & 23.4 & 8.8 & 3.4 & 5.3 &  10.0 &  \bgd {7.3} & 13.6 &  9.5  & 6.4  & 12.3 \\
        & rot. Laplace (Ours)             &  \bgd {9.4}  & \bgl 8.6 & \bgd {11.7} &  21.8 & \bgl 6.9 & \bgd {2.8} & \bgl 4.8 & \bgd {7.9} & \bgl 9.1 & \bgl 12.2 & \bgd {8.1} & 6.9 & \bgd {11.6}    \\
      
      \bottomrule
    \end{tabular}
  }
  \label{tab:supp_pascal}
  \end{table*}
